# Supplementary material for: Classical Benchmarks for Variational Quantum Eigensolver Simulations of the Hubbard Model
Source: arXiv:2408.00836 ancillary file (2025-05-13)
Supplement: Supplementary file 1 [file supplement.pdf]

# Supplementary Information to 'Classical Benchmarks for Variational Quantum Eigensolver Simulations of the Hubbard Model'

Antonios M. Alvertis[1,2], Abid Khan[3], Thomas Iadecola[4,5], Peter P. Orth[6], Norm Tubman[7]

[1]KBR, Inc., NASA Ames Research Center, Moffett Field, California 94035, United States

[2]Materials Sciences Division, Lawrence Berkeley National Laboratory, Berkeley, California 94720, United States

[3]Department of Physics, University of Illinois Urbana-Champaign, Urbana, IL, United States 61801

[4]Department of Physics and Astronomy, Iowa State University, Ames, IA 50011, USA

[5]Ames National Laboratory, Ames, IA 50011, USA

[6]Department of Physics, Saarland University, 66123 Saarbrücken, Germany

[7]NASA Ames Research Center, Moffett Field, CA 94035, United States

# Contents

**S1 NP ansatz,** $U/t = 2$ **2**

**S2 EP ansatz,** $U/t = 2$ **9**

**S3 NP ansatz,** $U/t = 8$ **16**

**S4 NP ansatz,** $U/t = 2$, $d = 0.2$ **23**

**S5 NP ansatz,** $U/t = 2$, $d = 0.8$ **25**

**S6 NP ansatz,** $U/t = 2$, $V = 0.2$ **26**

**S7 NP ansatz,** $U/t = 2$, $V = 0.8$ **28**

**S8 NP ansatz,** $U/t = 2$**, overlap-based optimization** **29**

**S9 NP ansatz,** $U/t = 8$**, overlap-based optimization** **36**

**S10NP ansatz,** $U/t = 2$, $4 \times 4$ **lattice** **43**

Below we give the tables of VQE and DMRG energies obtained at half-filling. For VQE, we give all energy values from the ten independent optimizations we perform for each number of variational parameters. Unless explicitly specified otherwise, it is implied that the off-site Coulomb interaction and disorder are equal to zero ($d = V = 0$). In some cases VQE optimizations failed, and less than ten columns of data are given. We sort the energy values from lowest to highest from left to right.

# S1 NP ansatz, $U/t = 2$

| Num Parameters | VQE 1 | VQE 2 | VQE 3 | VQE 4 | VQE 5 | VQE 6 | VQE 7 | VQE 8 | VQE 9 | VQE 10 |
|---|---|---|---|---|---|---|---|---|---|---|
| 12 | 0.0000 | 0.0000 | 0.0000 | 0.0000 | 0.0000 | 0.0000 | 0.0000 | 0.0000 | 0.0000 | 0.6530 |
| 20 | -1.2361 | -1.2361 | -1.2361 | -1.2361 | -1.2361 | -1.2361 | -1.2361 | -1.2361 | -1.2361 | -1.2361 |
| 28 | -1.2361 | -1.2361 | -1.2361 | -1.2361 | -1.2361 | -1.2361 | -1.2361 | -1.2361 | -1.2361 | -1.2361 |
| 36 | -1.2361 | -1.2361 | -1.2361 | -1.2361 | -1.2361 | -1.2361 | -1.2361 | -1.2361 | -1.2361 | -1.2361 |
| 44 | -1.2361 | -1.2361 | -1.2361 | -1.2361 | -1.2361 | -1.2361 | -1.2361 | -1.2361 | -1.2361 | -1.2361 |
| 52 | -1.2361 | -1.2361 | -1.2361 | -1.2361 | -1.2361 | -1.2361 | -1.2361 | -1.2361 | -1.2361 | -1.2361 |
| 60 | -1.2361 | -1.2361 | -1.2361 | -1.2361 | -1.2361 | -1.2361 | -1.2361 | -1.2361 | -1.2361 | -1.2361 |
| 68 | -1.2361 | -1.2361 | -1.2361 | -1.2361 | -1.2361 | -1.2361 | -1.2361 | -1.2361 | -1.2361 | -1.2361 |
| 76 | -1.2361 | -1.2361 | -1.2361 | -1.2361 | -1.2361 | -1.2361 | -1.2361 | -1.2361 | -1.2361 | -1.2361 |
| 84 | -1.2361 | -1.2361 | -1.2361 | -1.2361 | -1.2361 | -1.2361 | -1.2361 | -1.2361 | -1.2361 | -1.2361 |
| 92 | -1.2361 | -1.2361 | -1.2361 | -1.2361 | -1.2361 | -1.2361 | -1.2361 | -1.2361 | -1.2361 | -1.2361 |
| 100 | -1.2361 | -1.2361 | -1.2361 | -1.2361 | -1.2361 | -1.2361 | -1.2361 | -1.2361 | -1.2361 | -1.2361 |
| 108 | -1.2361 | -1.2361 | -1.2361 | -1.2361 | -1.2361 | -1.2361 | -1.2361 | -1.2361 | -1.2361 | -1.2361 |
| DMRG Energy: -1.2361 | | | | | | | | | | |

**Table S1** NP ansatz with U/t = 2, VQE Energies and DMRG Energy for lattice 1x2

| Num Parameters | VQE 1 | VQE 2 | VQE 3 | VQE 4 | VQE 5 | VQE 6 | VQE 7 | VQE 8 | VQE 9 | VQE 10 |
|---|---|---|---|---|---|---|---|---|---|---|
| 20 | -0.4142 | -0.4142 | -0.4142 | -0.4142 | -0.4142 | -0.4142 | 0.0000 | 0.0000 | 0.0000 | 0.0000 |
| 34 | -1.8148 | -1.8148 | -1.8104 | -1.8104 | -1.7967 | -1.7956 | -1.7503 | -1.7503 | -1.7503 | -1.7503 |
| 48 | -1.8201 | -1.8201 | -1.8201 | -1.8201 | -1.8201 | -1.8201 | -1.8201 | -1.8201 | -1.8201 | -1.8201 |
| 62 | -1.8201 | -1.8201 | -1.8201 | -1.8201 | -1.8201 | -1.8201 | -1.8201 | -1.8201 | -1.8201 | -1.8201 |
| 76 | -1.8201 | -1.8201 | -1.8201 | -1.8201 | -1.8201 | -1.8201 | -1.8201 | -1.8201 | -1.8201 | -1.8201 |
| 90 | -1.8201 | -1.8201 | -1.8201 | -1.8201 | -1.8201 | -1.8201 | -1.8201 | -1.8201 | -1.8201 | -1.8201 |
| 104 | -1.8201 | -1.8201 | -1.8201 | -1.8201 | -1.8201 | -1.8201 | -1.8201 | -1.8201 | -1.8201 | -1.8201 |
| 118 | -1.8201 | -1.8201 | -1.8201 | -1.8201 | -1.8201 | -1.8201 | -1.8201 | -1.8201 | -1.8201 | -1.8201 |
| 132 | -1.8201 | -1.8201 | -1.8201 | -1.8201 | -1.8201 | -1.8201 | -1.8201 | -1.8201 | -1.8201 | -1.8201 |
| 146 | -1.8201 | -1.8201 | -1.8201 | -1.8201 | -1.8201 | -1.8201 | -1.8201 | -1.8201 | -1.8201 | -1.8201 |
| 160 | -1.8201 | -1.8201 | -1.8201 | -1.8201 | -1.8201 | -1.8201 | -1.8201 | -1.8201 | -1.8201 | -1.8201 |
| 174 | -1.8201 | -1.8201 | -1.8201 | -1.8201 | -1.8201 | -1.8201 | -1.8201 | -1.8201 | -1.8201 | -1.8201 |
| 188 | -1.8201 | -1.8201 | -1.8201 | -1.8201 | -1.8201 | -1.8201 | -1.8201 | -1.8201 | -1.8201 | -1.8201 |
| DMRG Energy: -1.8201 | | | | | | | | | | |

**Table S2** NP ansatz with U/t = 2, VQE Energies and DMRG Energy for lattice 1x3

| Num Parameters | VQE 1 | VQE 2 | VQE 3 | VQE 4 | VQE 5 | VQE 6 | VQE 7 | VQE 8 | VQE 9 | VQE 10 |
|---|---|---|---|---|---|---|---|---|---|---|
| 28 | -0.8508 | -0.8508 | -0.8508 | -0.6818 | -0.6818 | -0.6818 | -0.4142 | -0.4142 | -0.4142 | 0.0000 |
| 48 | -2.8354 | -2.8330 | -2.8330 | -2.8330 | -2.7019 | -2.6621 | -2.5319 | -2.5319 | -2.4202 | -2.0014 |
| 68 | -2.8743 | -2.8737 | -2.8728 | -2.8721 | -2.8718 | -2.8708 | -2.8698 | -2.8690 | -2.8689 | -2.8649 |
| 88 | -2.8755 | -2.8751 | -2.8751 | -2.8751 | -2.8747 | -2.8746 | -2.8746 | -2.8745 | -2.8742 | -2.8681 |
| 108 | -2.8758 | -2.8758 | -2.8756 | -2.8756 | -2.8755 | -2.8755 | -2.8755 | -2.8753 | -2.8753 | -2.8752 |
| 128 | -2.8759 | -2.8759 | -2.8759 | -2.8759 | -2.8759 | -2.8759 | -2.8758 | -2.8758 | -2.8757 | -2.8747 |
| 148 | -2.8759 | -2.8759 | -2.8759 | -2.8759 | -2.8759 | -2.8759 | -2.8758 | -2.8758 | -2.8758 | -2.8758 |
| 168 | -2.8759 | -2.8759 | -2.8759 | -2.8759 | -2.8759 | -2.8759 | -2.8759 | -2.8759 | -2.8759 | -2.8759 |
| 188 | -2.8759 | -2.8759 | -2.8759 | -2.8759 | -2.8759 | -2.8759 | -2.8759 | -2.8759 | -2.8759 | -2.8759 |
| 208 | -2.8759 | -2.8759 | -2.8759 | -2.8759 | -2.8759 | -2.8759 | -2.8759 | -2.8759 | -2.8759 | -2.8759 |
| 228 | -2.8759 | -2.8759 | -2.8759 | -2.8759 | -2.8759 | -2.8759 | -2.8759 | -2.8759 | -2.8759 | -2.8759 |
| 248 | -2.8759 | -2.8759 | -2.8759 | -2.8759 | -2.8759 | -2.8759 | -2.8759 | -2.8759 | -2.8759 | -2.8759 |
| 268 | -2.8759 | -2.8759 | -2.8759 | -2.8759 | -2.8759 | -2.8759 | -2.8759 | -2.8759 | -2.8759 | -2.8759 |
| DMRG Energy: -2.8759 | | | | | | | | | | |

**Table S3** NP ansatz with U/t = 2, VQE Energies and DMRG Energy for lattice 1x4

| Num Parameters | VQE 1 | VQE 2 | VQE 3 | VQE 4 | VQE 5 | VQE 6 | VQE 7 | VQE 8 | VQE 9 | VQE 10 |
|---|---|---|---|---|---|---|---|---|---|---|
| 36 | -1.2049 | -1.2049 | -1.0000 | -1.0000 | -1.0000 | -0.8512 | -0.6873 | -0.4142 | 0.0000 | 0.0000 |
| 62 | -3.4026 | -3.4026 | -3.3967 | -3.3564 | -3.3166 | -3.2787 | -3.2376 | -3.2247 | -3.2067 | -3.1868 |
| 88 | -3.5273 | -3.5244 | -3.5218 | -3.5189 | -3.5177 | -3.5006 | -3.4968 | -3.4931 | -3.4889 | -3.4822 |
| 114 | -3.5478 | -3.5468 | -3.5436 | -3.5425 | -3.5418 | -3.5415 | -3.5404 | -3.5399 | -3.5392 | -3.5385 |
| 140 | -3.5509 | -3.5501 | -3.5499 | -3.5490 | -3.5489 | -3.5483 | -3.5474 | -3.5473 | -3.5470 | -3.5415 |
| 166 | -3.5526 | -3.5523 | -3.5515 | -3.5514 | -3.5511 | -3.5509 | -3.5504 | -3.5503 | -3.5501 | -3.5492 |
| 192 | -3.5533 | -3.5531 | -3.5528 | -3.5528 | -3.5527 | -3.5522 | -3.5516 | -3.5514 | -3.5508 | -3.5498 |
| 218 | -3.5537 | -3.5536 | -3.5534 | -3.5530 | -3.5528 | -3.5528 | -3.5526 | -3.5524 | -3.5522 | -3.5516 |
| 244 | -3.5539 | -3.5536 | -3.5536 | -3.5534 | -3.5533 | -3.5533 | -3.5533 | -3.5532 | -3.5529 | -3.5526 |
| 270 | -3.5540 | -3.5538 | -3.5537 | -3.5537 | -3.5536 | -3.5535 | -3.5534 | -3.5532 | -3.5531 | -3.5531 |
| 296 | -3.5540 | -3.5539 | -3.5538 | -3.5538 | -3.5537 | -3.5536 | -3.5535 | -3.5535 | -3.5534 | -3.5533 |
| 322 | -3.5540 | -3.5539 | -3.5539 | -3.5539 | -3.5538 | -3.5537 | -3.5537 | -3.5537 | -3.5536 | -3.5534 |
| 348 | -3.5540 | -3.5539 | -3.5539 | -3.5539 | -3.5538 | -3.5538 | -3.5538 | -3.5537 | -3.5537 | -3.5537 |
| DMRG Energy: -3.5542 | | | | | | | | | | |

**Table S4** NP ansatz with U/t = 2, VQE Energies and DMRG Energy for lattice 1x5

| Num Parameters | VQE 1 | VQE 2 | VQE 3 | VQE 4 | VQE 5 | VQE 6 | VQE 7 | VQE 8 | VQE 9 | VQE 10 |
|---|---|---|---|---|---|---|---|---|---|---|
| 44 | -1.4375 | -1.4257 | -1.2049 | -1.1116 | -1.1116 | -0.8284 | -0.8284 | -0.8284 | -0.8284 | -0.8284 |
| 76 | -4.3952 | -4.3933 | -4.0694 | -3.8777 | -3.7784 | -3.7764 | -3.7668 | -3.7398 | -3.7280 | -3.6992 |
| 108 | -4.5309 | -4.5247 | -4.5202 | -4.5186 | -4.5102 | -4.4945 | -4.4701 | -4.4589 | -4.4271 | -4.4116 |
| 140 | -4.5368 | -4.5364 | -4.5355 | -4.5353 | -4.5338 | -4.5313 | -4.5308 | -4.5295 | -4.5291 | -4.5230 |
| 172 | -4.5422 | -4.5421 | -4.5405 | -4.5404 | -4.5398 | -4.5395 | -4.5376 | -4.5375 | -4.5321 | -4.5311 |
| 204 | -4.5443 | -4.5440 | -4.5440 | -4.5438 | -4.5437 | -4.5435 | -4.5426 | -4.5420 | -4.5416 | -4.5406 |
| 236 | -4.5451 | -4.5449 | -4.5447 | -4.5445 | -4.5444 | -4.5441 | -4.5439 | -4.5428 | -4.5426 | -4.5413 |
| 268 | -4.5453 | -4.5453 | -4.5452 | -4.5452 | -4.5451 | -4.5451 | -4.5449 | -4.5447 | -4.5444 | -4.5408 |
| 300 | -4.5458 | -4.5455 | -4.5455 | -4.5455 | -4.5455 | -4.5453 | -4.5452 | -4.5452 | -4.5450 | -4.5443 |
| 332 | -4.5458 | -4.5458 | -4.5457 | -4.5457 | -4.5456 | -4.5456 | -4.5455 | -4.5455 | -4.5454 | -4.5454 |
| 364 | -4.5459 | -4.5458 | -4.5458 | -4.5458 | -4.5458 | -4.5457 | -4.5457 | -4.5456 | -4.5456 | -4.5454 |
| 396 | -4.5460 | -4.5459 | -4.5458 | -4.5458 | -4.5458 | -4.5458 | -4.5458 | -4.5457 | -4.5457 | -4.5455 |
| 428 | -4.5460 | -4.5460 | -4.5459 | -4.5458 | -4.5458 | -4.5458 | -4.5457 | -4.5457 | -4.5457 | -4.5455 |
| DMRG Energy: -4.5463 | | | | | | | | | | |

**Table S5** NP ansatz with U/t = 2, VQE Energies and DMRG Energy for lattice 1x6

| Num Parameters | VQE 1 | VQE 2 | VQE 3 | VQE 4 | VQE 5 | VQE 6 | VQE 7 | VQE 8 | VQE 9 | VQE 10 |
|---|---|---|---|---|---|---|---|---|---|---|
| 52 | -1.9023 | -1.9023 | -1.9023 | -1.9023 | -1.7869 | -1.7865 | -1.7599 | -1.6586 | -1.4142 | -1.2099 |
| 90 | -4.9023 | -4.8200 | -4.8038 | -4.7947 | -4.7634 | -4.6996 | -4.6844 | -4.6684 | -4.6229 | -4.5889 |
| 128 | -5.2057 | -5.1508 | -5.1505 | -5.1435 | -5.1148 | -5.1146 | -5.1006 | -5.0937 | -5.0926 | -5.0425 |
| 166 | -5.2517 | -5.2311 | -5.2218 | -5.2151 | -5.2123 | -5.2121 | -5.2115 | -5.2099 | -5.2092 | -5.1900 |
| 204 | -5.2542 | -5.2522 | -5.2521 | -5.2501 | -5.2490 | -5.2443 | -5.2442 | -5.2418 | -5.2400 | -5.2366 |
| 242 | -5.2611 | -5.2604 | -5.2591 | -5.2589 | -5.2589 | -5.2565 | -5.2547 | -5.2533 | -5.2503 | -5.2480 |
| 280 | -5.2631 | -5.2625 | -5.2618 | -5.2618 | -5.2615 | -5.2612 | -5.2609 | -5.2603 | -5.2565 | -5.2562 |
| 318 | -5.2632 | -5.2631 | -5.2631 | -5.2622 | -5.2622 | -5.2620 | -5.2612 | -5.2609 | -5.2585 | -5.2551 |
| 356 | -5.2646 | -5.2643 | -5.2641 | -5.2640 | -5.2637 | -5.2637 | -5.2631 | -5.2627 | -5.2624 | -5.2603 |
| 394 | -5.2651 | -5.2647 | -5.2645 | -5.2645 | -5.2642 | -5.2640 | -5.2638 | -5.2633 | -5.2620 | -5.2615 |
| 432 | -5.2655 | -5.2651 | -5.2651 | -5.2651 | -5.2651 | -5.2651 | -5.2650 | -5.2649 | -5.2644 | -5.2640 |
| 470 | -5.2657 | -5.2656 | -5.2656 | -5.2654 | -5.2652 | -5.2651 | -5.2650 | -5.2649 | -5.2647 | -5.2635 |
| 508 | -5.2658 | -5.2657 | -5.2656 | -5.2655 | -5.2655 | -5.2653 | -5.2653 | -5.2648 | -5.2644 | -5.2638 |
| DMRG Energy: -5.2671 | | | | | | | | | | |

**Table S6** NP ansatz with U/t = 2, VQE Energies and DMRG Energy for lattice 1x7

| Num Parameters | VQE 1 | VQE 2 | VQE 3 | VQE 4 | VQE 5 | VQE 6 | VQE 7 | VQE 8 | VQE 9 | VQE 10 |
|---|---|---|---|---|---|---|---|---|---|---|
| 60 | -2.1443 | -2.0999 | -2.0738 | -2.0486 | -2.0483 | -1.8671 | -1.7031 | -1.3751 | -0.8284 | -0.8284 |
| 104 | -5.9169 | -5.4030 | -5.3721 | -5.3442 | -5.3355 | -5.3275 | -5.2872 | -5.2176 | -5.1103 | -4.9984 |
| 148 | -6.1688 | -6.1164 | -6.0336 | -6.0326 | -6.0051 | -5.9810 | -5.9227 | -5.8150 | -5.7819 | -5.7511 |
| 192 | -6.1832 | -6.1781 | -6.1754 | -6.1736 | -6.1682 | -6.1570 | -6.1390 | -6.1147 | -6.0830 | -6.0469 |
| 236 | -6.2127 | -6.2104 | -6.2029 | -6.2022 | -6.2011 | -6.1978 | -6.1978 | -6.1928 | -6.1877 | -6.1869 |
| 280 | -6.2209 | -6.2173 | -6.2166 | -6.2143 | -6.2137 | -6.2128 | -6.2124 | -6.2100 | -6.2079 | -6.2030 |
| 324 | -6.2198 | -6.2192 | -6.2189 | -6.2187 | -6.2169 | -6.2163 | -6.2130 | -6.2127 | -6.2123 | -6.2115 |
| 368 | -6.2225 | -6.2222 | -6.2220 | -6.2216 | -6.2215 | -6.2212 | -6.2199 | -6.2195 | -6.2192 | -6.2170 |
| 412 | -6.2232 | -6.2232 | -6.2224 | -6.2224 | -6.2222 | -6.2218 | -6.2214 | -6.2210 | -6.2206 | -6.2183 |
| 456 | -6.2235 | -6.2233 | -6.2233 | -6.2227 | -6.2227 | -6.2227 | -6.2227 | -6.2215 | -6.2213 | -6.2207 |
| 500 | -6.2234 | -6.2233 | -6.2233 | -6.2232 | -6.2232 | -6.2231 | -6.2230 | -6.2224 | -6.2208 | -6.2204 |
| 544 | -6.2240 | -6.2240 | -6.2239 | -6.2238 | -6.2237 | -6.2237 | -6.2236 | -6.2235 | -6.2232 | -6.2208 |
| 588 | -6.2245 | -6.2240 | -6.2240 | -6.2240 | -6.2239 | -6.2238 | -6.2236 | -6.2235 | -6.2234 | -6.2233 |
| DMRG Energy: -6.2256 | | | | | | | | | | |

**Table S7** NP ansatz with U/t = 2, VQE Energies and DMRG Energy for lattice 1x8

| Num Parameters | VQE 1 | VQE 2 | VQE 3 | VQE 4 | VQE 5 | VQE 6 | VQE 7 | VQE 8 | VQE 9 | VQE 10 |
|---|---|---|---|---|---|---|---|---|---|---|
| 68 | -2.6287 | -2.6287 | -2.4362 | -2.4353 | -2.3986 | -2.3984 | -2.1582 | -2.1538 | -2.1289 | -2.0000 |
| 118 | -6.2402 | -5.9225 | -5.8661 | -5.8653 | -5.8361 | -5.8244 | -5.8233 | -5.8211 | -5.8007 | -5.7312 |
| 168 | -6.7953 | -6.7076 | -6.7007 | -6.6742 | -6.6719 | -6.6717 | -6.6535 | -6.6373 | -6.6307 | -6.6079 |
| 218 | -6.8922 | -6.8844 | -6.8833 | -6.8746 | -6.8618 | -6.8429 | -6.8415 | -6.8399 | -6.8146 | -6.7919 |
| 268 | -6.9194 | -6.9173 | -6.9140 | -6.9122 | -6.9095 | -6.9050 | -6.9046 | -6.9039 | -6.9012 | -6.8909 |
| 318 | -6.9510 | -6.9502 | -6.9473 | -6.9420 | -6.9390 | -6.9384 | -6.9379 | -6.9379 | -6.9369 | -6.9309 |
| 368 | -6.9584 | -6.9553 | -6.9549 | -6.9539 | -6.9524 | -6.9522 | -6.9517 | -6.9500 | -6.9476 | -6.9439 |
| 418 | -6.9602 | -6.9601 | -6.9592 | -6.9580 | -6.9577 | -6.9561 | -6.9538 | -6.9524 | -6.9511 | -6.9463 |
| 468 | -6.9647 | -6.9645 | -6.9635 | -6.9619 | -6.9616 | -6.9613 | -6.9609 | -6.9592 | -6.9571 | -6.9550 |
| 518 | -6.9665 | -6.9663 | -6.9652 | -6.9647 | -6.9635 | -6.9631 | -6.9629 | -6.9622 | -6.9597 | -6.9579 |
| 568 | -6.9675 | -6.9672 | -6.9663 | -6.9653 | -6.9649 | -6.9645 | -6.9643 | -6.9640 | -6.9631 | -6.9560 |
| 618 | -6.9683 | -6.9680 | -6.9678 | -6.9675 | -6.9673 | -6.9669 | -6.9665 | -6.9654 | -6.9640 | -6.9631 |
| 668 | -6.9688 | -6.9687 | -6.9685 | -6.9684 | -6.9683 | -6.9677 | -6.9669 | -6.9667 | -6.9657 | -6.9651 |
| DMRG Energy: -6.9712 | | | | | | | | | | |

**Table S8** NP ansatz with U/t = 2, VQE Energies and DMRG Energy for lattice 1x9

| Num Parameters | VQE 1 | VQE 2 | VQE 3 | VQE 4 | VQE 5 | VQE 6 | VQE 7 | VQE 8 | VQE 9 | VQE 10 |
|---|---|---|---|---|---|---|---|---|---|---|
| 76 | -2.7231 | -2.7086 | -2.7086 | -2.7014 | -2.6927 | -2.4858 | -2.4216 | -2.3165 | -2.1741 | -2.1741 |
| 132 | -6.8240 | -6.7646 | -6.6550 | -6.6229 | -6.6195 | -6.5423 | -6.4877 | -6.3717 | -6.2337 | -6.2337 |
| 188 | -7.6191 | -7.6055 | -7.4324 | -7.4228 | -7.4129 | -7.3487 | -7.3413 | -7.3362 | -7.3154 | -7.3108 |
| 244 | -7.8146 | -7.8109 | -7.7643 | -7.7550 | -7.7447 | -7.7236 | -7.7095 | -7.7014 | -7.6369 | -7.5822 |
| 300 | -7.8710 | -7.8694 | -7.8586 | -7.8542 | -7.8487 | -7.8203 | -7.8140 | -7.8080 | -7.7882 | -7.7809 |
| 356 | -7.8885 | -7.8873 | -7.8858 | -7.8856 | -7.8849 | -7.8845 | -7.8840 | -7.8838 | -7.8823 | -7.8769 |
| 412 | -7.9003 | -7.8995 | -7.8970 | -7.8956 | -7.8929 | -7.8929 | -7.8909 | -7.8908 | -7.8886 | -7.8762 |
| 468 | -7.9013 | -7.8995 | -7.8983 | -7.8972 | -7.8971 | -7.8970 | -7.8968 | -7.8951 | -7.8944 | -7.8930 |
| 524 | -7.9023 | -7.9019 | -7.9012 | -7.9007 | -7.9003 | -7.8991 | -7.8988 | -7.8987 | -7.8981 | -7.8935 |
| 580 | -7.9040 | -7.9038 | -7.9023 | -7.9022 | -7.9018 | -7.9012 | -7.9011 | -7.9002 | -7.8995 | -7.8991 |
| 636 | -7.9043 | -7.9041 | -7.9040 | -7.9033 | -7.9030 | -7.9030 | -7.9026 | -7.9021 | -7.9019 | -7.8984 |
| 692 | -7.9042 | -7.9039 | -7.9038 | -7.9038 | -7.9037 | -7.9032 | -7.9031 | -7.9029 | -7.9014 | -7.9014 |
| 748 | -7.9049 | -7.9048 | -7.9046 | -7.9046 | -7.9045 | -7.9045 | -7.9043 | -7.9041 | -7.9040 | -7.9033 |
| DMRG Energy: -7.9087 | | | | | | | | | | |

**Table S9** NP ansatz with U/t = 2, VQE Energies and DMRG Energy for lattice 1x10

| Num Parameters | VQE 1 | VQE 2 | VQE 3 | VQE 4 | VQE 5 | VQE 6 | VQE 7 | VQE 8 | VQE 9 | VQE 10 |
|---|---|---|---|---|---|---|---|---|---|---|
| 84 | -3.0466 | -3.0292 | -3.0237 | -3.0096 | -3.0093 | -3.0093 | -3.0093 | -2.9126 | -2.9023 | -2.8275 |
| 146 | -7.3832 | -7.3373 | -7.2518 | -7.2315 | -7.2263 | -7.2041 | -7.1348 | -7.1001 | -7.0701 | -7.0309 |
| 208 | -8.3206 | -8.2725 | -8.2600 | -8.2515 | -8.2448 | -8.2441 | -8.2423 | -8.2395 | -8.1811 | -8.1015 |
| 270 | -8.5511 | -8.5365 | -8.4898 | -8.4665 | -8.4634 | -8.4381 | -8.4319 | -8.4283 | -8.4097 | -8.3549 |
| 332 | -8.6058 | -8.5891 | -8.5753 | -8.5721 | -8.5706 | -8.5621 | -8.5504 | -8.5448 | -8.5362 | -8.5308 |
| 394 | -8.6367 | -8.6111 | -8.6070 | -8.6062 | -8.5934 | -8.5875 | -8.5855 | -8.5851 | -8.5826 | -8.5622 |
| 456 | -8.6348 | -8.6332 | -8.6320 | -8.6318 | -8.6305 | -8.6262 | -8.6224 | -8.6149 | -8.6142 | -8.5923 |
| 518 | -8.6442 | -8.6436 | -8.6425 | -8.6416 | -8.6411 | -8.6369 | -8.6352 | -8.6332 | -8.6302 | -8.6171 |
| 580 | -8.6561 | -8.6539 | -8.6488 | -8.6485 | -8.6386 | -8.6316 | -8.6315 | -8.6313 | -8.6290 | -8.6200 |
| 642 | -8.6570 | -8.6556 | -8.6428 | -8.6427 | -8.6411 | -8.6402 | -8.6398 | -8.6389 | -8.6386 | -8.6260 |
| 704 | -8.6570 | -8.6500 | -8.6495 | -8.6468 | -8.6450 | -8.6445 | -8.6439 | -8.6429 | -8.6382 | -8.6304 |
| 766 | -8.6559 | -8.6487 | -8.6480 | -8.6469 | -8.6466 | -8.6456 | -8.6415 | -8.6391 | -8.6375 | -8.6321 |
| 828 | -8.6551 | -8.6492 | -8.6482 | -8.6479 | -8.6476 | -8.6461 | -8.6399 | -8.6392 | -8.6366 | -8.6260 |
| DMRG Energy: -8.6706 | | | | | | | | | | |

**Table S10** NP ansatz with U/t = 2, VQE Energies and DMRG Energy for lattice 1x11

| Num Parameters | VQE 1 | VQE 2 | VQE 3 | VQE 4 | VQE 5 | VQE 6 | VQE 7 | VQE 8 | VQE 9 | VQE 10 |
|---|---|---|---|---|---|---|---|---|---|---|
| 92 | -3.3368 | -3.3177 | -3.3177 | -3.3177 | -3.3177 | -3.2872 | -3.2872 | -3.2872 | -3.2872 | -3.1071 |
| 160 | -8.1345 | -8.0630 | -7.9375 | -7.9282 | -7.8145 | -7.7251 | -7.6569 | -7.6510 | -7.6356 | -7.5642 |
| 228 | -9.1294 | -8.8827 | -8.8820 | -8.8708 | -8.8507 | -8.8092 | -8.7901 | -8.7888 | -8.7626 | -8.6769 |
| 296 | -9.3712 | -9.3461 | -9.2856 | -9.2651 | -9.2286 | -9.1969 | -9.1857 | -9.1805 | -9.0848 | -9.0407 |
| 364 | -9.4530 | -9.4500 | -9.4460 | -9.4093 | -9.4019 | -9.3970 | -9.3688 | -9.3626 | -9.3567 | -9.3288 |
| 432 | -9.5305 | -9.4907 | -9.4667 | -9.4473 | -9.4429 | -9.4381 | -9.4264 | -9.4009 | -9.3440 | -9.2219 |
| 500 | -9.4951 | -9.4899 | -9.4828 | -9.4765 | -9.4624 | -9.4489 | -9.4450 | -9.4442 | -9.4426 | -9.4165 |
| 568 | -9.5073 | -9.5019 | -9.4831 | -9.4780 | -9.4599 | -9.4515 | -9.4512 | -9.4189 | -9.3981 | -9.3516 |
| 636 | -9.4450 | -9.4434 | -9.4292 | -9.4217 | -9.4124 | -9.4037 | -9.3994 | -9.3440 | -9.3376 | -9.3239 |
| 704 | -9.4577 | -9.4141 | -9.4124 | -9.4054 | -9.3377 | -9.3321 | -9.3287 | -9.2851 | -9.2817 | -9.2204 |
| 772 | -9.3941 | -9.3280 | -9.3127 | -9.2748 | -9.1917 | -9.1462 | -9.1393 | -9.1205 | -9.0965 | -9.0697 |
| 840 | -9.5548 | -9.5493 | -9.5425 | -9.5420 | -9.5278 | -9.5245 | -9.5045 | -9.5002 | -9.4830 | -9.4615 |
| 908 | -9.5534 | -9.5401 | -9.5396 | -9.5390 | -9.5385 | -9.5261 | -9.5138 | -9.5133 | -9.4878 | -9.4843 |
| DMRG Energy: -9.5938 | | | | | | | | | | |

**Table S11** NP ansatz with U/t = 2, VQE Energies and DMRG Energy for lattice 1x12

| Num Parameters | VQE 1 | VQE 2 | VQE 3 | VQE 4 | VQE 5 | VQE 6 | VQE 7 | VQE 8 | VQE 9 | VQE 10 |
|---|---|---|---|---|---|---|---|---|---|---|
| 32 | -2.0000 | -2.0000 | -2.0000 | -2.0000 | -2.0000 | -2.0000 | -2.0000 | -0.4142 | -0.4142 | 0.0000 |
| 56 | -2.7702 | -2.7450 | -2.7325 | -2.7322 | -2.7322 | -2.7282 | -2.7248 | -2.7218 | -2.6155 | -2.5583 |
| 80 | -2.8177 | -2.7964 | -2.7927 | -2.7883 | -2.7539 | -2.7539 | -2.6858 | -2.6858 | -2.6858 | -2.6853 |
| 104 | -2.8284 | -2.8284 | -2.8284 | -2.8284 | -2.8284 | -2.8284 | -2.8284 | -2.8237 | -2.8118 | -2.7862 |
| 128 | -2.8284 | -2.8284 | -2.8284 | -2.8284 | -2.8284 | -2.8284 | -2.8284 | -2.8263 | -2.8257 | -2.8207 |
| 152 | -2.8284 | -2.8284 | -2.8284 | -2.8284 | -2.8284 | -2.8284 | -2.8284 | -2.8284 | -2.8284 | -2.8284 |
| 176 | -2.8284 | -2.8284 | -2.8284 | -2.8284 | -2.8284 | -2.8284 | -2.8284 | -2.8284 | -2.8284 | -2.8284 |
| 200 | -2.8284 | -2.8284 | -2.8284 | -2.8284 | -2.8284 | -2.8284 | -2.8284 | -2.8284 | -2.8284 | -2.8284 |
| 224 | -2.8284 | -2.8284 | -2.8284 | -2.8284 | -2.8284 | -2.8284 | -2.8284 | -2.8284 | -2.8284 | -2.8284 |
| 248 | -2.8284 | -2.8284 | -2.8284 | -2.8284 | -2.8284 | -2.8284 | -2.8284 | -2.8284 | -2.8284 | -2.8284 |
| 272 | -2.8284 | -2.8284 | -2.8284 | -2.8284 | -2.8284 | -2.8284 | -2.8284 | -2.8284 | -2.8284 | -2.8284 |
| 296 | -2.8284 | -2.8284 | -2.8284 | -2.8284 | -2.8284 | -2.8284 | -2.8284 | -2.8284 | -2.8284 | -2.8284 |
| 320 | -2.8284 | -2.8284 | -2.8284 | -2.8284 | -2.8284 | -2.8284 | -2.8284 | -2.8284 | -2.8284 | -2.8284 |
| DMRG Energy: -2.8284 | | | | | | | | | | |

**Table S12** NP ansatz with U/t = 2, VQE Energies and DMRG Energy for lattice 2x2

| Num Parameters | VQE 1 | VQE 2 | VQE 3 | VQE 4 | VQE 5 | VQE 6 | VQE 7 | VQE 8 | VQE 9 | VQE 10 |
|---|---|---|---|---|---|---|---|---|---|---|
| 52 | -2.6436 | -2.6296 | -2.4441 | -2.4441 | -2.4441 | -2.3256 | -2.3256 | -2.0000 | -2.0000 | -2.0000 |
| 92 | -4.9239 | -4.6551 | -4.5325 | -4.5133 | -4.4072 | -4.3481 | -4.3481 | -4.3219 | -4.3219 | -4.3219 |
| 132 | -5.0294 | -5.0068 | -4.9969 | -4.9924 | -4.9912 | -4.9836 | -4.9797 | -4.9714 | -4.9433 | -4.9341 |
| 172 | -5.1317 | -5.1314 | -5.1313 | -5.1235 | -5.1218 | -5.1167 | -5.1152 | -5.1125 | -5.1106 | -5.0846 |
| 212 | -5.1552 | -5.1547 | -5.1460 | -5.1456 | -5.1449 | -5.1434 | -5.1396 | -5.1374 | -5.1350 | -5.1339 |
| 252 | -5.1565 | -5.1533 | -5.1526 | -5.1500 | -5.1495 | -5.1493 | -5.1493 | -5.1493 | -5.1490 | -5.1430 |
| 292 | -5.1572 | -5.1569 | -5.1567 | -5.1565 | -5.1561 | -5.1555 | -5.1555 | -5.1552 | -5.1495 | -5.1424 |
| 332 | -5.1579 | -5.1579 | -5.1575 | -5.1565 | -5.1564 | -5.1561 | -5.1560 | -5.1558 | -5.1505 | -5.1488 |
| 372 | -5.1587 | -5.1577 | -5.1575 | -5.1571 | -5.1567 | -5.1561 | -5.1559 | -5.1555 | -5.1554 | -5.1524 |
| 412 | -5.1582 | -5.1579 | -5.1579 | -5.1578 | -5.1576 | -5.1574 | -5.1574 | -5.1572 | -5.1569 | -5.1558 |
| 452 | -5.1589 | -5.1589 | -5.1588 | -5.1588 | -5.1587 | -5.1587 | -5.1585 | -5.1585 | -5.1584 | -5.1584 |
| 492 | -5.1590 | -5.1589 | -5.1589 | -5.1588 | -5.1588 | -5.1588 | -5.1588 | -5.1588 | -5.1583 | -5.1583 |
| 532 | -5.1589 | -5.1589 | -5.1588 | -5.1588 | -5.1585 | -5.1583 | -5.1583 | -5.1581 | -5.1572 | -5.1557 |
| DMRG Energy: -5.1592 | | | | | | | | | | |

**Table S13** NP ansatz with U/t = 2, VQE Energies and DMRG Energy for lattice 2x3

| Num Parameters | VQE 1 | VQE 2 | VQE 3 | VQE 4 | VQE 5 | VQE 6 | VQE 7 | VQE 8 | VQE 9 | VQE 10 |
|---|---|---|---|---|---|---|---|---|---|---|
| 84 | -4.3471 | -4.3471 | -4.2564 | -4.2219 | -4.1379 | -4.1379 | -4.1379 | -4.0608 | -3.9269 | -3.9269 |
| 150 | -7.1217 | -7.1217 | -7.1217 | -7.1217 | -7.1217 | -7.1217 | -7.1217 | -7.1217 | -6.9658 | -6.8878 |
| 216 | -7.6340 | -7.5588 | -7.5585 | -7.5585 | -7.5585 | -7.5585 | -7.5585 | -7.5585 | -7.5585 | -7.5585 |
| 282 | -7.7836 | -7.7836 | -7.7836 | -7.7836 | -7.7836 | -7.7836 | -7.7836 | -7.7836 | -7.7836 | -7.7738 |
| 348 | -7.8645 | -7.8645 | -7.8645 | -7.8645 | -7.8645 | -7.8645 | -7.8645 | -7.8645 | -7.8645 | -7.8645 |
| 414 | -7.9002 | -7.9002 | -7.9002 | -7.9002 | -7.9002 | -7.9002 | -7.9002 | -7.9002 | -7.9002 | -7.9001 |
| 480 | -7.9166 | -7.9166 | -7.9166 | -7.9166 | -7.9166 | -7.9166 | -7.9166 | -7.9166 | -7.9166 | -7.9166 |
| 546 | -7.9247 | -7.9246 | -7.9246 | -7.9246 | -7.9246 | -7.9246 | -7.9245 | -7.9245 | -7.9245 | -7.9244 |
| 612 | -7.9333 | -7.9332 | -7.9331 | -7.9330 | -7.9328 | -7.9298 | -7.9298 | -7.9296 | -7.9291 | -7.9289 |
| 678 | -7.9782 | -7.9678 | -7.9460 | -7.9405 | -7.9373 | -7.9373 | -7.9373 | -7.9371 | -7.9370 | -7.9349 |
| 744 | -7.9793 | -7.9785 | -7.9758 | -7.9682 | -7.9676 | -7.9622 | -7.9617 | -7.9596 | -7.9583 | -7.9493 |
| 810 | -7.9833 | -7.9824 | -7.9817 | -7.9817 | -7.9815 | -7.9809 | -7.9797 | -7.9781 | -7.9736 | -7.9703 |
| 876 | -7.9838 | -7.9837 | -7.9831 | -7.9831 | -7.9830 | -7.9829 | -7.9827 | -7.9827 | -7.9814 | -7.9749 |
| DMRG Energy: -7.9865 | | | | | | | | | | |

**Table S14** NP ansatz with U/t = 2, VQE Energies and DMRG Energy for lattice 3x3

# S2 EP ansatz, $U/t = 2$

| Num Parameters | VQE 1 | VQE 2 | VQE 3 | VQE 4 | VQE 5 | VQE 6 | VQE 7 | VQE 8 | VQE 9 | VQE 10 |
|---|---|---|---|---|---|---|---|---|---|---|
| 14 | -1.0000 | -1.0000 | -1.0000 | -1.0000 | -1.0000 | -1.0000 | -1.0000 | -1.0000 | -1.0000 | -1.0000 |
| 20 | -1.0000 | -1.0000 | -1.0000 | -1.0000 | -1.0000 | -1.0000 | -1.0000 | -1.0000 | -1.0000 | -1.0000 |
| 26 | -1.2361 | -1.2361 | -1.2361 | -1.2361 | -1.2361 | -1.2361 | -1.2361 | -1.2361 | -1.2361 | -1.0000 |
| 32 | -1.2361 | -1.2361 | -1.2361 | -1.2361 | -1.2361 | -1.2361 | -1.2361 | -1.2361 | -1.2361 | -1.2361 |
| 38 | -1.2361 | -1.2361 | -1.2361 | -1.2361 | -1.2361 | -1.2361 | -1.2361 | -1.2361 | -1.2361 | -1.2361 |
| 44 | -1.2361 | -1.2361 | -1.2361 | -1.2361 | -1.2361 | -1.2361 | -1.2361 | -1.2361 | -1.2361 | -1.2361 |
| 50 | -1.2361 | -1.2361 | -1.2361 | -1.2361 | -1.2361 | -1.2361 | -1.2361 | -1.2361 | -1.2361 | -1.2361 |
| 56 | -1.2361 | -1.2361 | -1.2361 | -1.2361 | -1.2361 | -1.2361 | -1.2361 | -1.2361 | -1.2361 | -1.2361 |
| 62 | -1.2361 | -1.2361 | -1.2361 | -1.2361 | -1.2361 | -1.2361 | -1.2361 | -1.2361 | -1.2361 | -1.2361 |
| 68 | -1.2361 | -1.2361 | -1.2361 | -1.2361 | -1.2361 | -1.2361 | -1.2361 | -1.2361 | -1.2361 | -1.0000 |
| 74 | -1.2361 | -1.2361 | -1.2361 | -1.2361 | -1.2361 | -1.2361 | -1.2361 | -1.2361 | -1.2361 | -1.0000 |
| 80 | -1.2361 | -1.2361 | -1.2361 | -1.2361 | -1.2361 | -1.2361 | -1.2361 | -1.2361 | -1.2361 | -1.2361 |
| 86 | -1.2361 | -1.2361 | -1.2361 | -1.2361 | -1.2361 | -1.2361 | -1.2361 | -1.2361 | -1.2361 | -1.2361 |
| DMRG Energy: -1.2361 | | | | | | | | | | |

**Table S15** EP ansatz with U/t = 2, VQE Energies and DMRG Energy for lattice 1x2

| Num Parameters | VQE 1 | VQE 2 | VQE 3 | VQE 4 | VQE 5 | VQE 6 | VQE 7 | VQE 8 | VQE 9 | VQE 10 |
|---|---|---|---|---|---|---|---|---|---|---|
| 22 | -1.5400 | -1.5400 | -1.5400 | -1.5400 | -1.5400 | -1.5400 | -1.5400 | -1.5400 | -1.5400 | -1.5400 |
| 32 | -1.7493 | -1.7271 | -1.7271 | -1.6667 | -1.6664 | -1.6664 | -1.6664 | -1.6439 | -1.6439 | -1.6422 |
| 42 | -1.8201 | -1.8201 | -1.8201 | -1.8190 | -1.8189 | -1.8189 | -1.8186 | -1.8175 | -1.8175 | -1.8009 |
| 52 | -1.8201 | -1.8201 | -1.8201 | -1.8201 | -1.8201 | -1.8201 | -1.8201 | -1.8201 | -1.8201 | -1.8201 |
| 62 | -1.8201 | -1.8201 | -1.8201 | -1.8201 | -1.8201 | -1.8201 | -1.8201 | -1.8201 | -1.8201 | -1.8201 |
| 72 | -1.8201 | -1.8201 | -1.8201 | -1.8201 | -1.8201 | -1.8201 | -1.8201 | -1.8201 | -1.8201 | -1.8201 |
| 82 | -1.8201 | -1.8201 | -1.8201 | -1.8201 | -1.8201 | -1.8201 | -1.8201 | -1.8201 | -1.8201 | -1.8201 |
| 92 | -1.8201 | -1.8201 | -1.8201 | -1.8201 | -1.8201 | -1.8201 | -1.8201 | -1.8201 | -1.8201 | -1.8201 |
| 102 | -1.8201 | -1.8201 | -1.8201 | -1.8201 | -1.8201 | -1.8201 | -1.8201 | -1.8201 | -1.8201 | -1.8201 |
| 112 | -1.8201 | -1.8201 | -1.8201 | -1.8201 | -1.8201 | -1.8201 | -1.8201 | -1.8201 | -1.8201 | -1.8201 |
| 122 | -1.8201 | -1.8201 | -1.8201 | -1.8201 | -1.8201 | -1.8201 | -1.8201 | -1.8201 | -1.8201 | -1.8201 |
| 132 | -1.8201 | -1.8201 | -1.8201 | -1.8201 | -1.8201 | -1.8201 | -1.8201 | -1.8201 | -1.8201 | -1.8201 |
| 142 | -1.8201 | -1.8201 | -1.8201 | -1.8201 | -1.8201 | -1.8201 | -1.8201 | -1.8201 | -1.8201 | -1.8201 |
| DMRG Energy: -1.8201 | | | | | | | | | | |

**Table S16** EP ansatz with U/t = 2, VQE Energies and DMRG Energy for lattice 1x3

| Num Parameters | VQE 1 | VQE 2 | VQE 3 | VQE 4 | VQE 5 | VQE 6 | VQE 7 | VQE 8 | VQE 9 | VQE 10 |
|---|---|---|---|---|---|---|---|---|---|---|
| 30 | -2.2263 | -2.2263 | -2.2263 | -2.2263 | -2.2263 | -2.2263 | -2.2263 | -2.2263 | -2.2263 | -2.2263 |
| 44 | -2.4970 | -2.4970 | -2.4970 | -2.4970 | -2.4970 | -2.4970 | -2.4970 | -2.4970 | -2.4970 | -2.4814 |
| 58 | -2.8452 | -2.8452 | -2.8421 | -2.8366 | -2.8340 | -2.7979 | -2.7956 | -2.7956 | -2.7188 | -2.6582 |
| 72 | -2.8646 | -2.8643 | -2.8636 | -2.8636 | -2.8636 | -2.8625 | -2.8613 | -2.8544 | -2.8431 | -2.8067 |
| 86 | -2.8733 | -2.8719 | -2.8707 | -2.8701 | -2.8700 | -2.8692 | -2.8676 | -2.8667 | -2.8641 | -2.8602 |
| 100 | -2.8757 | -2.8748 | -2.8743 | -2.8739 | -2.8730 | -2.8728 | -2.8728 | -2.8727 | -2.8698 | -2.8694 |
| 114 | -2.8752 | -2.8750 | -2.8747 | -2.8744 | -2.8741 | -2.8740 | -2.8734 | -2.8728 | -2.8696 | -2.8694 |
| 128 | -2.8754 | -2.8754 | -2.8753 | -2.8752 | -2.8751 | -2.8749 | -2.8749 | -2.8745 | -2.8744 | -2.8743 |
| 142 | -2.8757 | -2.8756 | -2.8754 | -2.8753 | -2.8752 | -2.8752 | -2.8749 | -2.8749 | -2.8749 | -2.8746 |
| 156 | -2.8757 | -2.8757 | -2.8757 | -2.8756 | -2.8756 | -2.8756 | -2.8754 | -2.8753 | -2.8750 | -2.8745 |
| 170 | -2.8759 | -2.8758 | -2.8757 | -2.8757 | -2.8757 | -2.8757 | -2.8756 | -2.8755 | -2.8755 | -2.8752 |
| 184 | -2.8758 | -2.8758 | -2.8757 | -2.8757 | -2.8756 | -2.8756 | -2.8756 | -2.8756 | -2.8755 | -2.8753 |
| 198 | -2.8759 | -2.8759 | -2.8759 | -2.8759 | -2.8758 | -2.8758 | -2.8758 | -2.8758 | -2.8758 | -2.8758 |
| DMRG Energy: -2.8759 | | | | | | | | | | |

**Table S17** EP ansatz with U/t = 2, VQE Energies and DMRG Energy for lattice 1x4

| Num Parameters | VQE 1 | VQE 2 | VQE 3 | VQE 4 | VQE 5 | VQE 6 | VQE 7 | VQE 8 | VQE 9 | VQE 10 |
|---|---|---|---|---|---|---|---|---|---|---|
| 38 | -2.8863 | -2.8863 | -2.8863 | -2.8863 | -2.8863 | -2.8863 | -2.8863 | -2.8863 | -2.8863 | -2.8863 |
| 56 | -3.2509 | -3.2508 | -3.2508 | -3.2508 | -3.2508 | -3.2108 | -3.1835 | -3.1791 | -3.1791 | -3.1056 |
| 74 | -3.4609 | -3.4551 | -3.4519 | -3.4296 | -3.4277 | -3.4248 | -3.4179 | -3.3996 | -3.3942 | -3.3828 |
| 92 | -3.4964 | -3.4963 | -3.4951 | -3.4904 | -3.4882 | -3.4881 | -3.4853 | -3.4833 | -3.4827 | -3.4746 |
| 110 | -3.5323 | -3.5202 | -3.5190 | -3.5187 | -3.5163 | -3.5143 | -3.5107 | -3.5055 | -3.5025 | -3.5022 |
| 128 | -3.5394 | -3.5378 | -3.5357 | -3.5355 | -3.5335 | -3.5323 | -3.5311 | -3.5296 | -3.5267 | -3.5242 |
| 146 | -3.5462 | -3.5454 | -3.5445 | -3.5428 | -3.5422 | -3.5398 | -3.5395 | -3.5377 | -3.5348 | -3.5321 |
| 164 | -3.5486 | -3.5477 | -3.5475 | -3.5462 | -3.5453 | -3.5450 | -3.5438 | -3.5438 | -3.5433 | -3.5384 |
| 182 | -3.5489 | -3.5486 | -3.5479 | -3.5469 | -3.5467 | -3.5466 | -3.5454 | -3.5452 | -3.5448 | -3.5443 |
| 200 | -3.5496 | -3.5491 | -3.5480 | -3.5474 | -3.5473 | -3.5466 | -3.5465 | -3.5462 | -3.5452 | -3.5427 |
| 218 | -3.5520 | -3.5504 | -3.5503 | -3.5502 | -3.5500 | -3.5499 | -3.5491 | -3.5489 | -3.5489 | -3.5475 |
| 236 | -3.5521 | -3.5510 | -3.5508 | -3.5506 | -3.5506 | -3.5501 | -3.5497 | -3.5496 | -3.5493 | -3.5491 |
| 254 | -3.5515 | -3.5514 | -3.5513 | -3.5513 | -3.5512 | -3.5511 | -3.5510 | -3.5508 | -3.5507 | -3.5503 |
| DMRG Energy: -3.5542 | | | | | | | | | | |

**Table S18** EP ansatz with U/t = 2, VQE Energies and DMRG Energy for lattice 1x5

| Num Parameters | VQE 1 | VQE 2 | VQE 3 | VQE 4 | VQE 5 | VQE 6 | VQE 7 | VQE 8 | VQE 9 | VQE 10 |
|---|---|---|---|---|---|---|---|---|---|---|
| 46 | -3.5527 | -3.5527 | -3.5527 | -3.5527 | -3.5527 | -3.5527 | -3.5527 | -3.5527 | -3.5527 | -3.5527 |
| 68 | -3.9538 | -3.9234 | -3.9229 | -3.9229 | -3.9229 | -3.9229 | -3.9229 | -3.9229 | -3.9228 | -3.9228 |
| 90 | -4.3252 | -4.2924 | -4.2924 | -4.2924 | -4.2924 | -4.2362 | -4.2259 | -4.2139 | -4.2073 | -4.1773 |
| 112 | -4.4801 | -4.4699 | -4.4436 | -4.4390 | -4.4046 | -4.4042 | -4.4027 | -4.3897 | -4.3642 | -4.2888 |
| 134 | -4.4884 | -4.4835 | -4.4785 | -4.4748 | -4.4596 | -4.4586 | -4.4541 | -4.4248 | -4.3999 | -4.3927 |
| 156 | -4.5164 | -4.5033 | -4.4984 | -4.4968 | -4.4901 | -4.4882 | -4.4865 | -4.4783 | -4.4766 | -4.4508 |
| 178 | -4.5216 | -4.5185 | -4.5156 | -4.5031 | -4.4973 | -4.4972 | -4.4948 | -4.4869 | -4.4849 | -4.4491 |
| 200 | -4.5333 | -4.5249 | -4.5243 | -4.5225 | -4.5190 | -4.5137 | -4.5124 | -4.5068 | -4.5047 | -4.5010 |
| 222 | -4.5286 | -4.5284 | -4.5278 | -4.5258 | -4.5227 | -4.5207 | -4.5201 | -4.5183 | -4.5136 | -4.5041 |
| 244 | -4.5375 | -4.5328 | -4.5327 | -4.5305 | -4.5298 | -4.5212 | -4.5212 | -4.5207 | -4.5199 | -4.5137 |
| 266 | -4.5365 | -4.5342 | -4.5332 | -4.5312 | -4.5308 | -4.5285 | -4.5278 | -4.5275 | -4.5200 | -4.5179 |
| 288 | -4.5403 | -4.5386 | -4.5370 | -4.5352 | -4.5333 | -4.5328 | -4.5323 | -4.5310 | -4.5256 | -4.5210 |
| 310 | -4.5382 | -4.5376 | -4.5375 | -4.5372 | -4.5371 | -4.5356 | -4.5346 | -4.5312 | -4.5306 | -4.5251 |
| DMRG Energy: -4.5463 | | | | | | | | | | |

**Table S19** EP ansatz with U/t = 2, VQE Energies and DMRG Energy for lattice 1x6

| Num Parameters | VQE 1 | VQE 2 | VQE 3 | VQE 4 | VQE 5 | VQE 6 | VQE 7 | VQE 8 | VQE 9 | VQE 10 |
|---|---|---|---|---|---|---|---|---|---|---|
| 54 | -4.2177 | -4.2177 | -4.2177 | -4.2177 | -4.2177 | -4.2177 | -4.2177 | -4.2177 | -4.2177 | -4.2177 |
| 80 | -4.7437 | -4.7437 | -4.6770 | -4.6770 | -4.6770 | -4.6770 | -4.6770 | -4.6539 | -4.6256 | -4.6256 |
| 106 | -5.0013 | -4.9710 | -4.9682 | -4.9656 | -4.9532 | -4.9517 | -4.9498 | -4.9393 | -4.8875 | -4.8015 |
| 132 | -5.1471 | -5.1244 | -5.1144 | -5.1139 | -5.0994 | -5.0914 | -5.0726 | -5.0724 | -5.0691 | -5.0090 |
| 158 | -5.1727 | -5.1567 | -5.1505 | -5.1497 | -5.1473 | -5.1460 | -5.1231 | -5.1189 | -5.0945 | -5.0885 |
| 184 | -5.2119 | -5.2104 | -5.1983 | -5.1858 | -5.1796 | -5.1795 | -5.1784 | -5.1544 | -5.1311 | -5.1124 |
| 210 | -5.2357 | -5.2260 | -5.2217 | -5.2150 | -5.2139 | -5.2128 | -5.2117 | -5.2090 | -5.2078 | -5.1812 |
| 236 | -5.2383 | -5.2309 | -5.2286 | -5.2271 | -5.2247 | -5.2245 | -5.2241 | -5.2223 | -5.2189 | -5.1952 |
| 262 | -5.2399 | -5.2381 | -5.2358 | -5.2355 | -5.2316 | -5.2312 | -5.2296 | -5.2275 | -5.2228 | -5.2219 |
| 288 | -5.2455 | -5.2434 | -5.2403 | -5.2401 | -5.2390 | -5.2379 | -5.2372 | -5.2353 | -5.2274 | -5.2131 |
| 314 | -5.2453 | -5.2450 | -5.2427 | -5.2425 | -5.2421 | -5.2410 | -5.2370 | -5.2347 | -5.2306 | -5.2176 |
| 340 | -5.2515 | -5.2484 | -5.2467 | -5.2461 | -5.2450 | -5.2447 | -5.2407 | -5.2373 | -5.2323 | -5.2131 |
| 366 | -5.2542 | -5.2527 | -5.2522 | -5.2492 | -5.2474 | -5.2471 | -5.2468 | -5.2426 | -5.2396 | -5.2368 |
| DMRG Energy: -5.2671 | | | | | | | | | | |

**Table S20** EP ansatz with U/t = 2, VQE Energies and DMRG Energy for lattice 1x7

| Num Parameters | VQE 1 | VQE 2 | VQE 3 | VQE 4 | VQE 5 | VQE 6 | VQE 7 | VQE 8 | VQE 9 | VQE 10 |
|---|---|---|---|---|---|---|---|---|---|---|
| 62 | -4.8830 | -4.8830 | -4.8830 | -4.8830 | -4.8830 | -4.8830 | -4.8830 | -4.8830 | -4.8830 | -4.8830 |
| 92 | -5.4188 | -5.4077 | -5.4077 | -5.4077 | -5.4032 | -5.3881 | -5.3868 | -5.3622 | -5.3184 | -5.3147 |
| 122 | -5.8169 | -5.8108 | -5.8012 | -5.8009 | -5.7868 | -5.7846 | -5.7762 | -5.7760 | -5.7549 | -5.7512 |
| 152 | -5.9785 | -5.9634 | -5.9621 | -5.9532 | -5.9414 | -5.9260 | -5.9182 | -5.8887 | -5.8530 | -5.8101 |
| 182 | -6.0921 | -6.0704 | -6.0664 | -6.0605 | -6.0528 | -6.0490 | -6.0245 | -5.9836 | -5.9179 | -5.9134 |
| 212 | -6.1417 | -6.0977 | -6.0958 | -6.0848 | -6.0796 | -6.0731 | -6.0692 | -6.0522 | -6.0500 | -6.0125 |
| 242 | -6.1651 | -6.1336 | -6.1262 | -6.1254 | -6.1154 | -6.1131 | -6.0940 | -6.0818 | -6.0647 | -6.0355 |
| 272 | -6.1562 | -6.1551 | -6.1541 | -6.1528 | -6.1526 | -6.1468 | -6.1425 | -6.1357 | -6.1309 | -6.1265 |
| 302 | -6.1800 | -6.1779 | -6.1666 | -6.1590 | -6.1556 | -6.1555 | -6.1500 | -6.1482 | -6.1473 | -6.0973 |
| 332 | -6.1926 | -6.1913 | -6.1670 | -6.1611 | -6.1589 | -6.1507 | -6.1498 | -6.1460 | -6.1403 | -6.1159 |
| 362 | -6.1931 | -6.1851 | -6.1746 | -6.1739 | -6.1737 | -6.1660 | -6.1633 | -6.1521 | -6.1294 | -6.1233 |
| 392 | -6.2029 | -6.1962 | -6.1917 | -6.1848 | -6.1828 | -6.1820 | -6.1757 | -6.1620 | -6.1611 | -6.1528 |
| 422 | -6.2061 | -6.1990 | -6.1968 | -6.1955 | -6.1880 | -6.1820 | -6.1698 | -6.1698 | -6.1689 | -6.1575 |
| DMRG Energy: -6.2256 | | | | | | | | | | |

**Table S21** EP ansatz with U/t = 2, VQE Energies and DMRG Energy for lattice 1x8

| Num Parameters | VQE 1 | VQE 2 | VQE 3 | VQE 4 | VQE 5 | VQE 6 | VQE 7 | VQE 8 | VQE 9 | VQE 10 |
|---|---|---|---|---|---|---|---|---|---|---|
| 70 | -5.5482 | -5.5482 | -5.5482 | -5.5482 | -5.5482 | -5.5482 | -5.5482 | -5.5482 | -5.5482 | -5.5482 |
| 104 | -6.2386 | -6.2386 | -6.2386 | -6.1626 | -6.1613 | -6.1500 | -6.1481 | -6.0905 | -6.0601 | -5.9369 |
| 138 | -6.5191 | -6.5100 | -6.5001 | -6.4995 | -6.4847 | -6.4834 | -6.4830 | -6.4676 | -6.4399 | -6.4392 |
| 172 | -6.6663 | -6.6480 | -6.6362 | -6.6249 | -6.6191 | -6.6181 | -6.6116 | -6.5974 | -6.5902 | -6.5739 |
| 206 | -6.7641 | -6.7621 | -6.7479 | -6.7398 | -6.7314 | -6.7083 | -6.7033 | -6.7025 | -6.6930 | -6.6810 |
| 240 | -6.8175 | -6.8135 | -6.8109 | -6.8085 | -6.8034 | -6.8030 | -6.7937 | -6.7878 | -6.7635 | -6.7535 |
| 274 | -6.8704 | -6.8401 | -6.8337 | -6.8250 | -6.8196 | -6.8165 | -6.8153 | -6.8142 | -6.8018 | -6.7966 |
| 308 | -6.9114 | -6.8920 | -6.8898 | -6.8889 | -6.8878 | -6.8751 | -6.8442 | -6.8275 | -6.8053 | -6.7919 |
| 342 | -6.8996 | -6.8953 | -6.8701 | -6.8607 | -6.8596 | -6.8473 | -6.8418 | -6.8406 | -6.8375 | -6.7970 |
| 376 | -6.9199 | -6.9124 | -6.9095 | -6.9070 | -6.8997 | -6.8853 | -6.8851 | -6.8718 | -6.8677 | -6.8636 |
| 410 | -6.9140 | -6.9094 | -6.9093 | -6.9068 | -6.9042 | -6.8998 | -6.8983 | -6.8935 | -6.8846 | -6.8831 |
| 444 | -6.9303 | -6.9261 | -6.9225 | -6.9216 | -6.9195 | -6.9146 | -6.9051 | -6.9015 | -6.8886 | -6.8876 |
| 478 | -6.9321 | -6.9249 | -6.9199 | -6.9182 | -6.9156 | -6.9073 | -6.9027 | -6.8890 | -6.8853 | -6.8837 |
| DMRG Energy: -6.9712 | | | | | | | | | | |

**Table S22** EP ansatz with U/t = 2, VQE Energies and DMRG Energy for lattice 1x9

| Num Parameters | VQE 1 | VQE 2 | VQE 3 | VQE 4 | VQE 5 | VQE 6 | VQE 7 | VQE 8 | VQE 9 | VQE 10 |
|---|---|---|---|---|---|---|---|---|---|---|
| 78 | -6.2135 | -6.2135 | -6.2135 | -6.2135 | -6.2135 | -6.2135 | -6.2135 | -6.2135 | -6.2135 | -6.2135 |
| 116 | -6.9067 | -6.9016 | -6.8953 | -6.8953 | -6.8953 | -6.8953 | -6.8946 | -6.8759 | -6.8759 | -6.7332 |
| 154 | -7.3431 | -7.3126 | -7.3051 | -7.3013 | -7.2928 | -7.2691 | -7.2354 | -7.2273 | -7.2043 | -7.1752 |
| 192 | -7.5545 | -7.4882 | -7.4740 | -7.4698 | -7.4599 | -7.4333 | -7.4290 | -7.4057 | -7.3786 | -7.3639 |
| 230 | -7.6568 | -7.6467 | -7.6382 | -7.6289 | -7.6174 | -7.6086 | -7.6080 | -7.5515 | -7.5396 | -7.5379 |
| 268 | -7.6987 | -7.6919 | -7.6882 | -7.6682 | -7.6678 | -7.6559 | -7.6554 | -7.6234 | -7.6053 | -7.6048 |
| 306 | -7.7293 | -7.7267 | -7.7260 | -7.7168 | -7.7163 | -7.6995 | -7.6792 | -7.6676 | -7.6585 | -7.6354 |
| 344 | -7.7830 | -7.7748 | -7.7569 | -7.7519 | -7.7446 | -7.7433 | -7.6984 | -7.6938 | -7.6763 | -7.6683 |
| 382 | -7.7907 | -7.7705 | -7.7428 | -7.7421 | -7.7231 | -7.7161 | -7.7138 | -7.7035 | -7.6959 | -7.6792 |
| 420 | -7.8527 | -7.7901 | -7.7879 | -7.7713 | -7.7644 | -7.7591 | -7.7482 | -7.7347 | -7.7112 | -7.7058 |
| 458 | -7.8091 | -7.8051 | -7.8005 | -7.7924 | -7.7849 | -7.7824 | -7.7745 | -7.7662 | -7.7522 | -7.7128 |
| 496 | -7.8421 | -7.8237 | -7.8102 | -7.7959 | -7.7957 | -7.7896 | -7.7875 | -7.7777 | -7.7550 | -7.7527 |
| 534 | -7.8323 | -7.8244 | -7.8189 | -7.8096 | -7.7979 | -7.7815 | -7.7749 | -7.7705 | -7.7659 | -7.7237 |
| DMRG Energy: -7.9087 | | | | | | | | | | |

**Table S23** EP ansatz with U/t = 2, VQE Energies and DMRG Energy for lattice 1x10

| Num Parameters | VQE 1 | VQE 2 | VQE 3 | VQE 4 | VQE 5 | VQE 6 | VQE 7 | VQE 8 | VQE 9 | VQE 10 |
|---|---|---|---|---|---|---|---|---|---|---|
| 86 | -6.8787 | -6.8787 | -6.8787 | -6.8787 | -6.8787 | -6.8787 | -6.8787 | -6.8787 | -6.8787 | -6.8787 |
| 128 | -7.7320 | -7.6756 | -7.6503 | -7.6503 | -7.6410 | -7.6151 | -7.5774 | -7.5175 | -7.4999 | -7.3874 |
| 170 | -8.0295 | -8.0250 | -8.0196 | -8.0130 | -8.0078 | -8.0065 | -7.9989 | -7.9829 | -7.9768 | -7.9726 |
| 212 | -8.2320 | -8.2239 | -8.2115 | -8.2037 | -8.2010 | -8.1983 | -8.1746 | -8.1743 | -8.1426 | -8.0934 |
| 254 | -8.3740 | -8.3637 | -8.3511 | -8.3449 | -8.3356 | -8.3248 | -8.3039 | -8.2855 | -8.2830 | -8.2158 |
| 296 | -8.4505 | -8.4178 | -8.4099 | -8.4006 | -8.3965 | -8.3912 | -8.3866 | -8.3743 | -8.3674 | -8.3403 |
| 338 | -8.5020 | -8.4733 | -8.4655 | -8.4599 | -8.4591 | -8.4547 | -8.4526 | -8.4488 | -8.4387 | -8.4273 |
| 380 | -8.5110 | -8.5044 | -8.5039 | -8.5021 | -8.4978 | -8.4961 | -8.4710 | -8.4626 | -8.4520 | -8.4475 |
| 422 | -8.5489 | -8.5246 | -8.5117 | -8.5116 | -8.5049 | -8.5037 | -8.5029 | -8.4992 | -8.4862 | -8.4751 |
| 464 | -8.5438 | -8.5400 | -8.5253 | -8.5233 | -8.5145 | -8.5142 | -8.5117 | -8.5084 | -8.5003 | -8.4927 |
| 506 | -8.5576 | -8.5504 | -8.5499 | -8.5400 | -8.5383 | -8.5337 | -8.5313 | -8.5304 | -8.5302 | -8.5116 |
| 548 | -8.5778 | -8.5715 | -8.5565 | -8.5498 | -8.5421 | -8.5371 | -8.5361 | -8.5353 | -8.5290 | -8.5233 |
| 590 | -8.5706 | -8.5706 | -8.5696 | -8.5694 | -8.5679 | -8.5626 | -8.5617 | -8.5569 | -8.5557 | -8.5348 |
| DMRG Energy: -8.6706 | | | | | | | | | | |

**Table S24** EP ansatz with U/t = 2, VQE Energies and DMRG Energy for lattice 1x11

| Num Parameters | VQE 1 | VQE 2 | VQE 3 | VQE 4 | VQE 5 | VQE 6 | VQE 7 | VQE 8 | VQE 9 | VQE 10 |
|---|---|---|---|---|---|---|---|---|---|---|
| 94 | -7.5440 | -7.5440 | -7.5440 | -7.5440 | -7.5440 | -7.5440 | -7.5440 | -7.5440 | -7.5440 | -7.5440 |
| 140 | -8.3941 | -8.3941 | -8.3827 | -8.3827 | -8.3827 | -8.3827 | -8.3635 | -8.2912 | -8.2732 | -8.1038 |
| 186 | -8.8797 | -8.8396 | -8.8078 | -8.7975 | -8.7972 | -8.7836 | -8.7705 | -8.7615 | -8.7514 | -8.7502 |
| 232 | -9.1368 | -9.1211 | -9.0980 | -9.0101 | -9.0003 | -8.9743 | -8.9560 | -8.9358 | -8.9355 | -8.8888 |
| 278 | -9.2443 | -9.2309 | -9.2243 | -9.2181 | -9.1652 | -9.1351 | -9.1325 | -9.1165 | -9.0829 | -9.0658 |
| 324 | -9.2933 | -9.2687 | -9.2551 | -9.2448 | -9.2421 | -9.2328 | -9.2255 | -9.2223 | -9.2158 | -9.1944 |
| 370 | -9.3239 | -9.3228 | -9.3212 | -9.3103 | -9.3079 | -9.2970 | -9.2929 | -9.2879 | -9.2741 | -9.2613 |
| 416 | -9.4136 | -9.3715 | -9.3699 | -9.3643 | -9.3629 | -9.3521 | -9.3398 | -9.3055 | -9.2972 | -9.2872 |
| 462 | -9.3994 | -9.3899 | -9.3859 | -9.3847 | -9.3702 | -9.3702 | -9.3605 | -9.3471 | -9.3345 | -9.3184 |
| 508 | -9.3883 | -9.3877 | -9.3786 | -9.3783 | -9.3671 | -9.3644 | -9.3622 | -9.3554 | -9.3490 | -9.3168 |
| 554 | -9.4730 | -9.4475 | -9.4428 | -9.4371 | -9.4317 | -9.4303 | -9.4254 | -9.4126 | -9.4085 | -9.3958 |
| 600 | -9.4623 | -9.4537 | -9.4529 | -9.4459 | -9.4417 | -9.4403 | -9.4395 | -9.4143 | -9.4138 | -9.3985 |
| 646 | -9.5290 | -9.4866 | -9.4846 | -9.4782 | -9.4627 | -9.4582 | -9.4538 | -9.4506 | -9.4430 | -9.4421 |
| DMRG Energy: -9.5938 | | | | | | | | | | |

**Table S25** EP ansatz with U/t = 2, VQE Energies and DMRG Energy for lattice 1x12

| Num Parameters | VQE 1 | VQE 2 | VQE 3 | VQE 4 | VQE 5 | VQE 6 | VQE 7 | VQE 8 | VQE 9 | VQE 10 |
|---|---|---|---|---|---|---|---|---|---|---|
| 30 | -2.0000 | -2.0000 | -2.0000 | -2.0000 | -2.0000 | -2.0000 | -2.0000 | -2.0000 | -2.0000 | -2.0000 |
| 44 | -2.6610 | -2.6610 | -2.6610 | -2.6610 | -2.6610 | -2.6610 | -2.6610 | -2.6610 | -2.5088 | -2.5088 |
| 58 | -2.6942 | -2.6886 | -2.6886 | -2.6886 | -2.6886 | -2.6886 | -2.6853 | -2.6610 | -2.6610 | -2.6610 |
| 72 | -2.7576 | -2.7467 | -2.7401 | -2.7401 | -2.7397 | -2.7385 | -2.7366 | -2.7366 | -2.7329 | -2.7314 |
| 86 | -2.7710 | -2.7650 | -2.7641 | -2.7612 | -2.7582 | -2.7529 | -2.7526 | -2.7475 | -2.7452 | -2.6789 |
| 100 | -2.8284 | -2.7861 | -2.7858 | -2.7856 | -2.7786 | -2.7770 | -2.7740 | -2.7730 | -2.7711 | -2.7563 |
| 114 | -2.8284 | -2.8284 | -2.8098 | -2.8023 | -2.8000 | -2.7991 | -2.7973 | -2.7952 | -2.7911 | -2.7888 |
| 128 | -2.8284 | -2.8284 | -2.8234 | -2.8218 | -2.8184 | -2.8180 | -2.8168 | -2.8165 | -2.8164 | -2.8149 |
| 142 | -2.8279 | -2.8279 | -2.8278 | -2.8277 | -2.8276 | -2.8270 | -2.8266 | -2.8265 | -2.8263 | -2.8241 |
| 156 | -2.8284 | -2.8284 | -2.8284 | -2.8284 | -2.8283 | -2.8283 | -2.8283 | -2.8283 | -2.8282 | -2.8277 |
| 170 | -2.8284 | -2.8284 | -2.8284 | -2.8284 | -2.8284 | -2.8284 | -2.8283 | -2.8283 | -2.8282 | -2.8263 |
| 184 | -2.8284 | -2.8284 | -2.8284 | -2.8284 | -2.8284 | -2.8284 | -2.8284 | -2.8284 | -2.8284 | -2.8284 |
| 198 | -2.8284 | -2.8284 | -2.8284 | -2.8284 | -2.8284 | -2.8284 | -2.8284 | -2.8284 | -2.8284 | -2.8284 |
| DMRG Energy: -2.8284 | | | | | | | | | | |

**Table S26** EP ansatz with U/t = 2, VQE Energies and DMRG Energy for lattice 2x2

| Num Parameters | VQE 1 | VQE 2 | VQE 3 | VQE 4 | VQE 5 | VQE 6 | VQE 7 | VQE 8 | VQE 9 | VQE 10 |
|---|---|---|---|---|---|---|---|---|---|---|
| 46 | -3.0801 | -3.0801 | -3.0801 | -3.0801 | -3.0801 | -3.0801 | -3.0801 | -3.0801 | -3.0801 | -3.0801 |
| 68 | -4.1867 | -4.1867 | -4.1867 | -4.1867 | -4.1867 | -4.1867 | -4.1867 | -3.9478 | -3.8557 | -3.6554 |
| 90 | -4.7814 | -4.7215 | -4.7215 | -4.6569 | -4.2940 | -4.2940 | -4.2777 | -4.2723 | -4.2673 | -4.2566 |
| 112 | -4.9469 | -4.9445 | -4.9425 | -4.9222 | -4.9207 | -4.9131 | -4.8984 | -4.8758 | -4.7215 | -4.7215 |
| 134 | -5.0422 | -5.0123 | -5.0079 | -5.0070 | -5.0001 | -4.9934 | -4.9900 | -4.9725 | -4.9701 | -4.9483 |
| 156 | -5.0699 | -5.0624 | -5.0470 | -5.0396 | -5.0383 | -5.0383 | -5.0363 | -4.9856 | -4.9822 | -4.9789 |
| 178 | -5.0726 | -5.0704 | -5.0686 | -5.0672 | -5.0658 | -5.0586 | -5.0559 | -5.0506 | -5.0415 | -5.0216 |
| 200 | -5.0955 | -5.0862 | -5.0801 | -5.0794 | -5.0793 | -5.0768 | -5.0737 | -5.0725 | -5.0707 | -5.0623 |
| 222 | -5.0879 | -5.0850 | -5.0848 | -5.0839 | -5.0838 | -5.0835 | -5.0819 | -5.0790 | -5.0776 | -5.0613 |
| 244 | -5.0953 | -5.0943 | -5.0937 | -5.0907 | -5.0902 | -5.0880 | -5.0864 | -5.0858 | -5.0818 | -5.0789 |
| 266 | -5.0995 | -5.0960 | -5.0946 | -5.0942 | -5.0934 | -5.0898 | -5.0895 | -5.0888 | -5.0816 | -5.0796 |
| 288 | -5.1005 | -5.0997 | -5.0997 | -5.0992 | -5.0984 | -5.0980 | -5.0968 | -5.0941 | -5.0928 | -5.0833 |
| 310 | -5.1098 | -5.1061 | -5.1046 | -5.1019 | -5.1017 | -5.1000 | -5.0998 | -5.0993 | -5.0992 | -5.0952 |
| DMRG Energy: -5.1592 | | | | | | | | | | |

**Table S27** EP ansatz with U/t = 2, VQE Energies and DMRG Energy for lattice 2x3

| Num Parameters | VQE 1 | VQE 2 | VQE 3 | VQE 4 | VQE 5 | VQE 6 | VQE 7 | VQE 8 | VQE 9 | VQE 10 |
|---|---|---|---|---|---|---|---|---|---|---|
| 70 | -4.6201 | -4.6201 | -4.6201 | -4.6201 | -4.6201 | -4.6201 | -4.6201 | -4.6201 | -4.6201 | -4.6201 |
| 104 | -6.3136 | -6.3136 | -6.3136 | -6.3136 | -6.3136 | -6.3136 | -6.3136 | -6.0877 | -6.0877 | -5.8843 |
| 138 | -7.1213 | -7.1213 | -7.0753 | -7.0373 | -6.9950 | -6.9785 | -6.8155 | -6.8076 | -6.7540 | -6.5671 |
| 172 | -7.4877 | -7.4831 | -7.4381 | -7.4152 | -7.3810 | -7.3709 | -7.3703 | -7.3652 | -7.3360 | -7.1471 |
| 206 | -7.5920 | -7.5664 | -7.5634 | -7.5504 | -7.5470 | -7.5370 | -7.4692 | -7.4667 | -7.4652 | -7.2962 |
| 240 | -7.6916 | -7.6822 | -7.6791 | -7.6365 | -7.6320 | -7.6309 | -7.6103 | -7.5973 | -7.4730 | -7.3349 |
| 274 | -7.7258 | -7.7177 | -7.7080 | -7.6980 | -7.6174 | -7.6106 | -7.5905 | -7.5883 | -7.5389 | -7.3460 |
| 308 | -7.7669 | -7.7500 | -7.7489 | -7.7480 | -7.7365 | -7.7233 | -7.7222 | -7.6814 | -7.6151 | -7.6141 |
| 342 | -7.7780 | -7.7583 | -7.7539 | -7.7410 | -7.7377 | -7.7167 | -7.6882 | -7.6769 | -7.5909 | -7.4881 |
| 376 | -7.7867 | -7.7824 | -7.7694 | -7.7645 | -7.7538 | -7.7532 | -7.7455 | -7.7360 | -7.7054 | -7.6912 |
| 410 | -7.7898 | -7.7854 | -7.7826 | -7.7718 | -7.7653 | -7.7622 | -7.7532 | -7.7247 | -7.7070 | -7.6762 |
| 444 | -7.8173 | -7.7996 | -7.7956 | -7.7844 | -7.7834 | -7.7820 | -7.7624 | -7.7582 | -7.7511 | -7.7220 |
| 478 | -7.8104 | -7.8082 | -7.8060 | -7.7979 | -7.7890 | -7.7833 | -7.7820 | -7.7751 | -7.7692 | -7.7231 |
| DMRG Energy: -7.9865 | | | | | | | | | | |

**Table S28** EP ansatz with U/t = 2, VQE Energies and DMRG Energy for lattice 3x3

# S3 NP ansatz, $U/t = 8$

| Num Parameters | VQE 1 | VQE 2 | VQE 3 | VQE 4 | VQE 5 | VQE 6 | VQE 7 | VQE 8 | VQE 9 | VQE 10 |
|---|---|---|---|---|---|---|---|---|---|---|
| 12 | 0.0000 | 0.0000 | 0.0000 | 0.0000 | 0.0000 | 0.0000 | 0.0000 | 0.0000 | 0.0000 | 0.0000 |
| 20 | -0.4721 | -0.4721 | -0.4721 | -0.4721 | -0.4721 | -0.4721 | -0.4721 | -0.4721 | -0.2361 | 0.0000 |
| 28 | -0.4721 | -0.4721 | -0.4721 | -0.4721 | -0.4721 | -0.4721 | -0.4721 | -0.4721 | -0.4721 | -0.4721 |
| 36 | -0.4721 | -0.4721 | -0.4721 | -0.4721 | -0.4721 | -0.4721 | -0.4721 | -0.4721 | -0.4721 | -0.4721 |
| 44 | -0.4721 | -0.4721 | -0.4721 | -0.4721 | -0.4721 | -0.4721 | -0.4721 | -0.4721 | -0.4721 | -0.4721 |
| 52 | -0.4721 | -0.4721 | -0.4721 | -0.4721 | -0.4721 | -0.4721 | -0.4721 | -0.4721 | -0.4721 | -0.4721 |
| 60 | -0.4721 | -0.4721 | -0.4721 | -0.4721 | -0.4721 | -0.4721 | -0.4721 | -0.4721 | -0.4721 | -0.4721 |
| 68 | -0.4721 | -0.4721 | -0.4721 | -0.4721 | -0.4721 | -0.4721 | -0.4721 | -0.4721 | -0.4721 | -0.4721 |
| 76 | -0.4721 | -0.4721 | -0.4721 | -0.4721 | -0.4721 | -0.4721 | -0.4721 | -0.4721 | -0.4721 | -0.4721 |
| 84 | -0.4721 | -0.4721 | -0.4721 | -0.4721 | -0.4721 | -0.4721 | -0.4721 | -0.4721 | -0.4721 | -0.4721 |
| 92 | -0.4721 | -0.4721 | -0.4721 | -0.4721 | -0.4721 | -0.4721 | -0.4721 | -0.4721 | -0.4721 | -0.4721 |
| 100 | -0.4721 | -0.4721 | -0.4721 | -0.4721 | -0.4721 | -0.4721 | -0.4721 | -0.4721 | -0.4721 | -0.4721 |
| 108 | -0.4721 | -0.4721 | -0.4721 | -0.4721 | -0.4721 | -0.4721 | -0.4721 | -0.4721 | -0.4721 | -0.4721 |
| DMRG Energy: -0.4721 | | | | | | | | | | |

**Table S29** NP ansatz with U/t = 8, VQE Energies and DMRG Energy for lattice 1x2

| Num Parameters | VQE 1 | VQE 2 | VQE 3 | VQE 4 | VQE 5 | VQE 6 | VQE 7 | VQE 8 | VQE 9 | VQE 10 |
|---|---|---|---|---|---|---|---|---|---|---|
| 20 | -0.1231 | -0.1231 | -0.1231 | -0.1231 | -0.0000 | 0.0000 | 0.0000 | 0.0000 | 0.0000 | 0.0000 |
| 34 | -0.6936 | -0.6933 | -0.6912 | -0.6908 | -0.6897 | -0.6891 | -0.6447 | -0.6422 | -0.6271 | -0.5697 |
| 48 | -0.7077 | -0.7077 | -0.7077 | -0.7077 | -0.7077 | -0.7077 | -0.7077 | -0.7077 | -0.7074 | -0.7059 |
| 62 | -0.7077 | -0.7077 | -0.7077 | -0.7077 | -0.7077 | -0.7077 | -0.7077 | -0.7077 | -0.7077 | -0.7077 |
| 76 | -0.7077 | -0.7077 | -0.7077 | -0.7077 | -0.7077 | -0.7077 | -0.7077 | -0.7077 | -0.7077 | -0.7077 |
| 90 | -0.7077 | -0.7077 | -0.7077 | -0.7077 | -0.7077 | -0.7077 | -0.7077 | -0.7077 | -0.7077 | -0.7077 |
| 104 | -0.7077 | -0.7077 | -0.7077 | -0.7077 | -0.7077 | -0.7077 | -0.7077 | -0.7077 | -0.7077 | -0.7077 |
| 118 | -0.7077 | -0.7077 | -0.7077 | -0.7077 | -0.7077 | -0.7077 | -0.7077 | -0.7077 | -0.7077 | -0.7077 |
| 132 | -0.7077 | -0.7077 | -0.7077 | -0.7077 | -0.7077 | -0.7077 | -0.7077 | -0.7077 | -0.7077 | -0.7077 |
| 146 | -0.7077 | -0.7077 | -0.7077 | -0.7077 | -0.7077 | -0.7077 | -0.7077 | -0.7077 | -0.7077 | -0.7077 |
| 160 | -0.7077 | -0.7077 | -0.7077 | -0.7077 | -0.7077 | -0.7077 | -0.7077 | -0.7077 | -0.7077 | -0.7077 |
| 174 | -0.7077 | -0.7077 | -0.7077 | -0.7077 | -0.7077 | -0.7077 | -0.7077 | -0.7077 | -0.7077 | -0.7077 |
| 188 | -0.7077 | -0.7077 | -0.7077 | -0.7077 | -0.7077 | -0.7077 | -0.7077 | -0.7077 | -0.7077 | -0.7077 |
| DMRG Energy: -0.7077 | | | | | | | | | | |

**Table S30** NP ansatz with U/t = 8, VQE Energies and DMRG Energy for lattice 1x3

| Num Parameters | VQE 1 | VQE 2 | VQE 3 | VQE 4 | VQE 5 | VQE 6 | VQE 7 | VQE 8 | VQE 9 | VQE 10 |
|---|---|---|---|---|---|---|---|---|---|---|
| 28 | -0.2394 | -0.2394 | -0.2394 | -0.2394 | -0.1231 | -0.1231 | -0.1231 | 0.0000 | 0.0000 | 0.0000 |
| 48 | -1.0483 | -1.0483 | -1.0465 | -1.0462 | -1.0462 | -1.0446 | -0.9279 | -0.9101 | -0.8809 | -0.6185 |
| 68 | -1.1028 | -1.0988 | -1.0941 | -1.0924 | -1.0918 | -1.0895 | -1.0864 | -1.0859 | -1.0747 | -1.0660 |
| 88 | -1.1133 | -1.1127 | -1.1087 | -1.1085 | -1.1084 | -1.1084 | -1.1080 | -1.1077 | -1.1064 | -1.1061 |
| 108 | -1.1164 | -1.1163 | -1.1162 | -1.1161 | -1.1152 | -1.1140 | -1.1128 | -1.1128 | -1.1099 | -1.1091 |
| 128 | -1.1169 | -1.1167 | -1.1159 | -1.1159 | -1.1154 | -1.1151 | -1.1149 | -1.1117 | -1.1100 | -1.1072 |
| 148 | -1.1167 | -1.1163 | -1.1163 | -1.1162 | -1.1161 | -1.1156 | -1.1154 | -1.1154 | -1.1151 | -1.1110 |
| 168 | -1.1170 | -1.1168 | -1.1167 | -1.1167 | -1.1166 | -1.1165 | -1.1163 | -1.1161 | -1.1157 | -1.1155 |
| 188 | -1.1171 | -1.1171 | -1.1171 | -1.1170 | -1.1170 | -1.1169 | -1.1169 | -1.1169 | -1.1167 | -1.1160 |
| 208 | -1.1172 | -1.1172 | -1.1172 | -1.1171 | -1.1171 | -1.1170 | -1.1170 | -1.1169 | -1.1167 | -1.1162 |
| 228 | -1.1172 | -1.1172 | -1.1172 | -1.1171 | -1.1171 | -1.1171 | -1.1171 | -1.1171 | -1.1171 | -1.1169 |
| 248 | -1.1172 | -1.1172 | -1.1172 | -1.1172 | -1.1172 | -1.1172 | -1.1172 | -1.1172 | -1.1172 | -1.1171 |
| 268 | -1.1172 | -1.1172 | -1.1172 | -1.1172 | -1.1172 | -1.1172 | -1.1172 | -1.1172 | -1.1172 | -1.1172 |
| DMRG Energy: -1.1172 | | | | | | | | | | |

**Table S31** NP ansatz with U/t = 8, VQE Energies and DMRG Energy for lattice 1x4

| Num Parameters | VQE 1 | VQE 2 | VQE 3 | VQE 4 | VQE 5 | VQE 6 | VQE 7 | VQE 8 | VQE 9 | VQE 10 |
|---|---|---|---|---|---|---|---|---|---|---|
| 36 | -0.3661 | -0.3660 | -0.2500 | -0.2500 | -0.2500 | -0.1231 | -0.1231 | 0.0000 | 0.0000 | 0.0000 |
| 62 | -1.2937 | -1.2874 | -1.2596 | -1.2406 | -1.2346 | -1.2116 | -1.1957 | -1.1716 | -1.1661 | -1.1628 |
| 88 | -1.3489 | -1.3471 | -1.3459 | -1.3454 | -1.3441 | -1.3387 | -1.3360 | -1.3323 | -1.3309 | -1.3205 |
| 114 | -1.3638 | -1.3612 | -1.3576 | -1.3565 | -1.3558 | -1.3498 | -1.3480 | -1.3478 | -1.3472 | -1.3445 |
| 140 | -1.3666 | -1.3653 | -1.3645 | -1.3633 | -1.3627 | -1.3594 | -1.3588 | -1.3587 | -1.3523 | -1.3509 |
| 166 | -1.3696 | -1.3686 | -1.3677 | -1.3664 | -1.3653 | -1.3648 | -1.3618 | -1.3602 | -1.3583 | -1.3493 |
| 192 | -1.3720 | -1.3715 | -1.3706 | -1.3693 | -1.3693 | -1.3680 | -1.3643 | -1.3621 | -1.3607 | -1.3560 |
| 218 | -1.3738 | -1.3733 | -1.3728 | -1.3720 | -1.3705 | -1.3701 | -1.3687 | -1.3677 | -1.3670 | -1.3646 |
| 244 | -1.3774 | -1.3751 | -1.3747 | -1.3722 | -1.3718 | -1.3709 | -1.3706 | -1.3698 | -1.3697 | -1.3648 |
| 270 | -1.3765 | -1.3749 | -1.3747 | -1.3746 | -1.3744 | -1.3716 | -1.3706 | -1.3706 | -1.3686 | -1.3650 |
| 296 | -1.3765 | -1.3760 | -1.3744 | -1.3736 | -1.3729 | -1.3724 | -1.3718 | -1.3715 | -1.3713 | -1.3699 |
| 322 | -1.3761 | -1.3757 | -1.3756 | -1.3756 | -1.3756 | -1.3744 | -1.3732 | -1.3700 | -1.3697 | -1.3686 |
| 348 | -1.3778 | -1.3773 | -1.3769 | -1.3767 | -1.3763 | -1.3757 | -1.3750 | -1.3734 | -1.3713 | -1.3713 |
| DMRG Energy: -1.3826 | | | | | | | | | | |

**Table S32** NP ansatz with U/t = 8, VQE Energies and DMRG Energy for lattice 1x5

| Num Parameters | VQE 1 | VQE 2 | VQE 3 | VQE 4 | VQE 5 | VQE 6 | VQE 7 | VQE 8 | VQE 9 | VQE 10 |
|---|---|---|---|---|---|---|---|---|---|---|
| 44 | -0.4821 | -0.4821 | -0.2500 | -0.2463 | -0.2462 | -0.2462 | -0.2462 | -0.2462 | -0.2462 | -0.1231 |
| 76 | -1.5823 | -1.5760 | -1.5246 | -1.5213 | -1.5099 | -1.5054 | -1.4991 | -1.4872 | -1.4616 | -1.3121 |
| 108 | -1.6984 | -1.6969 | -1.6949 | -1.6934 | -1.6873 | -1.6809 | -1.6720 | -1.6694 | -1.6620 | -1.6341 |
| 140 | -1.7267 | -1.7260 | -1.7225 | -1.7196 | -1.7082 | -1.7059 | -1.6965 | -1.6955 | -1.6891 | -1.6859 |
| 172 | -1.7476 | -1.7296 | -1.7282 | -1.7259 | -1.7228 | -1.7217 | -1.7177 | -1.7141 | -1.7085 | -1.7001 |
| 204 | -1.7504 | -1.7410 | -1.7370 | -1.7328 | -1.7279 | -1.7263 | -1.7240 | -1.7165 | -1.7159 | -1.7100 |
| 236 | -1.7495 | -1.7471 | -1.7443 | -1.7423 | -1.7379 | -1.7379 | -1.7356 | -1.7324 | -1.7299 | -1.7266 |
| 268 | -1.7453 | -1.7436 | -1.7429 | -1.7407 | -1.7396 | -1.7386 | -1.7375 | -1.7324 | -1.7185 | -1.7119 |
| 300 | -1.7518 | -1.7470 | -1.7377 | -1.7328 | -1.7327 | -1.7314 | -1.7270 | -1.7220 | -1.7120 | -1.7114 |
| 332 | -1.7463 | -1.7445 | -1.7416 | -1.7377 | -1.7297 | -1.7217 | -1.7196 | -1.7180 | -1.7176 | -1.6987 |
| 364 | -1.7536 | -1.7501 | -1.7405 | -1.7398 | -1.7395 | -1.7345 | -1.7308 | -1.7252 | -1.7226 | -1.7157 |
| 396 | -1.7614 | -1.7544 | -1.7520 | -1.7482 | -1.7442 | -1.7426 | -1.7380 | -1.7265 | -1.7243 | -1.7210 |
| 428 | -1.7519 | -1.7487 | -1.7486 | -1.7469 | -1.7432 | -1.7385 | -1.7373 | -1.7329 | -1.7175 | -1.7105 |
| DMRG Energy: -1.7681 | | | | | | | | | | |

**Table S33** NP ansatz with U/t = 8, VQE Energies and DMRG Energy for lattice 1x6

| Num Parameters | VQE 1 | VQE 2 | VQE 3 | VQE 4 | VQE 5 | VQE 6 | VQE 7 | VQE 8 | VQE 9 | VQE 10 |
|---|---|---|---|---|---|---|---|---|---|---|
| 52 | -0.6086 | -0.6086 | -0.6019 | -0.4892 | -0.4853 | -0.3731 | -0.3731 | -0.3731 | -0.3731 | -0.3661 |
| 90 | -1.8825 | -1.8573 | -1.8567 | -1.8547 | -1.8514 | -1.8484 | -1.8033 | -1.7883 | -1.7659 | -1.6880 |
| 128 | -1.9754 | -1.9748 | -1.9734 | -1.9689 | -1.9574 | -1.9571 | -1.9548 | -1.9463 | -1.9122 | -1.9054 |
| 166 | -1.9992 | -1.9953 | -1.9914 | -1.9858 | -1.9832 | -1.9743 | -1.9684 | -1.9607 | -1.9465 | -1.9378 |
| 204 | -2.0120 | -2.0054 | -2.0009 | -1.9995 | -1.9951 | -1.9915 | -1.9891 | -1.9820 | -1.9771 | -1.9769 |
| 242 | -2.0134 | -2.0134 | -2.0126 | -2.0108 | -2.0097 | -2.0081 | -2.0077 | -2.0062 | -2.0043 | -2.0029 |
| 280 | -2.0198 | -2.0178 | -2.0176 | -2.0155 | -2.0139 | -2.0135 | -2.0132 | -2.0106 | -2.0065 | -2.0009 |
| 318 | -2.0195 | -2.0168 | -2.0162 | -2.0159 | -2.0148 | -2.0137 | -2.0125 | -2.0115 | -2.0101 | -2.0097 |
| 356 | -2.0268 | -2.0202 | -2.0197 | -2.0158 | -2.0156 | -2.0141 | -2.0138 | -2.0103 | -2.0091 | -2.0054 |
| 394 | -2.0219 | -2.0196 | -2.0190 | -2.0170 | -2.0159 | -2.0152 | -2.0145 | -2.0142 | -2.0082 | -2.0067 |
| 432 | -2.0272 | -2.0239 | -2.0234 | -2.0226 | -2.0195 | -2.0180 | -2.0172 | -2.0160 | -2.0143 | -2.0004 |
| 470 | -2.0295 | -2.0271 | -2.0269 | -2.0257 | -2.0227 | -2.0225 | -2.0224 | -2.0215 | -2.0199 | -2.0199 |
| 508 | -2.0268 | -2.0262 | -2.0255 | -2.0255 | -2.0243 | -2.0226 | -2.0222 | -2.0218 | -2.0216 | -2.0186 |
| DMRG Energy: -2.0482 | | | | | | | | | | |

**Table S34** NP ansatz with U/t = 8, VQE Energies and DMRG Energy for lattice 1x7

| Num Parameters | VQE 1 | VQE 2 | VQE 3 | VQE 4 | VQE 5 | VQE 6 | VQE 7 | VQE 8 | VQE 9 | VQE 10 |
|---|---|---|---|---|---|---|---|---|---|---|
| 60 | -0.7246 | -0.7246 | -0.7184 | -0.7184 | -0.7182 | -0.6086 | -0.6086 | -0.6055 | -0.6052 | -0.3694 |
| 104 | -2.1791 | -2.1787 | -2.1057 | -2.0758 | -2.0721 | -2.0456 | -2.0427 | -2.0379 | -2.0336 | -2.0275 |
| 148 | -2.2879 | -2.2845 | -2.2839 | -2.2760 | -2.2751 | -2.2077 | -2.2062 | -2.2025 | -2.1915 | -2.1774 |
| 192 | -2.3317 | -2.3289 | -2.3246 | -2.3198 | -2.3193 | -2.3181 | -2.3071 | -2.3058 | -2.3005 | -2.2186 |
| 236 | -2.3544 | -2.3487 | -2.3468 | -2.3378 | -2.3362 | -2.3335 | -2.3313 | -2.3298 | -2.3291 | -2.3181 |
| 280 | -2.3482 | -2.3475 | -2.3437 | -2.3422 | -2.3412 | -2.3406 | -2.3385 | -2.3341 | -2.3283 | -2.3132 |
| 324 | -2.3628 | -2.3521 | -2.3504 | -2.3496 | -2.3489 | -2.3466 | -2.3443 | -2.3374 | -2.3307 | -2.2610 |
| 368 | -2.3725 | -2.3678 | -2.3609 | -2.3523 | -2.3508 | -2.3502 | -2.3487 | -2.3465 | -2.3421 | -2.3397 |
| 412 | -2.3783 | -2.3688 | -2.3607 | -2.3594 | -2.3562 | -2.3519 | -2.3510 | -2.3476 | -2.3439 | -2.3424 |
| 456 | -2.3771 | -2.3690 | -2.3662 | -2.3641 | -2.3636 | -2.3621 | -2.3599 | -2.3563 | -2.3556 | -2.3527 |
| 500 | -2.3764 | -2.3718 | -2.3633 | -2.3606 | -2.3597 | -2.3546 | -2.3523 | -2.3491 | -2.3413 | -2.3383 |
| 544 | -2.3809 | -2.3793 | -2.3777 | -2.3776 | -2.3679 | -2.3661 | -2.3634 | -2.3567 | -2.3554 | -2.3443 |
| 588 | -2.3882 | -2.3820 | -2.3738 | -2.3722 | -2.3669 | -2.3664 | -2.3641 | -2.3632 | -2.3595 | -2.3584 |
| DMRG Energy: -2.4208 | | | | | | | | | | |

**Table S35** NP ansatz with U/t = 8, VQE Energies and DMRG Energy for lattice 1x8

| Num Parameters | VQE 1 | VQE 2 | VQE 3 | VQE 4 | VQE 5 | VQE 6 | VQE 7 | VQE 8 | VQE 9 | VQE 10 |
|---|---|---|---|---|---|---|---|---|---|---|
| 68 | -0.8512 | -0.8382 | -0.8382 | -0.8380 | -0.7321 | -0.7248 | -0.6160 | -0.6084 | -0.4892 | -0.4853 |
| 118 | -2.4423 | -2.4233 | -2.4225 | -2.4221 | -2.4163 | -2.4102 | -2.3703 | -2.3325 | -2.1956 | -2.1343 |
| 168 | -2.5982 | -2.5979 | -2.5932 | -2.5794 | -2.5787 | -2.5484 | -2.5353 | -2.5239 | -2.5108 | -2.5008 |
| 218 | -2.6462 | -2.6368 | -2.6285 | -2.6260 | -2.6243 | -2.6211 | -2.6175 | -2.6158 | -2.6133 | -2.6101 |
| 268 | -2.6508 | -2.6453 | -2.6431 | -2.6424 | -2.6383 | -2.6353 | -2.6329 | -2.6320 | -2.6314 | -2.6277 |
| 318 | -2.6562 | -2.6497 | -2.6489 | -2.6475 | -2.6459 | -2.6420 | -2.6418 | -2.6414 | -2.6381 | -2.6224 |
| 368 | -2.6601 | -2.6569 | -2.6556 | -2.6548 | -2.6522 | -2.6516 | -2.6513 | -2.6493 | -2.6451 | -2.6418 |
| 418 | -2.6684 | -2.6608 | -2.6599 | -2.6552 | -2.6546 | -2.6522 | -2.6489 | -2.6488 | -2.6466 | -2.6406 |
| 468 | -2.6703 | -2.6642 | -2.6633 | -2.6629 | -2.6585 | -2.6579 | -2.6575 | -2.6554 | -2.6550 | -2.6530 |
| 518 | -2.6676 | -2.6673 | -2.6649 | -2.6645 | -2.6620 | -2.6618 | -2.6564 | -2.6526 | -2.6519 | -2.6422 |
| 568 | -2.6715 | -2.6695 | -2.6693 | -2.6678 | -2.6621 | -2.6602 | -2.6598 | -2.6587 | -2.6541 | -2.6488 |
| 618 | -2.6757 | -2.6734 | -2.6680 | -2.6642 | -2.6638 | -2.6631 | -2.6615 | -2.6606 | -2.6593 | -2.6474 |
| 668 | -2.6720 | -2.6706 | -2.6704 | -2.6688 | -2.6679 | -2.6674 | -2.6643 | -2.6619 | -2.6440 | -2.6392 |
| DMRG Energy: -2.7098 | | | | | | | | | | |

**Table S36** NP ansatz with U/t = 8, VQE Energies and DMRG Energy for lattice 1x9

| Num Parameters | VQE 1 | VQE 2 | VQE 3 | VQE 4 | VQE 5 | VQE 6 | VQE 7 | VQE 8 | VQE 9 | VQE 10 |
|---|---|---|---|---|---|---|---|---|---|---|
| 76 | -0.9550 | -0.9546 | -0.9546 | -0.9546 | -0.9544 | -0.9543 | -0.8481 | -0.7321 | -0.7248 | -0.7248 |
| 132 | -2.6978 | -2.6936 | -2.6922 | -2.6824 | -2.6707 | -2.6698 | -2.6582 | -2.6446 | -2.5998 | -2.5928 |
| 188 | -2.9261 | -2.9194 | -2.9072 | -2.8784 | -2.8339 | -2.8228 | -2.7941 | -2.7833 | -2.7425 | -2.7273 |
| 244 | -2.9623 | -2.9585 | -2.9582 | -2.9560 | -2.9557 | -2.9472 | -2.9435 | -2.9418 | -2.9249 | -2.9204 |
| 300 | -2.9727 | -2.9699 | -2.9698 | -2.9654 | -2.9634 | -2.9631 | -2.9597 | -2.9452 | -2.9377 | -2.9275 |
| 356 | -2.9834 | -2.9750 | -2.9732 | -2.9731 | -2.9710 | -2.9706 | -2.9696 | -2.9686 | -2.9591 | -2.9560 |
| 412 | -2.9908 | -2.9867 | -2.9811 | -2.9735 | -2.9729 | -2.9727 | -2.9667 | -2.9615 | -2.9601 | -2.9511 |
| 468 | -2.9961 | -2.9958 | -2.9862 | -2.9853 | -2.9811 | -2.9781 | -2.9721 | -2.9717 | -2.9716 | -2.9612 |
| 524 | -2.9924 | -2.9910 | -2.9905 | -2.9868 | -2.9860 | -2.9854 | -2.9823 | -2.9771 | -2.9767 | -2.9748 |
| 580 | -3.0075 | -2.9997 | -2.9972 | -2.9858 | -2.9846 | -2.9814 | -2.9773 | -2.9680 | -2.9659 | -2.9573 |
| 636 | -2.9986 | -2.9969 | -2.9963 | -2.9924 | -2.9898 | -2.9884 | -2.9855 | -2.9815 | -2.9790 | -2.9770 |
| 692 | -3.0088 | -2.9993 | -2.9976 | -2.9962 | -2.9947 | -2.9896 | -2.9870 | -2.9837 | -2.9808 | -2.9777 |
| 748 | -3.0123 | -3.0102 | -3.0076 | -3.0048 | -2.9940 | -2.9936 | -2.9890 | -2.9786 | -2.9773 | -2.9723 |
| DMRG Energy: -3.0744 | | | | | | | | | | |

**Table S37** NP ansatz with U/t = 8, VQE Energies and DMRG Energy for lattice 1x10

| Num Parameters | VQE 1 | VQE 2 | VQE 3 | VQE 4 | VQE 5 | VQE 6 | VQE 7 | VQE 8 | VQE 9 | VQE 10 |
|---|---|---|---|---|---|---|---|---|---|---|
| 84 | -1.0746 | -1.0744 | -1.0741 | -1.0739 | -1.0739 | -1.0739 | -0.9610 | -0.8586 | -0.8505 | -0.8447 |
| 146 | -2.9901 | -2.9728 | -2.9726 | -2.9692 | -2.9520 | -2.9345 | -2.8888 | -2.8315 | -2.7578 | -2.7229 |
| 208 | -3.2262 | -3.2247 | -3.2176 | -3.2148 | -3.2144 | -3.2125 | -3.2063 | -3.2028 | -3.1801 | -3.1037 |
| 270 | -3.2742 | -3.2736 | -3.2620 | -3.2563 | -3.2524 | -3.2327 | -3.2313 | -3.2057 | -3.1386 | -3.0873 |
| 332 | -3.2838 | -3.2834 | -3.2758 | -3.2676 | -3.2652 | -3.2644 | -3.2639 | -3.2367 | -3.2341 | -3.2257 |
| 394 | -3.2901 | -3.2875 | -3.2853 | -3.2831 | -3.2797 | -3.2777 | -3.2739 | -3.2681 | -3.2640 | -3.2415 |
| 456 | -3.2925 | -3.2900 | -3.2869 | -3.2865 | -3.2848 | -3.2841 | -3.2791 | -3.2787 | -3.2685 | -3.2646 |
| 518 | -3.2991 | -3.2975 | -3.2960 | -3.2950 | -3.2921 | -3.2901 | -3.2862 | -3.2787 | -3.2720 | -3.2704 |
| 580 | -3.3117 | -3.3060 | -3.3022 | -3.3008 | -3.3004 | -3.2989 | -3.2982 | -3.2927 | -3.2861 | -3.2777 |
| 642 | -3.3167 | -3.3119 | -3.3064 | -3.3012 | -3.3012 | -3.2991 | -3.2988 | -3.2920 | -3.2903 | -3.2833 |
| 704 | -3.3173 | -3.3071 | -3.3067 | -3.3056 | -3.3049 | -3.3046 | -3.3032 | -3.3015 | -3.2945 | -3.2930 |
| 766 | -3.3159 | -3.3115 | -3.3112 | -3.3100 | -3.3090 | -3.3050 | -3.3024 | -3.3008 | -3.2999 | -3.2917 |
| 828 | -3.3147 | -3.3128 | -3.3121 | -3.3104 | -3.3101 | -3.3090 | -3.3071 | -3.3013 | -3.2965 | -3.2928 |
| DMRG Energy: -3.3693 | | | | | | | | | | |

**Table S38** NP ansatz with U/t = 8, VQE Energies and DMRG Energy for lattice 1x11

| Num Parameters | VQE 1 | VQE 2 | VQE 3 | VQE 4 | VQE 5 | VQE 6 | VQE 7 | VQE 8 | VQE 9 | VQE 10 |
|---|---|---|---|---|---|---|---|---|---|---|
| 92 | -1.1909 | -1.1907 | -1.1907 | -1.1907 | -1.1903 | -1.1903 | -1.0741 | -1.0739 | -0.8553 | -0.8553 |
| 160 | -3.2791 | -3.2168 | -3.2037 | -3.1947 | -3.1644 | -3.1549 | -3.1444 | -3.1317 | -3.0959 | -3.0629 |
| 228 | -3.5358 | -3.5255 | -3.5242 | -3.5126 | -3.5114 | -3.5034 | -3.4619 | -3.4353 | -3.3719 | -3.2766 |
| 296 | -3.5754 | -3.5707 | -3.5587 | -3.5554 | -3.5497 | -3.5362 | -3.5241 | -3.5073 | -3.4914 | -3.4510 |
| 364 | -3.6040 | -3.5993 | -3.5953 | -3.5846 | -3.5742 | -3.5704 | -3.5704 | -3.5385 | -3.5221 | -3.5048 |
| 432 | -3.6217 | -3.6089 | -3.6053 | -3.6051 | -3.6016 | -3.5924 | -3.5846 | -3.5710 | -3.5578 | -3.5492 |
| 500 | -3.6274 | -3.6256 | -3.6144 | -3.6096 | -3.6089 | -3.6085 | -3.5990 | -3.5934 | -3.5709 | -3.5672 |
| 568 | -3.6266 | -3.6233 | -3.6219 | -3.6196 | -3.6165 | -3.6137 | -3.6124 | -3.6116 | -3.6058 | -3.5848 |
| 636 | -3.6232 | -3.6227 | -3.6202 | -3.6169 | -3.6155 | -3.6104 | -3.6102 | -3.6017 | -3.5995 | -3.5981 |
| 704 | -3.6318 | -3.6270 | -3.6258 | -3.6223 | -3.6205 | -3.6205 | -3.6202 | -3.6173 | -3.6147 | -3.6048 |
| 772 | -3.6344 | -3.6297 | -3.6266 | -3.6228 | -3.6227 | -3.6223 | -3.6195 | -3.6153 | -3.6135 | -3.6095 |
| 840 | -3.6341 | -3.6214 | -3.6201 | -3.6161 | -3.6149 | -3.6146 | -3.6142 | -3.6132 | -3.6071 | -3.5594 |
| 908 | -3.6116 | -3.6115 | -3.6106 | -3.6094 | -3.6066 | -3.6002 | -3.5935 | -3.5930 | -3.5656 | -3.5396 |
| DMRG Energy: -3.7284 | | | | | | | | | | |

**Table S39** NP ansatz with U/t = 8, VQE Energies and DMRG Energy for lattice 1x12

| Num Parameters | VQE 1 | VQE 2 | VQE 3 | VQE 4 | VQE 5 | VQE 6 | VQE 7 | VQE 8 | VQE 9 | VQE 10 |
|---|---|---|---|---|---|---|---|---|---|---|
| 32 | -0.5000 | -0.5000 | -0.5000 | -0.5000 | -0.5000 | -0.5000 | 0.0000 | 0.0000 | 0.0000 | 0.0000 |
| 56 | -1.2186 | -1.1863 | -1.1603 | -1.1603 | -1.1427 | -1.1172 | -1.1150 | -1.1125 | -1.0566 | -1.0187 |
| 80 | -1.2950 | -1.2616 | -1.2577 | -1.2566 | -1.2131 | -1.2007 | -1.1592 | -1.1562 | -0.9879 | -0.9876 |
| 104 | -1.3197 | -1.3156 | -1.3133 | -1.3121 | -1.3074 | -1.3063 | -1.2923 | -1.2836 | -1.2446 | -1.2253 |
| 128 | -1.3200 | -1.3199 | -1.3199 | -1.3199 | -1.3173 | -1.3162 | -1.3144 | -1.3040 | -1.3021 | -1.2784 |
| 152 | -1.3202 | -1.3202 | -1.3200 | -1.3200 | -1.3199 | -1.3197 | -1.3197 | -1.3191 | -1.3189 | -1.3184 |
| 176 | -1.3202 | -1.3202 | -1.3202 | -1.3202 | -1.3202 | -1.3202 | -1.3201 | -1.3201 | -1.3200 | -1.3192 |
| 200 | -1.3202 | -1.3202 | -1.3202 | -1.3202 | -1.3202 | -1.3202 | -1.3202 | -1.3202 | -1.3202 | -1.3202 |
| 224 | -1.3202 | -1.3202 | -1.3202 | -1.3202 | -1.3202 | -1.3202 | -1.3202 | -1.3202 | -1.3202 | -1.3202 |
| 248 | -1.3202 | -1.3202 | -1.3202 | -1.3202 | -1.3202 | -1.3202 | -1.3202 | -1.3202 | -1.3202 | -1.3202 |
| 272 | -1.3202 | -1.3202 | -1.3202 | -1.3202 | -1.3202 | -1.3202 | -1.3202 | -1.3202 | -1.3202 | -1.3202 |
| 296 | -1.3202 | -1.3202 | -1.3202 | -1.3202 | -1.3202 | -1.3202 | -1.3202 | -1.3202 | -1.3202 | -1.3202 |
| 320 | -1.3202 | -1.3202 | -1.3202 | -1.3202 | -1.3202 | -1.3202 | -1.3202 | -1.3202 | -1.3202 | -1.3202 |
| DMRG Energy: -1.3202 | | | | | | | | | | |

**Table S40** NP ansatz with U/t = 8, VQE Energies and DMRG Energy for lattice 2x2

| Num Parameters | VQE 1 | VQE 2 | VQE 3 | VQE 4 | VQE 5 | VQE 6 | VQE 7 | VQE 8 | VQE 9 | VQE 10 |
|---|---|---|---|---|---|---|---|---|---|---|
| 52 | -0.9565 | -0.9561 | -0.9274 | -0.7343 | -0.7343 | -0.7343 | -0.6125 | -0.5000 | -0.5000 | -0.5000 |
| 92 | -1.9833 | -1.8645 | -1.8611 | -1.8454 | -1.8336 | -1.8098 | -1.8084 | -1.8003 | -1.7799 | -1.3991 |
| 132 | -2.0351 | -2.0344 | -2.0276 | -2.0237 | -2.0208 | -2.0195 | -2.0151 | -1.9921 | -1.9601 | -1.9305 |
| 172 | -2.0703 | -2.0620 | -2.0410 | -2.0407 | -2.0366 | -2.0351 | -2.0253 | -2.0108 | -1.9805 | -1.9358 |
| 212 | -2.0817 | -2.0728 | -2.0723 | -2.0628 | -2.0558 | -2.0479 | -2.0476 | -2.0471 | -2.0172 | -1.9897 |
| 252 | -2.0802 | -2.0736 | -2.0669 | -2.0659 | -2.0632 | -2.0519 | -2.0505 | -2.0448 | -2.0297 | -1.9996 |
| 292 | -2.1201 | -2.0933 | -2.0861 | -2.0804 | -2.0715 | -2.0703 | -2.0668 | -2.0640 | -2.0078 | -2.0048 |
| 332 | -2.1145 | -2.1056 | -2.1000 | -2.0930 | -2.0883 | -2.0817 | -2.0813 | -2.0707 | -2.0626 | -2.0181 |
| 372 | -2.1035 | -2.0996 | -2.0981 | -2.0965 | -2.0938 | -2.0921 | -2.0916 | -2.0889 | -2.0882 | -2.0645 |
| 412 | -2.1355 | -2.1073 | -2.1023 | -2.1005 | -2.0969 | -2.0930 | -2.0876 | -2.0870 | -2.0851 | -2.0840 |
| 452 | -2.1237 | -2.1136 | -2.1092 | -2.1076 | -2.1075 | -2.1031 | -2.1019 | -2.0973 | -2.0945 | -2.0745 |
| 492 | -2.1492 | -2.1296 | -2.1272 | -2.1111 | -2.1103 | -2.1056 | -2.1041 | -2.1011 | -2.0948 | -2.0912 |
| 532 | -2.1591 | -2.1555 | -2.1180 | -2.1141 | -2.1130 | -2.1114 | -2.1058 | -2.0932 | -2.0884 | -2.0623 |
| DMRG Energy: -2.1778 | | | | | | | | | | |

**Table S41** NP ansatz with U/t = 8, VQE Energies and DMRG Energy for lattice 2x3

| Num Parameters | VQE 1 | VQE 2 | VQE 3 | VQE 4 | VQE 5 | VQE 6 | VQE 7 | VQE 8 | VQE 9 | VQE 10 |
|---|---|---|---|---|---|---|---|---|---|---|
| 84 | -1.7186 | -1.6955 | -1.6955 | -1.6955 | -1.6955 | -1.6955 | -1.6955 | -1.3205 | -0.8661 | -0.6598 |
| 150 | -3.0019 | -2.9996 | -2.9550 | -2.9062 | -2.8980 | -2.8978 | -2.8974 | -2.8974 | -2.8973 | -2.8894 |
| 216 | -3.3424 | -3.3349 | -3.3317 | -3.3316 | -3.2980 | -3.1871 | -3.1860 | -3.1833 | -3.1751 | -3.1560 |
| 282 | -3.3693 | -3.3649 | -3.3559 | -3.3463 | -3.3457 | -3.3300 | -3.3267 | -3.3141 | -3.2330 | -3.2309 |
| 348 | -3.3722 | -3.3704 | -3.3664 | -3.3660 | -3.3592 | -3.3571 | -3.3562 | -3.3379 | -3.3137 | -3.2704 |
| 414 | -3.3815 | -3.3809 | -3.3742 | -3.3732 | -3.3724 | -3.3723 | -3.3695 | -3.3690 | -3.3656 | -3.3645 |
| 480 | -3.3965 | -3.3895 | -3.3837 | -3.3823 | -3.3816 | -3.3815 | -3.3780 | -3.3715 | -3.3702 | -3.3695 |
| 546 | -3.3990 | -3.3938 | -3.3921 | -3.3878 | -3.3851 | -3.3849 | -3.3829 | -3.3819 | -3.3801 | -3.3776 |
| 612 | -3.4095 | -3.4031 | -3.4030 | -3.3980 | -3.3944 | -3.3856 | -3.3841 | -3.3826 | -3.3816 | -3.3783 |
| 678 | -3.4055 | -3.3996 | -3.3988 | -3.3982 | -3.3967 | -3.3966 | -3.3924 | -3.3901 | -3.3846 | -3.3843 |
| 744 | -3.4211 | -3.4116 | -3.4070 | -3.4055 | -3.3944 | -3.3942 | -3.3928 | -3.3914 | -3.3911 | -3.3872 |
| 810 | -3.4189 | -3.4131 | -3.4054 | -3.3985 | -3.3974 | -3.3947 | -3.3932 | -3.3924 | -3.3861 | -3.3471 |
| 876 | -3.4223 | -3.4207 | -3.4141 | -3.4063 | -3.4060 | -3.4029 | -3.4017 | -3.3998 | -3.3972 | -3.3925 |
| DMRG Energy: -3.4911 | | | | | | | | | | |

**Table S42** NP ansatz with U/t = 8, VQE Energies and DMRG Energy for lattice 3x3

# S4 NP ansatz, $U/t = 2$, $d = 0.2$

| Num Parameters | VQE 1 | VQE 2 | VQE 3 | VQE 4 | VQE 5 | VQE 6 | VQE 7 | VQE 8 | VQE 9 | VQE 10 |
|---|---|---|---|---|---|---|---|---|---|---|
| 32 | -1.4522 | -1.1804 | -0.9888 | -0.9888 | -0.9888 | -0.9888 | -0.9888 | -0.9888 | -0.9888 | -0.9888 |
| 56 | -2.2562 | -2.2562 | -2.2562 | -2.2562 | -2.2562 | -2.2562 | -2.2562 | -2.2532 | -2.2492 | -2.2487 |
| 80 | -2.3384 | -2.3346 | -2.3317 | -2.3227 | -2.3211 | -2.3196 | -2.3180 | -2.3171 | -2.3036 | -2.2985 |
| 104 | -2.3400 | -2.3400 | -2.3400 | -2.3400 | -2.3400 | -2.3400 | -2.3400 | -2.3400 | -2.3400 | -2.3400 |
| 128 | -2.3400 | -2.3400 | -2.3400 | -2.3400 | -2.3400 | -2.3400 | -2.3400 | -2.3400 | -2.3400 | -2.3400 |
| 152 | -2.3400 | -2.3400 | -2.3400 | -2.3400 | -2.3400 | -2.3400 | -2.3400 | -2.3400 | -2.3400 | -2.3400 |
| 176 | -2.3400 | -2.3400 | -2.3400 | -2.3400 | -2.3400 | -2.3400 | -2.3400 | -2.3400 | -2.3400 | -2.3400 |
| 200 | -2.3400 | -2.3400 | -2.3400 | -2.3400 | -2.3400 | -2.3400 | -2.3400 | -2.3400 | -2.3400 | -2.3400 |
| 224 | -2.3400 | -2.3400 | -2.3400 | -2.3400 | -2.3400 | -2.3400 | -2.3400 | -2.3400 | -2.3400 | -2.3400 |
| 248 | -2.3400 | -2.3400 | -2.3400 | -2.3400 | -2.3400 | -2.3400 | -2.3400 | -2.3400 | -2.3400 | -2.3400 |
| 272 | -2.3400 | -2.3400 | -2.3400 | -2.3400 | -2.3400 | -2.3400 | -2.3400 | -2.3400 | -2.3400 | -2.3400 |
| 296 | -2.3400 | -2.3400 | -2.3400 | -2.3400 | -2.3400 | -2.3400 | -2.3400 | -2.3400 | -2.3400 | -2.3400 |
| 320 | -2.3400 | -2.3400 | -2.3400 | -2.3400 | -2.3400 | -2.3400 | -2.3400 | -2.3400 | -2.3400 | -2.3400 |
| DMRG Energy: -2.3400 | | | | | | | | | | |

**Table S43** NP ansatz with U/t = 2 and d = 0.2, VQE Energies and DMRG Energy for lattice 2x2

| Num Parameters | VQE 1 | VQE 2 | VQE 3 | VQE 4 | VQE 5 | VQE 6 | VQE 7 | VQE 8 | VQE 9 | VQE 10 |
|---|---|---|---|---|---|---|---|---|---|---|
| 52 | -2.3626 | -2.3626 | -2.3626 | -2.3626 | -2.3624 | -2.3624 | -2.3624 | -2.3624 | -2.3610 | -2.3610 |
| 92 | -4.7765 | -4.7297 | -4.7297 | -4.6771 | -4.6755 | -4.6744 | -4.6744 | -4.6690 | -4.6306 | -4.6110 |
| 132 | -4.9714 | -4.9667 | -4.9664 | -4.9640 | -4.9626 | -4.9593 | -4.9481 | -4.9356 | -4.9223 | -4.8142 |
| 172 | -5.0301 | -5.0265 | -5.0262 | -5.0234 | -5.0212 | -5.0135 | -5.0098 | -5.0067 | -5.0053 | -4.9695 |
| 212 | -5.0807 | -5.0728 | -5.0692 | -5.0633 | -5.0602 | -5.0580 | -5.0562 | -5.0551 | -5.0519 | -5.0460 |
| 252 | -5.0941 | -5.0935 | -5.0923 | -5.0900 | -5.0874 | -5.0835 | -5.0825 | -5.0807 | -5.0702 | -5.0586 |
| 292 | -5.1032 | -5.1008 | -5.1003 | -5.0998 | -5.0966 | -5.0948 | -5.0941 | -5.0940 | -5.0933 | -5.0897 |
| 332 | -5.1079 | -5.1071 | -5.1063 | -5.1059 | -5.1044 | -5.1041 | -5.1036 | -5.1014 | -5.1005 | -5.1002 |
| 372 | -5.1103 | -5.1102 | -5.1096 | -5.1093 | -5.1084 | -5.1083 | -5.1078 | -5.1072 | -5.1060 | -5.1059 |
| 412 | -5.1145 | -5.1138 | -5.1133 | -5.1133 | -5.1132 | -5.1128 | -5.1125 | -5.1116 | -5.1101 | -5.1073 |
| 452 | -5.1163 | -5.1159 | -5.1153 | -5.1151 | -5.1149 | -5.1145 | -5.1143 | -5.1141 | -5.1138 | -5.1125 |
| 492 | -5.1168 | -5.1166 | -5.1166 | -5.1165 | -5.1165 | -5.1164 | -5.1161 | -5.1157 | -5.1156 | -5.1144 |
| 532 | -5.1184 | -5.1180 | -5.1178 | -5.1178 | -5.1175 | -5.1174 | -5.1174 | -5.1167 | -5.1166 | -5.1160 |
| DMRG Energy: -5.1201 | | | | | | | | | | |

**Table S44** NP ansatz with U/t = 2 and d = 0.2, VQE Energies and DMRG Energy for lattice 2x3

| Num Parameters | VQE 1 | VQE 2 | VQE 3 | VQE 4 | VQE 5 | VQE 6 | VQE 7 | VQE 8 | VQE 9 | VQE 10 |
|---|---|---|---|---|---|---|---|---|---|---|
| 84 | -4.8379 | -4.8379 | -4.8379 | -4.7771 | -4.7691 | -4.7582 | -4.7582 | -4.7582 | -4.7044 | -4.6248 |
| 150 | -8.1896 | -8.1843 | -8.1543 | -8.0511 | -8.0187 | -7.9992 | -7.9191 | -7.8403 | -7.8403 | -7.8403 |
| 216 | -8.8190 | -8.7522 | -8.6974 | -8.6747 | -8.6719 | -8.6655 | -8.6387 | -8.5702 | -8.5442 | -8.5420 |
| 282 | -8.9115 | -8.9030 | -8.8881 | -8.8747 | -8.8675 | -8.8527 | -8.8426 | -8.8398 | -8.8212 | -8.8073 |
| 348 | -8.9596 | -8.9313 | -8.9307 | -8.9284 | -8.9272 | -8.9230 | -8.9224 | -8.9224 | -8.9202 | -8.9018 |
| 414 | -8.9984 | -8.9811 | -8.9791 | -8.9780 | -8.9761 | -8.9683 | -8.9667 | -8.9660 | -8.9547 | -8.9501 |
| 480 | -9.0031 | -9.0026 | -9.0025 | -9.0020 | -9.0016 | -9.0014 | -8.9995 | -8.9983 | -8.9933 | -8.9866 |
| 546 | -9.0234 | -9.0198 | -9.0177 | -9.0159 | -9.0143 | -9.0103 | -9.0089 | -9.0065 | -8.9867 | -8.9859 |
| 612 | -9.0352 | -9.0345 | -9.0254 | -9.0237 | -9.0234 | -9.0231 | -9.0217 | -9.0146 | -9.0094 | -8.9917 |
| 678 | -9.0541 | -9.0511 | -9.0479 | -9.0277 | -9.0272 | -9.0269 | -9.0221 | -9.0217 | -9.0186 | -9.0094 |
| 744 | -9.0593 | -9.0538 | -9.0500 | -9.0451 | -9.0450 | -9.0427 | -9.0315 | -9.0291 | -9.0254 | -9.0160 |
| 810 | -9.0618 | -9.0594 | -9.0591 | -9.0547 | -9.0540 | -9.0510 | -9.0413 | -9.0408 | -9.0349 | -9.0218 |
| 876 | -9.0610 | -9.0602 | -9.0588 | -9.0587 | -9.0577 | -9.0559 | -9.0556 | -9.0522 | -9.0418 | -9.0334 |
| DMRG Energy: -9.0667 | | | | | | | | | | |

**Table S45** NP ansatz with U/t = 2 and d = 0.2, VQE Energies and DMRG Energy for lattice 3x3

## S5 NP ansatz, $U/t = 2$, $d = 0.8$

| Num Parameters | VQE 1 | VQE 2 | VQE 3 | VQE 4 | VQE 5 | VQE 6 | VQE 7 | VQE 8 | VQE 9 | VQE 10 |
|---|---|---|---|---|---|---|---|---|---|---|
| 32 | -0.4643 | -0.4643 | -0.4643 | -0.4643 | -0.4643 | -0.4643 | -0.4643 | -0.4643 | -0.4643 | -0.4643 |
| 56 | -2.8242 | -2.8225 | -2.8225 | -2.8222 | -2.8206 | -2.8200 | -2.8197 | -2.8141 | -2.4959 | -2.4932 |
| 80 | -2.8295 | -2.8294 | -2.8294 | -2.8292 | -2.8290 | -2.8290 | -2.8289 | -2.8289 | -2.8289 | -2.8277 |
| 104 | -2.8298 | -2.8298 | -2.8298 | -2.8298 | -2.8298 | -2.8298 | -2.8298 | -2.8298 | -2.8298 | -2.8298 |
| 128 | -2.8298 | -2.8298 | -2.8298 | -2.8298 | -2.8298 | -2.8298 | -2.8298 | -2.8298 | -2.8298 | -2.8298 |
| 152 | -2.8298 | -2.8298 | -2.8298 | -2.8298 | -2.8298 | -2.8298 | -2.8298 | -2.8298 | -2.8298 | -2.8298 |
| 176 | -2.8298 | -2.8298 | -2.8298 | -2.8298 | -2.8298 | -2.8298 | -2.8298 | -2.8298 | -2.8298 | -2.8298 |
| 200 | -2.8298 | -2.8298 | -2.8298 | -2.8298 | -2.8298 | -2.8298 | -2.8298 | -2.8298 | -2.8298 | -2.8298 |
| 224 | -2.8298 | -2.8298 | -2.8298 | -2.8298 | -2.8298 | -2.8298 | -2.8298 | -2.8298 | -2.8298 | -2.8298 |
| 248 | -2.8298 | -2.8298 | -2.8298 | -2.8298 | -2.8298 | -2.8298 | -2.8298 | -2.8298 | -2.8298 | -2.8298 |
| 272 | -2.8298 | -2.8298 | -2.8298 | -2.8298 | -2.8298 | -2.8298 | -2.8298 | -2.8298 | -2.8298 | -2.8298 |
| 296 | -2.8298 | -2.8298 | -2.8298 | -2.8298 | -2.8298 | -2.8298 | -2.8298 | -2.8298 | -2.8298 | -2.8298 |
| 320 | -2.8298 | -2.8298 | -2.8298 | -2.8298 | -2.8298 | -2.8298 | -2.8298 | -2.8298 | -2.8298 | -2.8298 |
| DMRG Energy: -2.8298 | | | | | | | | | | |

**Table S46** NP ansatz with U/t = 2 and d = 0.8, VQE Energies and DMRG Energy for lattice 2x2

| Num Parameters | VQE 1 | VQE 2 | VQE 3 | VQE 4 | VQE 5 | VQE 6 | VQE 7 | VQE 8 | VQE 9 | VQE 10 |
|---|---|---|---|---|---|---|---|---|---|---|
| 52 | -4.2806 | -4.2800 | -4.2800 | -4.1260 | -4.1260 | -4.1260 | -4.1260 | -4.0411 | -4.0411 | -3.7305 |
| 92 | -5.3513 | -5.2851 | -5.2790 | -5.2780 | -5.2765 | -5.2765 | -5.2751 | -5.2693 | -5.2683 | -5.2589 |
| 132 | -5.6288 | -5.6176 | -5.6021 | -5.5758 | -5.5718 | -5.4601 | -5.4556 | -5.4529 | -5.4368 | -5.4320 |
| 172 | -5.6708 | -5.6704 | -5.6699 | -5.6684 | -5.6615 | -5.6565 | -5.6548 | -5.6522 | -5.6482 | -5.6434 |
| 212 | -5.6911 | -5.6867 | -5.6866 | -5.6865 | -5.6857 | -5.6852 | -5.6843 | -5.6806 | -5.6802 | -5.6771 |
| 252 | -5.6973 | -5.6965 | -5.6961 | -5.6957 | -5.6954 | -5.6952 | -5.6950 | -5.6943 | -5.6929 | -5.6903 |
| 292 | -5.7004 | -5.6998 | -5.6988 | -5.6975 | -5.6965 | -5.6964 | -5.6960 | -5.6959 | -5.6956 | -5.6945 |
| 332 | -5.7016 | -5.7012 | -5.7006 | -5.7005 | -5.7004 | -5.7003 | -5.7003 | -5.7000 | -5.6987 | -5.6982 |
| 372 | -5.7024 | -5.7023 | -5.7023 | -5.7022 | -5.7021 | -5.7019 | -5.7018 | -5.7014 | -5.7012 | -5.7011 |
| 412 | -5.7029 | -5.7029 | -5.7025 | -5.7025 | -5.7024 | -5.7024 | -5.7022 | -5.7020 | -5.7016 | -5.7009 |
| 452 | -5.7035 | -5.7035 | -5.7030 | -5.7029 | -5.7029 | -5.7029 | -5.7028 | -5.7027 | -5.7015 | -5.7007 |
| 492 | -5.7036 | -5.7036 | -5.7033 | -5.7033 | -5.7033 | -5.7032 | -5.7031 | -5.7031 | -5.7030 | -5.7024 |
| 532 | -5.7035 | -5.7035 | -5.7035 | -5.7035 | -5.7034 | -5.7034 | -5.7034 | -5.7033 | -5.7030 | -5.7030 |
| DMRG Energy: -5.7043 | | | | | | | | | | |

**Table S47** NP ansatz with U/t = 2 and d = 0.8, VQE Energies and DMRG Energy for lattice 2x3

| Num Parameters | VQE 1 | VQE 2 | VQE 3 | VQE 4 | VQE 5 | VQE 6 | VQE 7 | VQE 8 | VQE 9 | VQE 10 |
|---|---|---|---|---|---|---|---|---|---|---|
| 84 | -9.0353 | -9.0353 | -9.0351 | -9.0268 | -9.0268 | -9.0264 | -9.0183 | -8.7007 | -8.7007 | -8.6893 |
| 150 | -13.3482 | -13.3371 | -13.2662 | -13.1633 | -13.1431 | -12.9668 | -12.9637 | -12.9542 | -12.9374 | -12.9219 |
| 216 | -13.8365 | -13.8343 | -13.8222 | -13.8150 | -13.8134 | -13.8005 | -13.8003 | -13.7981 | -13.7576 | -13.7480 |
| 282 | -13.8971 | -13.8967 | -13.8940 | -13.8893 | -13.8849 | -13.8774 | -13.8712 | -13.8653 | -13.8651 | -13.8528 |
| 348 | -13.9142 | -13.9107 | -13.9098 | -13.9044 | -13.9020 | -13.8990 | -13.8955 | -13.8917 | -13.8905 | -13.8903 |
| 414 | -13.9206 | -13.9201 | -13.9196 | -13.9191 | -13.9187 | -13.9157 | -13.9149 | -13.9142 | -13.9137 | -13.9047 |
| 480 | -13.9226 | -13.9213 | -13.9210 | -13.9209 | -13.9191 | -13.9189 | -13.9188 | -13.9178 | -13.9156 | -13.9155 |
| 546 | -13.9261 | -13.9258 | -13.9252 | -13.9247 | -13.9241 | -13.9239 | -13.9230 | -13.9223 | -13.9222 | -13.9207 |
| 612 | -13.9295 | -13.9281 | -13.9275 | -13.9274 | -13.9261 | -13.9258 | -13.9256 | -13.9239 | -13.9235 | -13.9206 |
| 678 | -13.9301 | -13.9300 | -13.9292 | -13.9282 | -13.9269 | -13.9265 | | | | |
| 744 | -13.9316 | -13.9314 | -13.9304 | -13.9302 | -13.9287 | -13.9286 | -13.9285 | | | |
| 810 | -13.9316 | -13.9314 | -13.9314 | -13.9303 | -13.9303 | -13.9297 | -13.9293 | -13.9291 | -13.9290 | |
| 876 | -13.9314 | -13.9313 | -13.9311 | -13.9302 | -13.9301 | -13.9297 | -13.9291 | | | |
| DMRG Energy: -13.9354 | | | | | | | | | | |

**Table S48** NP ansatz with U/t = 2 and d = 0.8, VQE Energies and DMRG Energy for lattice 3x3

# S6 NP ansatz, $U/t = 2$, $V = 0.2$

| Num Parameters | VQE 1 | VQE 2 | VQE 3 | VQE 4 | VQE 5 | VQE 6 | VQE 7 | VQE 8 | VQE 9 | VQE 10 |
|---|---|---|---|---|---|---|---|---|---|---|
| 32 | -1.8182 | -1.8182 | -1.8182 | -1.8000 | -1.8000 | -1.8000 | -1.4373 | -1.4373 | -0.0142 | 0.0000 |
| 56 | -2.5905 | -2.5905 | -2.5836 | -2.5832 | -2.5830 | -2.5817 | -2.5801 | -2.5704 | -2.5611 | -2.5081 |
| 80 | -2.6681 | -2.6680 | -2.6557 | -2.6462 | -2.6305 | -2.6076 | -2.6073 | -2.6073 | -2.6056 | -2.6048 |
| 104 | -2.6681 | -2.6681 | -2.6681 | -2.6678 | -2.6677 | -2.6673 | -2.6639 | -2.6623 | -2.6623 | -2.6462 |
| 128 | -2.6681 | -2.6681 | -2.6681 | -2.6681 | -2.6681 | -2.6681 | -2.6681 | -2.6681 | -2.6681 | -2.6299 |
| 152 | -2.6681 | -2.6681 | -2.6681 | -2.6681 | -2.6681 | -2.6681 | -2.6681 | -2.6681 | -2.6680 | -2.6679 |
| 176 | -2.6681 | -2.6681 | -2.6681 | -2.6681 | -2.6681 | -2.6681 | -2.6681 | -2.6681 | -2.6681 | -2.6681 |
| 200 | -2.6681 | -2.6681 | -2.6681 | -2.6681 | -2.6681 | -2.6681 | -2.6681 | -2.6681 | -2.6681 | -2.6681 |
| 224 | -2.6681 | -2.6681 | -2.6681 | -2.6681 | -2.6681 | -2.6681 | -2.6681 | -2.6681 | -2.6681 | -2.6681 |
| 248 | -2.6681 | -2.6681 | -2.6681 | -2.6681 | -2.6681 | -2.6681 | -2.6681 | -2.6681 | -2.6681 | -2.6681 |
| 272 | -2.6681 | -2.6681 | -2.6681 | -2.6681 | -2.6681 | -2.6681 | -2.6681 | -2.6681 | -2.6681 | -2.6681 |
| 296 | -2.6681 | -2.6681 | -2.6681 | -2.6681 | -2.6681 | -2.6681 | -2.6681 | -2.6681 | -2.6681 | -2.6681 |
| 320 | -2.6681 | -2.6681 | -2.6681 | -2.6681 | -2.6681 | -2.6681 | -2.6681 | -2.6681 | -2.6681 | -2.6681 |
| DMRG Energy: -2.6681 | | | | | | | | | | |

**Table S49** NP ansatz with U/t = 2 and V = 0.2, VQE Energies and DMRG Energy for lattice 2x2

| Num Parameters | VQE 1 | VQE 2 | VQE 3 | VQE 4 | VQE 5 | VQE 6 | VQE 7 | VQE 8 | VQE 9 | VQE 10 |
|---|---|---|---|---|---|---|---|---|---|---|
| 52 | -2.2728 | -2.2728 | -2.2728 | -2.1695 | -2.1695 | -2.1695 | -2.1403 | -2.1403 | -2.1403 | -1.4402 |
| 92 | -4.4213 | -4.3303 | -4.2455 | -4.2455 | -4.2455 | -4.2455 | -4.2432 | -4.2178 | -4.2178 | -4.1421 |
| 132 | -4.6875 | -4.6342 | -4.6324 | -4.5600 | -4.5499 | -4.5396 | -4.5344 | -4.5340 | -4.5332 | -4.5297 |
| 172 | -4.7342 | -4.7341 | -4.7338 | -4.7281 | -4.7279 | -4.7238 | -4.7232 | -4.7161 | -4.7017 | -4.6192 |
| 212 | -4.7557 | -4.7431 | -4.7419 | -4.7410 | -4.7406 | -4.7402 | -4.7378 | -4.7375 | -4.7338 | -4.7215 |
| 252 | -4.7581 | -4.7555 | -4.7554 | -4.7550 | -4.7543 | -4.7515 | -4.7514 | -4.7510 | -4.7509 | -4.7503 |
| 292 | -4.7603 | -4.7603 | -4.7597 | -4.7592 | -4.7588 | -4.7587 | -4.7583 | -4.7566 | -4.7565 | -4.7539 |
| 332 | -4.7607 | -4.7604 | -4.7603 | -4.7601 | -4.7599 | -4.7589 | -4.7589 | -4.7586 | -4.7580 | -4.7477 |
| 372 | -4.7613 | -4.7599 | -4.7597 | -4.7596 | -4.7592 | -4.7589 | -4.7580 | -4.7576 | -4.7546 | -4.7544 |
| 412 | -4.7614 | -4.7610 | -4.7607 | -4.7605 | -4.7604 | -4.7603 | -4.7601 | -4.7600 | -4.7600 | -4.7591 |
| 452 | -4.7614 | -4.7614 | -4.7611 | -4.7611 | -4.7608 | -4.7608 | -4.7608 | -4.7605 | -4.7605 | -4.7603 |
| 492 | -4.7618 | -4.7616 | -4.7616 | -4.7615 | -4.7614 | -4.7612 | -4.7611 | -4.7611 | -4.7608 | -4.7606 |
| 532 | -4.7617 | -4.7617 | -4.7617 | -4.7616 | -4.7616 | -4.7615 | -4.7611 | -4.7605 | -4.7603 | -4.7598 |
| DMRG Energy: -4.7620 | | | | | | | | | | |

**Table S50** NP ansatz with U/t = 2 and V = 0.2, VQE Energies and DMRG Energy for lattice 2x3

| Num Parameters | VQE 1 | VQE 2 | VQE 3 | VQE 4 | VQE 5 | VQE 6 | VQE 7 | VQE 8 | VQE 9 | VQE 10 |
|---|---|---|---|---|---|---|---|---|---|---|
| 84 | -3.7638 | -3.7638 | -3.7477 | -3.7128 | -3.6577 | -3.6577 | -3.6577 | -3.6577 | -3.6577 | -3.6577 |
| 150 | -6.4484 | -6.4484 | -6.4484 | -6.4484 | -6.4484 | -6.4260 | -6.4260 | -6.3949 | -6.3893 | -6.3826 |
| 216 | -7.0233 | -6.9852 | -6.9852 | -6.9852 | -6.9852 | -6.9852 | -6.9852 | -6.9852 | -6.9852 | -6.9846 |
| 282 | -7.1740 | -7.1740 | -7.1740 | -7.1740 | -7.1740 | -7.1740 | -7.1740 | -7.1740 | -7.1740 | -7.1740 |
| 348 | -7.2519 | -7.2394 | -7.2394 | -7.2394 | -7.2394 | -7.2394 | -7.2394 | -7.2394 | -7.2394 | -7.2394 |
| 414 | -7.2683 | -7.2683 | -7.2683 | -7.2683 | -7.2683 | -7.2683 | -7.2683 | -7.2683 | -7.2683 | -7.2683 |
| 480 | -7.2804 | -7.2804 | -7.2804 | -7.2804 | -7.2804 | -7.2804 | -7.2804 | -7.2804 | -7.2804 | -7.2804 |
| 546 | -7.2860 | -7.2859 | -7.2859 | -7.2859 | -7.2859 | -7.2859 | -7.2857 | -7.2857 | -7.2856 | -7.2854 |
| 612 | -7.2890 | -7.2890 | -7.2889 | -7.2889 | -7.2889 | -7.2888 | -7.2888 | -7.2887 | -7.2887 | -7.2886 |
| 678 | -7.2910 | -7.2910 | -7.2910 | -7.2910 | -7.2909 | -7.2908 | -7.2907 | -7.2907 | -7.2904 | -7.2903 |
| 744 | -7.2928 | -7.2924 | -7.2923 | -7.2922 | -7.2922 | -7.2921 | -7.2919 | -7.2919 | -7.2919 | -7.2918 |
| 810 | -7.2931 | -7.2930 | -7.2929 | -7.2929 | -7.2928 | -7.2928 | -7.2928 | -7.2928 | -7.2925 | -7.2922 |
| 876 | -7.2936 | -7.2934 | -7.2932 | -7.2931 | -7.2928 | -7.2927 | -7.2926 | -7.2926 | -7.2923 | -7.2920 |
| DMRG Energy: -7.3037 | | | | | | | | | | |

**Table S51** NP ansatz with U/t = 2 and V = 0.2, VQE Energies and DMRG Energy for lattice 3x3

## S7 NP ansatz, $U/t = 2$, $V = 0.8$

| Num Parameters | VQE 1 | VQE 2 | VQE 3 | VQE 4 | VQE 5 | VQE 6 | VQE 7 | VQE 8 | VQE 9 | VQE 10 |
|---|---|---|---|---|---|---|---|---|---|---|
| 32 | -1.3327 | -1.1962 | -1.0132 | -1.0132 | 0.0000 | 0.0000 | 0.0000 | 0.0000 | 0.0000 | 0.0000 |
| 56 | -2.1824 | -2.1824 | -2.1820 | -2.1243 | -2.1146 | -2.0773 | -2.0560 | -1.9919 | -1.9131 | -1.2949 |
| 80 | -2.2684 | -2.2655 | -2.2649 | -2.2635 | -2.2619 | -2.2610 | -2.2604 | -2.2562 | -2.2535 | -2.2527 |
| 104 | -2.2686 | -2.2686 | -2.2686 | -2.2684 | -2.2684 | -2.2680 | -2.2672 | -2.2663 | -2.2603 | -2.2499 |
| 128 | -2.2686 | -2.2686 | -2.2686 | -2.2686 | -2.2686 | -2.2686 | -2.2685 | -2.2673 | -2.2658 | -2.2615 |
| 152 | -2.2686 | -2.2686 | -2.2686 | -2.2686 | -2.2686 | -2.2686 | -2.2685 | -2.2685 | -2.2684 | -2.2684 |
| 176 | -2.2686 | -2.2686 | -2.2686 | -2.2686 | -2.2686 | -2.2686 | -2.2686 | -2.2686 | -2.2686 | -2.2686 |
| 200 | -2.2686 | -2.2686 | -2.2686 | -2.2686 | -2.2686 | -2.2686 | -2.2686 | -2.2686 | -2.2686 | -2.2686 |
| 224 | -2.2686 | -2.2686 | -2.2686 | -2.2686 | -2.2686 | -2.2686 | -2.2686 | -2.2686 | -2.2686 | -2.2686 |
| 248 | -2.2686 | -2.2686 | -2.2686 | -2.2686 | -2.2686 | -2.2686 | -2.2686 | -2.2686 | -2.2686 | -2.2686 |
| 272 | -2.2686 | -2.2686 | -2.2686 | -2.2686 | -2.2686 | -2.2686 | -2.2686 | -2.2686 | -2.2686 | -2.2686 |
| 296 | -2.2686 | -2.2686 | -2.2686 | -2.2686 | -2.2686 | -2.2686 | -2.2686 | -2.2686 | -2.2686 | -2.2686 |
| 320 | -2.2686 | -2.2686 | -2.2686 | -2.2686 | -2.2686 | -2.2686 | -2.2686 | -2.2686 | -2.2686 | -2.2686 |
| DMRG Energy: -2.2686 | | | | | | | | | | |

**Table S52** NP ansatz with U/t = 2 and V = 0.8, VQE Energies and DMRG Energy for lattice 2x2

| Num Parameters | VQE 1 | VQE 2 | VQE 3 | VQE 4 | VQE 5 | VQE 6 | VQE 7 | VQE 8 | VQE 9 | VQE 10 |
|---|---|---|---|---|---|---|---|---|---|---|
| 52 | -1.6493 | -1.6493 | -1.6493 | -1.6493 | -1.6493 | -1.6493 | -1.6493 | -1.6493 | -1.6493 | -1.6493 |
| 92 | -2.9897 | -2.9764 | -2.9431 | -2.9050 | -2.8385 | -2.7614 | -2.6661 | -2.6533 | -2.6297 | -2.3220 |
| 132 | -3.6849 | -3.6845 | -3.6685 | -3.6258 | -3.6158 | -3.5980 | -3.5783 | -3.5035 | -3.4350 | -3.3467 |
| 172 | -3.7915 | -3.7808 | -3.7795 | -3.7769 | -3.7582 | -3.7514 | -3.7350 | -3.7261 | -3.7235 | -3.7168 |
| 212 | -3.8038 | -3.8033 | -3.8007 | -3.8001 | -3.7990 | -3.7959 | -3.7932 | -3.7909 | -3.7799 | -3.7705 |
| 252 | -3.8119 | -3.8089 | -3.8059 | -3.8055 | -3.8054 | -3.8042 | -3.7983 | -3.7933 | -3.7882 | -3.7720 |
| 292 | -3.8149 | -3.8134 | -3.8130 | -3.8078 | -3.8076 | -3.8043 | -3.8025 | -3.8023 | -3.8018 | -3.7989 |
| 332 | -3.8176 | -3.8161 | -3.8136 | -3.8127 | -3.8096 | -3.8090 | -3.8087 | -3.8087 | -3.8076 | -3.8064 |
| 372 | -3.8181 | -3.8176 | -3.8162 | -3.8151 | -3.8146 | -3.8143 | -3.8138 | -3.8124 | -3.8071 | -3.7904 |
| 412 | -3.8176 | -3.8167 | -3.8167 | -3.8164 | -3.8159 | -3.8158 | -3.8158 | -3.8155 | -3.8140 | -3.8110 |
| 452 | -3.8183 | -3.8181 | -3.8177 | -3.8172 | -3.8168 | -3.8163 | -3.8152 | -3.8151 | -3.8132 | -3.8119 |
| 492 | -3.8192 | -3.8185 | -3.8184 | -3.8183 | -3.8182 | -3.8179 | -3.8177 | -3.8175 | -3.8174 | -3.8164 |
| 532 | -3.8195 | -3.8193 | -3.8192 | -3.8191 | -3.8189 | -3.8187 | -3.8182 | -3.8180 | -3.8176 | -3.8163 |
| DMRG Energy: -3.8199 | | | | | | | | | | |

**Table S53** NP ansatz with U/t = 2 and V = 0.8, VQE Energies and DMRG Energy for lattice 2x3

| Num Parameters | VQE 1 | VQE 2 | VQE 3 | VQE 4 | VQE 5 | VQE 6 | VQE 7 | VQE 8 | VQE 9 | VQE 10 |
|---|---|---|---|---|---|---|---|---|---|---|
| 84 | -2.9552 | -2.9552 | -2.9552 | -2.9551 | -2.9551 | -2.9551 | -2.9551 | -2.9551 | -2.9551 | -2.9551 |
| 150 | -5.1978 | -5.1978 | -5.1978 | -5.1977 | -5.1977 | -5.1977 | -5.1977 | -5.1977 | -5.1977 | -5.1977 |
| 216 | -5.6304 | -5.6304 | -5.6303 | -5.6303 | -5.6303 | -5.6303 | -5.6159 | -5.6128 | -5.6110 | -5.6021 |
| 282 | -5.7322 | -5.7322 | -5.7322 | -5.7322 | -5.7322 | -5.7322 | -5.7320 | -5.7312 | -5.7310 | -5.7219 |
| 348 | -5.7688 | -5.7687 | -5.7687 | -5.7687 | -5.7687 | -5.7687 | -5.7687 | -5.7687 | -5.7686 | -5.7619 |
| 414 | -5.7823 | -5.7822 | -5.7822 | -5.7821 | -5.7821 | -5.7821 | -5.7821 | -5.7820 | -5.7785 | -5.7769 |
| 480 | -5.7868 | -5.7867 | -5.7867 | -5.7867 | -5.7867 | -5.7866 | -5.7866 | -5.7864 | -5.7864 | -5.7847 |
| 546 | -5.7886 | -5.7886 | -5.7885 | -5.7884 | -5.7884 | -5.7883 | -5.7883 | -5.7882 | -5.7881 | -5.7879 |
| 612 | -5.7894 | -5.7894 | -5.7893 | -5.7893 | -5.7893 | -5.7891 | -5.7890 | -5.7887 | -5.7885 | -5.7881 |
| 678 | -5.7895 | -5.7895 | -5.7893 | -5.7893 | -5.7892 | -5.7890 | -5.7889 | -5.7886 | -5.7885 | -5.7885 |
| 744 | -5.7897 | -5.7897 | -5.7895 | -5.7893 | -5.7893 | -5.7892 | -5.7892 | -5.7891 | -5.7890 | -5.7889 |
| 810 | -5.7899 | -5.7899 | -5.7894 | -5.7894 | -5.7894 | -5.7893 | -5.7893 | -5.7892 | -5.7889 | -5.7888 |
| 876 | -5.7902 | -5.7899 | -5.7899 | -5.7898 | -5.7897 | -5.7896 | -5.7895 | -5.7894 | -5.7890 | -5.7887 |
| DMRG Energy: -5.7925 | | | | | | | | | | |

**Table S54** NP ansatz with U/t = 2 and V = 0.8, VQE Energies and DMRG Energy for lattice 3x3

# S8 NP ansatz, $U/t = 2$, overlap-based optimization

| Num Parameters | VQE 1 | VQE 2 | VQE 3 | VQE 4 | VQE 5 | VQE 6 | VQE 7 | VQE 8 | VQE 9 | VQE 10 |
|---|---|---|---|---|---|---|---|---|---|---|
| 12 | 0.0001 | 0.0061 | 0.0106 | 0.0133 | 0.0257 | 0.0862 | 0.1650 | 0.1943 | 0.3517 | 0.4414 |
| 20 | -1.2361 | -1.2361 | -1.2361 | -1.2361 | -1.2361 | -1.2361 | -1.2361 | -1.2361 | -1.2361 | -1.2361 |
| 28 | -1.2361 | -1.2361 | -1.2361 | -1.2361 | -1.2361 | -1.2361 | -1.2361 | -1.2361 | -1.2361 | -1.2361 |
| 36 | -1.2361 | -1.2361 | -1.2361 | -1.2361 | -1.2361 | -1.2361 | -1.2361 | -1.2361 | -1.2361 | -1.2361 |
| 44 | -1.2361 | -1.2361 | -1.2361 | -1.2361 | -1.2361 | -1.2361 | -1.2361 | -1.2361 | -1.2361 | -1.2361 |
| 52 | -1.2361 | -1.2361 | -1.2361 | -1.2361 | -1.2361 | -1.2361 | -1.2361 | -1.2361 | -1.2361 | -1.2361 |
| 60 | -1.2361 | -1.2361 | -1.2361 | -1.2361 | -1.2361 | -1.2361 | -1.2361 | -1.2361 | -1.2361 | -1.2361 |
| 68 | -1.2361 | -1.2361 | -1.2361 | -1.2361 | -1.2361 | -1.2361 | -1.2361 | -1.2361 | -1.2361 | -1.2361 |
| 76 | -1.2361 | -1.2361 | -1.2361 | -1.2361 | -1.2361 | -1.2361 | -1.2361 | -1.2361 | -1.2361 | -1.2361 |
| 84 | -1.2361 | -1.2361 | -1.2361 | -1.2361 | -1.2361 | -1.2361 | -1.2361 | -1.2361 | -1.2361 | -1.2361 |
| 92 | -1.2361 | -1.2361 | -1.2361 | -1.2361 | -1.2361 | -1.2361 | -1.2361 | -1.2361 | -1.2361 | -1.2361 |
| 100 | -1.2361 | -1.2361 | -1.2361 | -1.2361 | -1.2361 | -1.2361 | -1.2361 | -1.2361 | -1.2361 | -1.2361 |
| 108 | -1.2361 | -1.2361 | -1.2361 | -1.2361 | -1.2361 | -1.2361 | -1.2361 | -1.2361 | -1.2361 | -1.2361 |
| DMRG Energy: -1.2361 | | | | | | | | | | |

**Table S55** NP ansatz with U/t = 2, overlap-based VQE Energies and DMRG Energy for lattice 1x2

| Num Parameters | VQE 1 | VQE 2 | VQE 3 | VQE 4 | VQE 5 | VQE 6 | VQE 7 | VQE 8 | VQE 9 | VQE 10 |
|---|---|---|---|---|---|---|---|---|---|---|
| 20 | -0.4109 | -0.4109 | -0.4109 | -0.4109 | -0.4109 | 0.0000 | 0.0000 | 0.0000 | 0.0000 | 0.0000 |
| 34 | -1.8200 | -1.8137 | -1.8137 | -1.8137 | -1.7968 | -1.7617 | -1.7599 | -1.7453 | -1.7387 | -1.7262 |
| 48 | -1.8201 | -1.8201 | -1.8201 | -1.8201 | -1.8201 | -1.8201 | -1.8201 | -1.8201 | -1.8201 | -1.8201 |
| 62 | -1.8201 | -1.8201 | -1.8201 | -1.8201 | -1.8201 | -1.8201 | -1.8201 | -1.8201 | -1.8201 | -1.8201 |
| 76 | -1.8201 | -1.8201 | -1.8201 | -1.8201 | -1.8201 | -1.8201 | -1.8201 | -1.8201 | -1.8201 | -1.8201 |
| 90 | -1.8201 | -1.8201 | -1.8201 | -1.8201 | -1.8201 | -1.8201 | -1.8201 | -1.8201 | -1.8201 | -1.8201 |
| 104 | -1.8201 | -1.8201 | -1.8201 | -1.8201 | -1.8201 | -1.8201 | -1.8201 | -1.8201 | -1.8201 | -1.8201 |
| 118 | -1.8201 | -1.8201 | -1.8201 | -1.8201 | -1.8201 | -1.8201 | -1.8201 | -1.8201 | -1.8201 | -1.8201 |
| 132 | -1.8201 | -1.8201 | -1.8201 | -1.8201 | -1.8201 | -1.8201 | -1.8201 | -1.8201 | -1.8201 | -1.8201 |
| 146 | -1.8201 | -1.8201 | -1.8201 | -1.8201 | -1.8201 | -1.8201 | -1.8201 | -1.8201 | -1.8201 | -1.8201 |
| 160 | -1.8201 | -1.8201 | -1.8201 | -1.8201 | -1.8201 | -1.8201 | -1.8201 | -1.8201 | -1.8201 | -1.8201 |
| 174 | -1.8201 | -1.8201 | -1.8201 | -1.8201 | -1.8201 | -1.8201 | -1.8201 | -1.8201 | -1.8201 | -1.8201 |
| 188 | -1.8201 | -1.8201 | -1.8201 | -1.8201 | -1.8201 | -1.8201 | -1.8201 | -1.8201 | -1.8201 | -1.8201 |
| DMRG Energy: -1.8201 | | | | | | | | | | |

**Table S56** NP ansatz with U/t = 2, overlap-based VQE Energies and DMRG Energy for lattice 1x3

| Num Parameters | VQE 1 | VQE 2 | VQE 3 | VQE 4 | VQE 5 | VQE 6 | VQE 7 | VQE 8 | VQE 9 | VQE 10 |
|---|---|---|---|---|---|---|---|---|---|---|
| 28 | -0.1341 | -0.1341 | -0.1341 | -0.1341 | -0.1341 | -0.1341 | -0.1341 | 0.0000 | 0.0000 | 0.0000 |
| 48 | -2.8313 | -2.8242 | -2.8242 | -2.8242 | -2.8093 | -2.8081 | -2.7493 | -2.6808 | -2.6433 | -2.4869 |
| 68 | -2.8738 | -2.8737 | -2.8728 | -2.8728 | -2.8717 | -2.8678 | -2.8676 | -2.8639 | -2.8630 | -2.8550 |
| 88 | -2.8756 | -2.8755 | -2.8753 | -2.8751 | -2.8750 | -2.8747 | -2.8747 | -2.8725 | -2.8671 | -2.8643 |
| 108 | -2.8759 | -2.8759 | -2.8758 | -2.8758 | -2.8757 | -2.8757 | -2.8756 | -2.8754 | -2.8753 | -2.8731 |
| 128 | -2.8759 | -2.8759 | -2.8759 | -2.8759 | -2.8759 | -2.8759 | -2.8758 | -2.8756 | -2.8754 | -2.8753 |
| 148 | -2.8759 | -2.8759 | -2.8759 | -2.8759 | -2.8759 | -2.8759 | -2.8759 | -2.8759 | -2.8759 | -2.8759 |
| 168 | -2.8759 | -2.8759 | -2.8759 | -2.8759 | -2.8759 | -2.8759 | -2.8759 | -2.8759 | -2.8759 | -2.8759 |
| 188 | -2.8759 | -2.8759 | -2.8759 | -2.8759 | -2.8759 | -2.8759 | -2.8759 | -2.8759 | -2.8759 | -2.8759 |
| 208 | -2.8759 | -2.8759 | -2.8759 | -2.8759 | -2.8759 | -2.8759 | -2.8759 | -2.8759 | -2.8759 | -2.8759 |
| 228 | -2.8759 | -2.8759 | -2.8759 | -2.8759 | -2.8759 | -2.8759 | -2.8759 | -2.8759 | -2.8759 | -2.8759 |
| 248 | -2.8759 | -2.8759 | -2.8759 | -2.8759 | -2.8759 | -2.8759 | -2.8759 | -2.8759 | -2.8759 | -2.8759 |
| 268 | -2.8759 | -2.8759 | -2.8759 | -2.8759 | -2.8759 | -2.8759 | -2.8759 | -2.8759 | -2.8759 | -2.8759 |
| DMRG Energy: -2.8759 | | | | | | | | | | |

**Table S57** NP ansatz with U/t = 2, overlap-based VQE Energies and DMRG Energy for lattice 1x4

| Num Parameters | VQE 1 | VQE 2 | VQE 3 | VQE 4 | VQE 5 | VQE 6 | VQE 7 | VQE 8 | VQE 9 | VQE 10 |
|---|---|---|---|---|---|---|---|---|---|---|
| 36 | -1.0671 | -1.0671 | -1.0671 | -1.0671 | -1.0526 | -1.0526 | -1.0526 | -1.0526 | -0.4024 | 0.0346 |
| 62 | -3.3630 | -3.3607 | -3.3528 | -3.3516 | -3.3442 | -3.2237 | -3.1972 | -3.1956 | -3.1584 | -3.1072 |
| 88 | -3.5310 | -3.5261 | -3.5060 | -3.5054 | -3.5002 | -3.4883 | -3.4862 | -3.4688 | -3.4607 | -3.4590 |
| 114 | -3.5412 | -3.5392 | -3.5389 | -3.5385 | -3.5384 | -3.5355 | -3.5344 | -3.5283 | -3.5275 | -3.5234 |
| 140 | -3.5500 | -3.5499 | -3.5494 | -3.5475 | -3.5458 | -3.5448 | -3.5439 | -3.5438 | -3.5436 | -3.5427 |
| 166 | -3.5527 | -3.5525 | -3.5524 | -3.5522 | -3.5520 | -3.5516 | -3.5516 | -3.5512 | -3.5507 | -3.5484 |
| 192 | -3.5532 | -3.5530 | -3.5528 | -3.5528 | -3.5527 | -3.5526 | -3.5525 | -3.5511 | -3.5506 | -3.5500 |
| 218 | -3.5537 | -3.5531 | -3.5530 | -3.5530 | -3.5528 | -3.5527 | -3.5513 | -3.5512 | -3.5510 | -3.5496 |
| 244 | -3.5538 | -3.5538 | -3.5538 | -3.5537 | -3.5537 | -3.5534 | -3.5533 | -3.5532 | -3.5531 | -3.5526 |
| 270 | -3.5540 | -3.5539 | -3.5539 | -3.5539 | -3.5539 | -3.5538 | -3.5538 | -3.5536 | -3.5533 | -3.5532 |
| 296 | -3.5541 | -3.5540 | -3.5540 | -3.5540 | -3.5538 | -3.5537 | -3.5537 | -3.5535 | -3.5533 | -3.5531 |
| 322 | -3.5541 | -3.5540 | -3.5540 | -3.5539 | -3.5539 | -3.5539 | -3.5538 | -3.5538 | -3.5538 | -3.5537 |
| 348 | -3.5541 | -3.5541 | -3.5540 | -3.5540 | -3.5540 | -3.5540 | -3.5539 | -3.5539 | -3.5538 | -3.5538 |
| DMRG Energy: -3.5542 | | | | | | | | | | |

**Table S58** NP ansatz with U/t = 2, overlap-based VQE Energies and DMRG Energy for lattice 1x5

| Num Parameters | VQE 1 | VQE 2 | VQE 3 | VQE 4 | VQE 5 | VQE 6 | VQE 7 | VQE 8 | VQE 9 | VQE 10 |
|---|---|---|---|---|---|---|---|---|---|---|
| 44 | -0.9229 | -0.8624 | -0.8624 | -0.8624 | -0.8294 | -0.8294 | -0.8294 | -0.5004 | -0.0554 | -0.0554 |
| 76 | -4.1553 | -4.0976 | -4.0652 | -3.9498 | -3.9287 | -3.9118 | -3.8485 | -3.7063 | -3.6720 | -3.1945 |
| 108 | -4.5221 | -4.5193 | -4.5191 | -4.5108 | -4.4606 | -4.4563 | -4.4546 | -4.4234 | -4.4169 | -4.3648 |
| 140 | -4.5379 | -4.5369 | -4.5343 | -4.5340 | -4.5312 | -4.5286 | -4.5280 | -4.5159 | -4.5153 | -4.4913 |
| 172 | -4.5427 | -4.5416 | -4.5406 | -4.5404 | -4.5403 | -4.5391 | -4.5391 | -4.5388 | -4.5377 | -4.5359 |
| 204 | -4.5447 | -4.5439 | -4.5437 | -4.5427 | -4.5427 | -4.5422 | -4.5409 | -4.5398 | -4.5387 | -4.5382 |
| 236 | -4.5450 | -4.5449 | -4.5446 | -4.5446 | -4.5445 | -4.5443 | -4.5438 | -4.5424 | -4.5411 | -4.5394 |
| 268 | -4.5455 | -4.5452 | -4.5452 | -4.5449 | -4.5448 | -4.5448 | -4.5443 | -4.5442 | -4.5441 | -4.5433 |
| 300 | -4.5458 | -4.5456 | -4.5456 | -4.5455 | -4.5455 | -4.5453 | -4.5452 | -4.5447 | -4.5441 | -4.5422 |
| 332 | -4.5457 | -4.5457 | -4.5457 | -4.5456 | -4.5456 | -4.5456 | -4.5455 | -4.5449 | -4.5446 | -4.5443 |
| 364 | -4.5460 | -4.5459 | -4.5458 | -4.5457 | -4.5457 | -4.5456 | -4.5456 | -4.5456 | -4.5455 | -4.5454 |
| 396 | -4.5460 | -4.5458 | -4.5458 | -4.5458 | -4.5458 | -4.5456 | -4.5456 | -4.5455 | -4.5454 | -4.5446 |
| 428 | -4.5459 | -4.5459 | -4.5458 | -4.5458 | -4.5458 | -4.5458 | -4.5457 | -4.5456 | -4.5456 | -4.5455 |
| DMRG Energy: -4.5463 | | | | | | | | | | |

**Table S59** NP ansatz with U/t = 2, overlap-based VQE Energies and DMRG Energy for lattice 1x6

| Num Parameters | VQE 1 | VQE 2 | VQE 3 | VQE 4 | VQE 5 | VQE 6 | VQE 7 | VQE 8 | VQE 9 | VQE 10 |
|---|---|---|---|---|---|---|---|---|---|---|
| 52 | -1.5384 | -1.5241 | -1.5241 | -1.5241 | -1.5241 | -1.5241 | -1.5241 | -1.5241 | -1.4992 | -1.4992 |
| 90 | -4.8446 | -4.7668 | -4.7514 | -4.7278 | -4.6759 | -4.6443 | -4.6025 | -4.4907 | -4.4083 | -4.4083 |
| 128 | -5.1300 | -5.1203 | -5.1134 | -5.1058 | -5.1040 | -5.0961 | -5.0903 | -5.0818 | -5.0739 | -5.0199 |
| 166 | -5.2307 | -5.2291 | -5.2142 | -5.2095 | -5.2086 | -5.2015 | -5.2015 | -5.1804 | -5.1691 | -5.1336 |
| 204 | -5.2468 | -5.2453 | -5.2451 | -5.2451 | -5.2446 | -5.2434 | -5.2375 | -5.2364 | -5.2346 | -5.1502 |
| 242 | -5.2600 | -5.2578 | -5.2578 | -5.2577 | -5.2576 | -5.2571 | -5.2558 | -5.2539 | -5.2531 | -5.2414 |
| 280 | -5.2620 | -5.2614 | -5.2610 | -5.2606 | -5.2602 | -5.2600 | -5.2599 | -5.2598 | -5.2594 | -5.2580 |
| 318 | -5.2636 | -5.2634 | -5.2632 | -5.2632 | -5.2632 | -5.2628 | -5.2606 | -5.2604 | -5.2584 | -5.2562 |
| 356 | -5.2645 | -5.2642 | -5.2641 | -5.2641 | -5.2639 | -5.2639 | -5.2638 | -5.2625 | -5.2618 | -5.2616 |
| 394 | -5.2658 | -5.2657 | -5.2650 | -5.2648 | -5.2647 | -5.2647 | -5.2644 | -5.2640 | -5.2637 | -5.2632 |
| 432 | -5.2658 | -5.2656 | -5.2653 | -5.2652 | -5.2651 | -5.2650 | -5.2650 | -5.2648 | -5.2648 | -5.2644 |
| 470 | -5.2660 | -5.2658 | -5.2658 | -5.2657 | -5.2657 | -5.2653 | -5.2653 | -5.2653 | -5.2650 | -5.2645 |
| 508 | -5.2661 | -5.2661 | -5.2661 | -5.2660 | -5.2660 | -5.2659 | -5.2658 | -5.2658 | -5.2657 | -5.2652 |
| DMRG Energy: -5.2671 | | | | | | | | | | |

**Table S60** NP ansatz with U/t = 2, overlap-based VQE Energies and DMRG Energy for lattice 1x7

| Num Parameters | VQE 1 | VQE 2 | VQE 3 | VQE 4 | VQE 5 | VQE 6 | VQE 7 | VQE 8 | VQE 9 | VQE 10 |
|---|---|---|---|---|---|---|---|---|---|---|
| 60 | -1.5300 | -1.5300 | -1.5300 | -1.4912 | -1.4912 | -1.4912 | -1.1817 | -0.4740 | -0.4740 | -0.4740 |
| 104 | -5.5916 | -5.3855 | -5.3605 | -5.1108 | -4.9136 | -4.8208 | -4.7627 | -4.7518 | -4.5919 | -4.5454 |
| 148 | -6.0715 | -6.0197 | -5.9819 | -5.9626 | -5.9386 | -5.9238 | -5.9179 | -5.9139 | -5.8736 | -5.8258 |
| 192 | -6.1975 | -6.1927 | -6.1919 | -6.1882 | -6.1844 | -6.1777 | -6.1662 | -6.1360 | -6.1204 | -6.0734 |
| 236 | -6.2145 | -6.2052 | -6.2038 | -6.2036 | -6.2022 | -6.2013 | -6.2008 | -6.1963 | -6.1907 | -6.1859 |
| 280 | -6.2204 | -6.2151 | -6.2130 | -6.2127 | -6.2125 | -6.2105 | -6.2105 | -6.2103 | -6.2088 | -6.2044 |
| 324 | -6.2215 | -6.2193 | -6.2189 | -6.2180 | -6.2159 | -6.2159 | -6.2154 | -6.2142 | -6.2134 | -6.2127 |
| 368 | -6.2237 | -6.2214 | -6.2214 | -6.2201 | -6.2190 | -6.2188 | -6.2184 | -6.2181 | -6.2173 | -6.2169 |
| 412 | -6.2224 | -6.2222 | -6.2212 | -6.2210 | -6.2207 | -6.2206 | -6.2200 | -6.2187 | -6.2186 | -6.2180 |
| 456 | -6.2234 | -6.2232 | -6.2230 | -6.2229 | -6.2229 | -6.2224 | -6.2220 | -6.2208 | -6.2207 | -6.2194 |
| 500 | -6.2236 | -6.2234 | -6.2233 | -6.2233 | -6.2229 | -6.2229 | -6.2219 | -6.2209 | -6.2198 | -6.2192 |
| 544 | -6.2241 | -6.2241 | -6.2236 | -6.2235 | -6.2226 | -6.2218 | -6.2212 | -6.2209 | -6.2208 | -6.2201 |
| 588 | -6.2244 | -6.2243 | -6.2240 | -6.2234 | -6.2234 | -6.2233 | -6.2232 | -6.2228 | -6.2227 | -6.2218 |
| DMRG Energy: -6.2256 | | | | | | | | | | |

**Table S61** NP ansatz with U/t = 2, overlap-based VQE Energies and DMRG Energy for lattice 1x8

| Num Parameters | VQE 1 | VQE 2 | VQE 3 | VQE 4 | VQE 5 | VQE 6 | VQE 7 | VQE 8 | VQE 9 | VQE 10 |
|---|---|---|---|---|---|---|---|---|---|---|
| 68 | -2.1514 | -2.1504 | -2.1102 | -2.0850 | -2.0820 | -2.0820 | -2.0587 | -2.0291 | -2.0291 | -2.0216 |
| 118 | -6.2981 | -6.2604 | -6.1831 | -6.1642 | -6.1299 | -6.1141 | -6.0735 | -6.0441 | -5.9717 | -5.9003 |
| 168 | -6.7123 | -6.6412 | -6.6217 | -6.6157 | -6.6133 | -6.6106 | -6.5864 | -6.5708 | -6.5649 | -6.5239 |
| 218 | -6.8755 | -6.8613 | -6.8204 | -6.8128 | -6.8052 | -6.7917 | -6.7901 | -6.7895 | -6.7857 | -6.7560 |
| 268 | -6.9338 | -6.9245 | -6.9232 | -6.9219 | -6.9152 | -6.9095 | -6.8930 | -6.8919 | -6.8895 | -6.8860 |
| 318 | -6.9446 | -6.9441 | -6.9423 | -6.9415 | -6.9404 | -6.9333 | -6.9298 | -6.9179 | -6.9177 | -6.9029 |
| 368 | -6.9575 | -6.9554 | -6.9544 | -6.9501 | -6.9485 | -6.9467 | -6.9464 | -6.9460 | -6.9434 | -6.9432 |
| 418 | -6.9616 | -6.9605 | -6.9601 | -6.9595 | -6.9587 | -6.9585 | -6.9575 | -6.9566 | -6.9554 | -6.9548 |
| 468 | -6.9650 | -6.9639 | -6.9635 | -6.9631 | -6.9629 | -6.9626 | -6.9623 | -6.9622 | -6.9594 | -6.9584 |
| 518 | -6.9681 | -6.9670 | -6.9663 | -6.9659 | -6.9656 | -6.9647 | -6.9641 | -6.9636 | -6.9635 | -6.9635 |
| 568 | -6.9685 | -6.9677 | -6.9675 | -6.9673 | -6.9672 | -6.9671 | -6.9668 | -6.9667 | -6.9665 | -6.9662 |
| 618 | -6.9684 | -6.9682 | -6.9682 | -6.9682 | -6.9680 | -6.9679 | -6.9674 | -6.9666 | -6.9666 | -6.9656 |
| 668 | -6.9691 | -6.9688 | -6.9684 | -6.9683 | -6.9681 | -6.9678 | -6.9676 | -6.9671 | -6.9669 | -6.9653 |
| DMRG Energy: -6.9712 | | | | | | | | | | |

**Table S62** NP ansatz with U/t = 2, overlap-based VQE Energies and DMRG Energy for lattice 1x9

| Num Parameters | VQE 1 | VQE 2 | VQE 3 | VQE 4 | VQE 5 | VQE 6 | VQE 7 | VQE 8 | VQE 9 | VQE 10 |
|---|---|---|---|---|---|---|---|---|---|---|
| 76 | -1.8881 | -1.8881 | -1.8276 | -1.8276 | -1.7926 | -1.7926 | -1.7426 | -1.6697 | -1.6504 | -1.5597 |
| 132 | -6.3150 | -6.1771 | -6.0420 | -6.0346 | -5.9987 | -5.7210 | -5.6478 | -5.6445 | -5.4996 | -5.4905 |
| 188 | -7.5081 | -7.4798 | -7.4775 | -7.4743 | -7.4724 | -7.4656 | -7.4588 | -7.4211 | -7.4129 | -7.3946 |
| 244 | -7.8522 | -7.8413 | -7.8376 | -7.7915 | -7.7798 | -7.7745 | -7.7735 | -7.7018 | -7.7005 | -7.6832 |
| 300 | -7.8711 | -7.8682 | -7.8645 | -7.8638 | -7.8610 | -7.8577 | -7.8506 | -7.8501 | -7.8314 | -7.8046 |
| 356 | -7.8868 | -7.8848 | -7.8843 | -7.8831 | -7.8820 | -7.8754 | -7.8737 | -7.8702 | -7.8631 | -7.8209 |
| 412 | -7.8957 | -7.8925 | -7.8898 | -7.8888 | -7.8877 | -7.8877 | -7.8876 | -7.8832 | -7.8738 | -7.8685 |
| 468 | -7.8998 | -7.8952 | -7.8946 | -7.8945 | -7.8926 | -7.8922 | -7.8892 | -7.8889 | -7.8875 | -7.8705 |
| 524 | -7.9018 | -7.9007 | -7.8999 | -7.8998 | -7.8996 | -7.8987 | -7.8982 | -7.8952 | -7.8950 | -7.8885 |
| 580 | -7.9038 | -7.9036 | -7.9031 | -7.9029 | -7.9009 | -7.9003 | -7.8993 | -7.8989 | -7.8965 | -7.8962 |
| 636 | -7.9043 | -7.9043 | -7.9040 | -7.9031 | -7.9028 | -7.9027 | -7.9016 | -7.9002 | -7.8996 | -7.8988 |
| 692 | -7.9055 | -7.9052 | -7.9050 | -7.9047 | -7.9045 | -7.9039 | -7.9039 | -7.9030 | -7.8984 | -7.8969 |
| 748 | -7.9057 | -7.9056 | -7.9050 | -7.9047 | -7.9046 | -7.9040 | -7.9037 | -7.9036 | -7.9024 | -7.9019 |
| DMRG Energy: -7.9087 | | | | | | | | | | |

**Table S63** NP ansatz with U/t = 2, overlap-based VQE Energies and DMRG Energy for lattice 1x10

| Num Parameters | VQE 1 | VQE 2 | VQE 3 | VQE 4 | VQE 5 | VQE 6 | VQE 7 | VQE 8 | VQE 9 | VQE 10 |
|---|---|---|---|---|---|---|---|---|---|---|
| 84 | -2.7322 | -2.7257 | -2.7231 | -2.7073 | -2.6886 | -2.6672 | -2.6021 | -2.5723 | -2.5705 | -2.5184 |
| 146 | -7.7516 | -7.5473 | -7.5397 | -7.5013 | -7.4980 | -7.4654 | -7.4607 | -7.4416 | -7.3261 | -6.9084 |
| 208 | -8.3020 | -8.2932 | -8.2904 | -8.1967 | -8.1879 | -8.0832 | -8.0808 | -8.0726 | -8.0501 | -7.9162 |
| 270 | -8.5003 | -8.4772 | -8.4609 | -8.4493 | -8.4031 | -8.3507 | -8.3425 | -8.3407 | -8.2497 | -8.2354 |
| 332 | -8.5799 | -8.5790 | -8.5782 | -8.5551 | -8.5458 | -8.5244 | -8.5219 | -8.5213 | -8.5050 | -8.4894 |
| 394 | -8.6318 | -8.6248 | -8.6235 | -8.6178 | -8.6089 | -8.6035 | -8.5875 | -8.5800 | -8.5648 | -8.5633 |
| 456 | -8.6433 | -8.6390 | -8.6387 | -8.6363 | -8.6359 | -8.6353 | -8.6326 | -8.6229 | -8.6169 | -8.5604 |
| 518 | -8.6534 | -8.6511 | -8.6508 | -8.6502 | -8.6496 | -8.6485 | -8.6451 | -8.6441 | -8.6416 | -8.6411 |
| 580 | -8.6550 | -8.6549 | -8.6548 | -8.6542 | -8.6536 | -8.6534 | -8.6532 | -8.6524 | -8.6505 | -8.6501 |
| 642 | -8.6604 | -8.6576 | -8.6576 | -8.6563 | -8.6548 | -8.6547 | -8.6545 | -8.6519 | -8.6515 | -8.6458 |
| 704 | -8.6617 | -8.6600 | -8.6598 | -8.6567 | -8.6566 | -8.6563 | -8.6561 | -8.6549 | -8.6529 | -8.6516 |
| 766 | -8.6613 | -8.6604 | -8.6602 | -8.6597 | -8.6575 | -8.6564 | -8.6555 | -8.6543 | -8.6539 | -8.6536 |
| 828 | -8.6616 | -8.6587 | -8.6575 | -8.6573 | -8.6550 | -8.6541 | -8.6529 | -8.6513 | -8.6479 | -8.6462 |
| DMRG Energy: -8.6706 | | | | | | | | | | |

**Table S64** NP ansatz with U/t = 2, overlap-based VQE Energies and DMRG Energy for lattice 1x11

| Num Parameters | VQE 1 | VQE 2 | VQE 3 | VQE 4 | VQE 5 | VQE 6 | VQE 7 | VQE 8 | VQE 9 | VQE 10 |
|---|---|---|---|---|---|---|---|---|---|---|
| 92 | -2.5723 | -2.5285 | -2.5260 | -2.5260 | -2.4197 | -2.4134 | -2.4134 | -2.3505 | -2.3036 | -2.2209 |
| 160 | -7.4711 | -7.2230 | -7.1939 | -7.0745 | -6.9640 | -6.8966 | -6.8122 | -6.7444 | -6.7444 | -6.7414 |
| 228 | -9.0844 | -8.9650 | -8.9557 | -8.8964 | -8.8940 | -8.8842 | -8.8839 | -8.8338 | -8.8290 | -8.7595 |
| 296 | -9.4391 | -9.3429 | -9.2899 | -9.2859 | -9.2847 | -9.2806 | -9.2318 | -9.2171 | -9.1870 | -9.1743 |
| 364 | -9.5214 | -9.5192 | -9.4717 | -9.4269 | -9.3726 | -9.3692 | -9.3634 | -9.3614 | -9.3572 | -9.3318 |
| 432 | -9.5306 | -9.5222 | -9.4924 | -9.4200 | -9.4019 | -9.3977 | -9.3641 | -9.3596 | -9.2999 | -9.2331 |
| 500 | -9.4813 | -9.3767 | -9.3379 | -9.3067 | -9.2926 | -9.2849 | -9.2731 | -9.2582 | -9.2221 | -9.1639 |
| 568 | -9.3121 | -9.2818 | -9.2385 | -9.2285 | -9.2154 | -9.2088 | -9.1836 | -9.1680 | -9.0474 | -8.9542 |
| 636 | -9.1814 | -9.1666 | -9.1630 | -9.1029 | -9.0286 | -9.0032 | -8.9774 | -8.9738 | -8.9214 | -8.0865 |
| 704 | -9.0280 | -9.0131 | -8.9460 | -8.8084 | -8.6690 | -8.6025 | -8.5967 | -8.5933 | -6.4069 | 1.9164 |
| 772 | -8.6952 | -8.4070 | -8.0763 | -7.9139 | -7.8056 | -7.7780 | -7.7568 | -7.5473 | -7.4678 | 2.0111 |
| 840 | -9.5769 | -9.5731 | -9.5710 | -9.5692 | -9.5686 | -9.5610 | -9.5558 | -9.5536 | -9.5439 | -9.5431 |
| 908 | -9.5768 | -9.5757 | -9.5708 | -9.5697 | -9.5560 | -9.5524 | -9.5522 | -9.5377 | -9.5243 | |
| DMRG Energy: -9.5938 | | | | | | | | | | |

**Table S65** NP ansatz with U/t = 2, overlap-based VQE Energies and DMRG Energy for lattice 1x12

| Num Parameters | VQE 1 | VQE 2 | VQE 3 | VQE 4 | VQE 5 | VQE 6 | VQE 7 | VQE 8 | VQE 9 | VQE 10 |
|---|---|---|---|---|---|---|---|---|---|---|
| 32 | -2.0000 | -2.0000 | -2.0000 | -1.4920 | -1.1613 | -1.1612 | -1.1612 | 0.0000 | 0.0000 | 0.0000 |
| 56 | -2.6164 | -2.6164 | -2.5782 | -2.4865 | -2.4812 | -2.4393 | -2.4381 | -2.2795 | -2.2321 | -2.2218 |
| 80 | -2.8284 | -2.8245 | -2.8207 | -2.8197 | -2.8148 | -2.7920 | -2.7901 | -2.7852 | -2.7817 | -2.7685 |
| 104 | -2.8284 | -2.8284 | -2.8284 | -2.8284 | -2.8283 | -2.8278 | -2.8265 | -2.8260 | -2.8054 | -2.8037 |
| 128 | -2.8284 | -2.8284 | -2.8283 | -2.8283 | -2.8268 | -2.8261 | -2.8247 | -2.8243 | -2.8235 | -2.8217 |
| 152 | -2.8284 | -2.8284 | -2.8283 | -2.8282 | -2.8281 | -2.8281 | -2.8280 | -2.8278 | -2.8278 | -2.8273 |
| 176 | -2.8284 | -2.8284 | -2.8284 | -2.8284 | -2.8284 | -2.8284 | -2.8284 | -2.8284 | -2.8284 | -2.8284 |
| 200 | -2.8284 | -2.8284 | -2.8284 | -2.8284 | -2.8284 | -2.8284 | -2.8284 | -2.8284 | -2.8284 | -2.8284 |
| 224 | -2.8284 | -2.8284 | -2.8284 | -2.8284 | -2.8284 | -2.8284 | -2.8284 | -2.8284 | -2.8284 | -2.8284 |
| 248 | -2.8284 | -2.8284 | -2.8284 | -2.8284 | -2.8284 | -2.8284 | -2.8284 | -2.8284 | -2.8284 | -2.8284 |
| 272 | -2.8284 | -2.8284 | -2.8284 | -2.8284 | -2.8284 | -2.8284 | -2.8284 | -2.8284 | -2.8284 | -2.8284 |
| 296 | -2.8284 | -2.8284 | -2.8284 | -2.8284 | -2.8284 | -2.8284 | -2.8284 | -2.8284 | -2.8284 | -2.8284 |
| 320 | -2.8284 | -2.8284 | -2.8284 | -2.8284 | -2.8284 | -2.8284 | -2.8284 | -2.8284 | -2.8284 | -2.8284 |
| DMRG Energy: -2.8284 | | | | | | | | | | |

**Table S66** NP ansatz with U/t = 2, overlap-based VQE Energies and DMRG Energy for lattice 2x2

| Num Parameters | VQE 1 | VQE 2 | VQE 3 | VQE 4 | VQE 5 | VQE 6 | VQE 7 | VQE 8 | VQE 9 | VQE 10 |
|---|---|---|---|---|---|---|---|---|---|---|
| 52 | -1.7153 | -1.7153 | -1.7153 | -1.7063 | -1.7063 | -1.7063 | -1.7063 | -1.7063 | -1.7063 | -1.7063 |
| 92 | -4.8186 | -4.7303 | -4.7099 | -4.7051 | -4.6852 | -4.6258 | -4.5046 | -4.4837 | -4.2608 | -4.1810 |
| 132 | -5.0119 | -4.9932 | -4.9668 | -4.9657 | -4.9330 | -4.9264 | -4.9213 | -4.9068 | -4.8258 | -4.7835 |
| 172 | -5.1355 | -5.1026 | -5.0939 | -5.0861 | -5.0750 | -5.0506 | -5.0386 | -5.0255 | -5.0008 | -4.9647 |
| 212 | -5.1440 | -5.1412 | -5.1356 | -5.1345 | -5.1294 | -5.1285 | -5.1047 | -5.1039 | -5.0945 | -5.0879 |
| 252 | -5.1471 | -5.1468 | -5.1461 | -5.1460 | -5.1441 | -5.1387 | -5.1374 | -5.1197 | -5.1077 | -5.0816 |
| 292 | -5.1534 | -5.1533 | -5.1469 | -5.1445 | -5.1419 | -5.1400 | -5.1395 | -5.1372 | -5.1318 | -5.1308 |
| 332 | -5.1560 | -5.1552 | -5.1540 | -5.1496 | -5.1480 | -5.1472 | -5.1452 | -5.1442 | -5.1371 | -5.1367 |
| 372 | -5.1550 | -5.1531 | -5.1520 | -5.1506 | -5.1489 | -5.1476 | -5.1464 | -5.1329 | -5.1309 | -5.1158 |
| 412 | -5.1573 | -5.1558 | -5.1558 | -5.1553 | -5.1550 | -5.1550 | -5.1536 | -5.1521 | -5.1454 | -5.1399 |
| 452 | -5.1571 | -5.1567 | -5.1563 | -5.1562 | -5.1546 | -5.1538 | -5.1534 | -5.1491 | -5.1455 | -5.1444 |
| 492 | -5.1575 | -5.1571 | -5.1568 | -5.1558 | -5.1542 | -5.1530 | -5.1527 | -5.1522 | -5.1519 | -5.1453 |
| 532 | -5.1578 | -5.1576 | -5.1569 | -5.1566 | -5.1563 | -5.1548 | -5.1522 | -5.1520 | -5.1509 | -5.1498 |
| DMRG Energy: -5.1592 | | | | | | | | | | |

**Table S67** NP ansatz with U/t = 2, overlap-based VQE Energies and DMRG Energy for lattice 2x3

| Num Parameters | VQE 1 | VQE 2 | VQE 3 | VQE 4 | VQE 5 | VQE 6 | VQE 7 | VQE 8 | VQE 9 | VQE 10 |
|---|---|---|---|---|---|---|---|---|---|---|
| 84 | -3.8118 | -3.6857 | -3.6857 | -3.6857 | -3.6857 | -3.6857 | -3.6857 | -3.6857 | -3.6857 | -3.6857 |
| 150 | -6.6861 | -6.6062 | -6.6059 | -6.5948 | -6.5869 | -6.5837 | -6.5786 | -6.5713 | -6.5578 | -6.5559 |
| 216 | -7.6228 | -7.5907 | -7.5217 | -7.4468 | -7.3249 | -7.2508 | -7.1237 | -6.9547 | -6.9133 | -6.8879 |
| 282 | -7.7467 | -7.7212 | -7.6837 | -7.6223 | -7.4391 | -7.2891 | -7.2534 | -7.2275 | -7.2228 | -7.1943 |
| 348 | -7.8572 | -7.8366 | -7.8272 | -7.8265 | -7.8144 | -7.7174 | -7.5466 | -7.4985 | -7.4834 | -7.4137 |
| 414 | -7.9175 | -7.9018 | -7.9015 | -7.8880 | -7.8875 | -7.8284 | -7.7688 | -7.6869 | -7.5921 | -7.5913 |
| 480 | -7.9312 | -7.9236 | -7.9219 | -7.9167 | -7.9150 | -7.8651 | -7.8635 | -7.8523 | -7.8294 | -7.6861 |
| 546 | -7.9471 | -7.9440 | -7.9324 | -7.9224 | -7.9215 | -7.9185 | -7.9179 | -7.9161 | -7.8758 | -7.5223 |
| 612 | -7.9486 | -7.9444 | -7.9372 | -7.9353 | -7.9242 | -7.9195 | -7.9118 | -7.8918 | -7.8136 | -7.8093 |
| 678 | -7.9625 | -7.9555 | -7.9528 | -7.9495 | -7.9485 | -7.9396 | -7.9300 | -7.9289 | -7.9127 | -7.8992 |
| 744 | -7.9674 | -7.9604 | -7.9587 | -7.9573 | -7.9562 | -7.9489 | -7.9446 | -7.9058 | -7.8934 | -7.7966 |
| 810 | -7.9690 | -7.9680 | -7.9663 | -7.9659 | -7.9602 | -7.9460 | -7.9339 | -7.9309 | -7.8673 | -7.8415 |
| 876 | -7.9740 | -7.9611 | -7.9610 | -7.9608 | -7.9602 | -7.9590 | -7.8931 | -7.8891 | -7.8818 | -7.8731 |
| DMRG Energy: -7.9865 | | | | | | | | | | |

**Table S68** NP ansatz with U/t = 2, overlap-based VQE Energies and DMRG Energy for lattice 3x3

## S9 NP ansatz, $U/t = 8$, overlap-based optimization

| Num Parameters | VQE 1 | VQE 2 | VQE 3 | VQE 4 | VQE 5 | VQE 6 | VQE 7 | VQE 8 | VQE 9 | VQE 10 |
|---|---|---|---|---|---|---|---|---|---|---|
| 12 | 0.0003 | 0.0246 | 0.0425 | 0.0532 | 0.1030 | 0.3448 | 0.6602 | 0.7771 | 1.4066 | 1.7657 |
| 20 | -0.4721 | -0.4721 | -0.4721 | -0.4721 | -0.4721 | -0.4721 | -0.4721 | -0.4721 | -0.4721 | -0.4721 |
| 28 | -0.4721 | -0.4721 | -0.4721 | -0.4721 | -0.4721 | -0.4721 | -0.4721 | -0.4721 | -0.4721 | -0.4721 |
| 36 | -0.4721 | -0.4721 | -0.4721 | -0.4721 | -0.4721 | -0.4721 | -0.4721 | -0.4721 | -0.4721 | -0.4721 |
| 44 | -0.4721 | -0.4721 | -0.4721 | -0.4721 | -0.4721 | -0.4721 | -0.4721 | -0.4721 | -0.4721 | -0.4721 |
| 52 | -0.4721 | -0.4721 | -0.4721 | -0.4721 | -0.4721 | -0.4721 | -0.4721 | -0.4721 | -0.4721 | -0.4721 |
| 60 | -0.4721 | -0.4721 | -0.4721 | -0.4721 | -0.4721 | -0.4721 | -0.4721 | -0.4721 | -0.4721 | -0.4721 |
| 68 | -0.4721 | -0.4721 | -0.4721 | -0.4721 | -0.4721 | -0.4721 | -0.4721 | -0.4721 | -0.4721 | -0.4721 |
| 76 | -0.4721 | -0.4721 | -0.4721 | -0.4721 | -0.4721 | -0.4721 | -0.4721 | -0.4721 | -0.4721 | -0.4721 |
| 84 | -0.4721 | -0.4721 | -0.4721 | -0.4721 | -0.4721 | -0.4721 | -0.4721 | -0.4721 | -0.4721 | -0.4721 |
| 92 | -0.4721 | -0.4721 | -0.4721 | -0.4721 | -0.4721 | -0.4721 | -0.4721 | -0.4721 | -0.4721 | -0.4721 |
| 100 | -0.4721 | -0.4721 | -0.4721 | -0.4721 | -0.4721 | -0.4721 | -0.4721 | -0.4721 | -0.4721 | -0.4721 |
| 108 | -0.4721 | -0.4721 | -0.4721 | -0.4721 | -0.4721 | -0.4721 | -0.4721 | -0.4721 | -0.4721 | -0.4721 |
| DMRG Energy: -0.4721 | | | | | | | | | | |

**Table S69** NP ansatz with U/t = 8, overlap-based VQE Energies and DMRG Energy for lattice 1x2

| Num Parameters | VQE 1 | VQE 2 | VQE 3 | VQE 4 | VQE 5 | VQE 6 | VQE 7 | VQE 8 | VQE 9 | VQE 10 |
|---|---|---|---|---|---|---|---|---|---|---|
| 20 | -0.1003 | -0.1003 | -0.1003 | -0.1003 | -0.1003 | 0.0000 | 0.0000 | 0.0000 | 0.0000 | 0.0000 |
| 34 | -0.6931 | -0.6918 | -0.6876 | -0.6876 | -0.6707 | -0.6462 | -0.2762 | -0.2762 | -0.2762 | -0.2762 |
| 48 | -0.7077 | -0.7077 | -0.7077 | -0.7077 | -0.7077 | -0.7077 | -0.7077 | -0.7077 | -0.7077 | -0.7077 |
| 62 | -0.7077 | -0.7077 | -0.7077 | -0.7077 | -0.7077 | -0.7077 | -0.7077 | -0.7077 | -0.7077 | -0.7077 |
| 76 | -0.7077 | -0.7077 | -0.7077 | -0.7077 | -0.7077 | -0.7077 | -0.7077 | -0.7077 | -0.7077 | -0.7077 |
| 90 | -0.7077 | -0.7077 | -0.7077 | -0.7077 | -0.7077 | -0.7077 | -0.7077 | -0.7077 | -0.7077 | -0.7077 |
| 104 | -0.7077 | -0.7077 | -0.7077 | -0.7077 | -0.7077 | -0.7077 | -0.7077 | -0.7077 | -0.7077 | -0.7077 |
| 118 | -0.7077 | -0.7077 | -0.7077 | -0.7077 | -0.7077 | -0.7077 | -0.7077 | -0.7077 | -0.7077 | -0.7077 |
| 132 | -0.7077 | -0.7077 | -0.7077 | -0.7077 | -0.7077 | -0.7077 | -0.7077 | -0.7077 | -0.7077 | -0.7077 |
| 146 | -0.7077 | -0.7077 | -0.7077 | -0.7077 | -0.7077 | -0.7077 | -0.7077 | -0.7077 | -0.7077 | -0.7077 |
| 160 | -0.7077 | -0.7077 | -0.7077 | -0.7077 | -0.7077 | -0.7077 | -0.7077 | -0.7077 | -0.7077 | -0.7077 |
| 174 | -0.7077 | -0.7077 | -0.7077 | -0.7077 | -0.7077 | -0.7077 | -0.7077 | -0.7077 | -0.7077 | -0.7077 |
| 188 | -0.7077 | -0.7077 | -0.7077 | -0.7077 | -0.7077 | -0.7077 | -0.7077 | -0.7077 | -0.7077 | -0.7077 |
| DMRG Energy: -0.7077 | | | | | | | | | | |

**Table S70** NP ansatz with U/t = 8, overlap-based VQE Energies and DMRG Energy for lattice 1x3

| Num Parameters | VQE 1 | VQE 2 | VQE 3 | VQE 4 | VQE 5 | VQE 6 | VQE 7 | VQE 8 | VQE 9 | VQE 10 |
|---|---|---|---|---|---|---|---|---|---|---|
| 28 | -0.0947 | -0.0947 | -0.0947 | 0.0000 | 0.0000 | 0.0000 | 0.0000 | 0.0000 | 0.0000 | 0.0021 |
| 48 | -1.0072 | -0.9859 | -0.9842 | -0.9365 | -0.9166 | -0.8992 | -0.8988 | -0.7551 | -0.6185 | -0.5378 |
| 68 | -1.1128 | -1.1018 | -1.1006 | -1.0899 | -1.0876 | -1.0678 | -1.0166 | -1.0004 | -0.9987 | -0.9947 |
| 88 | -1.1169 | -1.1168 | -1.1163 | -1.1160 | -1.1159 | -1.1144 | -1.1142 | -1.1114 | -1.1007 | -1.0946 |
| 108 | -1.1171 | -1.1170 | -1.1170 | -1.1170 | -1.1170 | -1.1170 | -1.1170 | -1.1164 | -1.1161 | -1.1154 |
| 128 | -1.1172 | -1.1171 | -1.1171 | -1.1171 | -1.1171 | -1.1170 | -1.1170 | -1.1159 | -1.1129 | -1.1122 |
| 148 | -1.1172 | -1.1172 | -1.1172 | -1.1172 | -1.1172 | -1.1172 | -1.1171 | -1.1171 | -1.1170 | -1.1170 |
| 168 | -1.1172 | -1.1172 | -1.1172 | -1.1172 | -1.1172 | -1.1172 | -1.1172 | -1.1172 | -1.1172 | -1.1172 |
| 188 | -1.1172 | -1.1172 | -1.1172 | -1.1172 | -1.1172 | -1.1172 | -1.1172 | -1.1172 | -1.1172 | -1.1171 |
| 208 | -1.1172 | -1.1172 | -1.1172 | -1.1172 | -1.1172 | -1.1172 | -1.1172 | -1.1172 | -1.1172 | -1.1171 |
| 228 | -1.1172 | -1.1172 | -1.1172 | -1.1172 | -1.1172 | -1.1172 | -1.1171 | -1.1171 | -1.1171 | -1.1171 |
| 248 | -1.1172 | -1.1172 | -1.1172 | -1.1172 | -1.1172 | -1.1172 | -1.1172 | -1.1172 | -1.1172 | -1.1172 |
| 268 | -1.1172 | -1.1172 | -1.1172 | -1.1172 | -1.1172 | -1.1172 | -1.1172 | -1.1172 | -1.1172 | -1.1171 |
| DMRG Energy: -1.1172 | | | | | | | | | | |

**Table S71** NP ansatz with U/t = 8, overlap-based VQE Energies and DMRG Energy for lattice 1x4

| Num Parameters | VQE 1 | VQE 2 | VQE 3 | VQE 4 | VQE 5 | VQE 6 | VQE 7 | VQE 8 | VQE 9 | VQE 10 |
|---|---|---|---|---|---|---|---|---|---|---|
| 36 | -0.1899 | -0.1899 | -0.1899 | -0.1839 | -0.1839 | -0.1839 | -0.0912 | -0.0912 | 0.0000 | 0.0010 |
| 62 | -1.2517 | -1.1517 | -1.1371 | -1.1220 | -1.0929 | -1.0899 | -1.0094 | -0.9825 | -0.9285 | -0.8483 |
| 88 | -1.3140 | -1.3135 | -1.3081 | -1.3047 | -1.3030 | -1.2969 | -1.2837 | -1.2790 | -1.2437 | -1.1149 |
| 114 | -1.3556 | -1.3525 | -1.3512 | -1.3504 | -1.3484 | -1.3412 | -1.3222 | -1.3174 | -1.3081 | -1.3057 |
| 140 | -1.3716 | -1.3650 | -1.3633 | -1.3601 | -1.3579 | -1.3566 | -1.3549 | -1.3522 | -1.3411 | -1.3288 |
| 166 | -1.3753 | -1.3747 | -1.3697 | -1.3673 | -1.3671 | -1.3666 | -1.3655 | -1.3647 | -1.3623 | -1.3566 |
| 192 | -1.3776 | -1.3774 | -1.3773 | -1.3770 | -1.3766 | -1.3738 | -1.3719 | -1.3711 | -1.3709 | -1.3673 |
| 218 | -1.3795 | -1.3783 | -1.3779 | -1.3765 | -1.3762 | -1.3758 | -1.3758 | -1.3747 | -1.3729 | -1.3704 |
| 244 | -1.3799 | -1.3798 | -1.3798 | -1.3796 | -1.3790 | -1.3788 | -1.3787 | -1.3775 | -1.3773 | -1.3768 |
| 270 | -1.3810 | -1.3807 | -1.3807 | -1.3802 | -1.3802 | -1.3801 | -1.3800 | -1.3795 | -1.3794 | -1.3792 |
| 296 | -1.3818 | -1.3818 | -1.3810 | -1.3809 | -1.3806 | -1.3804 | -1.3803 | -1.3800 | -1.3798 | -1.3794 |
| 322 | -1.3817 | -1.3815 | -1.3815 | -1.3814 | -1.3813 | -1.3812 | -1.3810 | -1.3808 | -1.3806 | -1.3805 |
| 348 | -1.3821 | -1.3819 | -1.3818 | -1.3817 | -1.3816 | -1.3815 | -1.3814 | -1.3812 | -1.3811 | -1.3805 |
| DMRG Energy: -1.3826 | | | | | | | | | | |

**Table S72** NP ansatz with U/t = 8, overlap-based VQE Energies and DMRG Energy for lattice 1x5

| Num Parameters | VQE 1 | VQE 2 | VQE 3 | VQE 4 | VQE 5 | VQE 6 | VQE 7 | VQE 8 | VQE 9 | VQE 10 |
|---|---|---|---|---|---|---|---|---|---|---|
| 44 | -0.0768 | -0.0768 | 0.0000 | 0.0000 | 0.1741 | 0.1741 | 0.2197 | 0.2197 | 0.2414 | 0.2414 |
| 76 | -1.4539 | -1.4538 | -1.4339 | -1.3811 | -1.3153 | -1.2780 | -0.9704 | -0.8848 | -0.7278 | -0.6358 |
| 108 | -1.6487 | -1.5518 | -1.4989 | -1.4972 | -1.4730 | -1.4683 | -1.4312 | -1.4178 | -1.4044 | -1.4027 |
| 140 | -1.7352 | -1.7256 | -1.6956 | -1.6915 | -1.6910 | -1.6873 | -1.6840 | -1.6519 | -1.6287 | -1.5301 |
| 172 | -1.7548 | -1.7526 | -1.7487 | -1.7483 | -1.7478 | -1.7457 | -1.7429 | -1.7392 | -1.6866 | -1.6647 |
| 204 | -1.7607 | -1.7604 | -1.7601 | -1.7594 | -1.7589 | -1.7572 | -1.7527 | -1.7492 | -1.7483 | -1.7424 |
| 236 | -1.7625 | -1.7599 | -1.7595 | -1.7593 | -1.7573 | -1.7568 | -1.7566 | -1.7540 | -1.7506 | -1.7441 |
| 268 | -1.7637 | -1.7635 | -1.7621 | -1.7620 | -1.7618 | -1.7618 | -1.7614 | -1.7599 | -1.7583 | -1.7582 |
| 300 | -1.7632 | -1.7618 | -1.7617 | -1.7615 | -1.7615 | -1.7596 | -1.7596 | -1.7595 | -1.7595 | -1.7575 |
| 332 | -1.7651 | -1.7632 | -1.7617 | -1.7608 | -1.7608 | -1.7605 | -1.7602 | -1.7593 | -1.7593 | -1.7574 |
| 364 | -1.7647 | -1.7646 | -1.7641 | -1.7639 | -1.7636 | -1.7627 | -1.7626 | -1.7622 | -1.7617 | -1.7597 |
| 396 | -1.7650 | -1.7644 | -1.7636 | -1.7634 | -1.7631 | -1.7629 | -1.7626 | -1.7623 | -1.7620 | -1.7619 |
| 428 | -1.7656 | -1.7654 | -1.7650 | -1.7649 | -1.7640 | -1.7639 | -1.7631 | -1.7619 | -1.7615 | -1.7603 |
| DMRG Energy: -1.7681 | | | | | | | | | | |

**Table S73** NP ansatz with U/t = 8, overlap-based VQE Energies and DMRG Energy for lattice 1x6

| Num Parameters | VQE 1 | VQE 2 | VQE 3 | VQE 4 | VQE 5 | VQE 6 | VQE 7 | VQE 8 | VQE 9 | VQE 10 |
|---|---|---|---|---|---|---|---|---|---|---|
| 52 | -0.2728 | -0.2728 | -0.2639 | -0.2639 | -0.2639 | -0.2639 | -0.2639 | -0.2601 | -0.2476 | 0.0006 |
| 90 | -1.7314 | -1.6624 | -1.6196 | -1.5584 | -1.5399 | -1.5380 | -1.4447 | -1.4067 | -1.3506 | -1.0972 |
| 128 | -1.8505 | -1.8396 | -1.8260 | -1.8031 | -1.8002 | -1.7715 | -1.7470 | -1.7320 | -1.7311 | -1.6719 |
| 166 | -1.9608 | -1.9497 | -1.9321 | -1.9250 | -1.9188 | -1.9050 | -1.8940 | -1.8759 | -1.8494 | -1.7969 |
| 204 | -2.0013 | -1.9987 | -1.9762 | -1.9757 | -1.9713 | -1.9707 | -1.9658 | -1.9579 | -1.9462 | -1.9428 |
| 242 | -2.0088 | -2.0063 | -2.0010 | -1.9980 | -1.9976 | -1.9876 | -1.9871 | -1.9838 | -1.9803 | -1.9745 |
| 280 | -2.0189 | -2.0131 | -2.0124 | -2.0120 | -2.0102 | -2.0085 | -2.0068 | -2.0058 | -2.0055 | -2.0044 |
| 318 | -2.0253 | -2.0250 | -2.0250 | -2.0221 | -2.0202 | -2.0200 | -2.0156 | -2.0147 | -2.0143 | -2.0138 |
| 356 | -2.0336 | -2.0324 | -2.0278 | -2.0275 | -2.0274 | -2.0260 | -2.0257 | -2.0221 | -2.0195 | -2.0184 |
| 394 | -2.0375 | -2.0350 | -2.0339 | -2.0336 | -2.0327 | -2.0322 | -2.0319 | -2.0307 | -2.0294 | -2.0166 |
| 432 | -2.0404 | -2.0398 | -2.0382 | -2.0381 | -2.0348 | -2.0341 | -2.0330 | -2.0312 | -2.0309 | -2.0283 |
| 470 | -2.0406 | -2.0396 | -2.0391 | -2.0384 | -2.0376 | -2.0343 | -2.0340 | -2.0331 | -2.0319 | -2.0300 |
| 508 | -2.0419 | -2.0417 | -2.0407 | -2.0404 | -2.0391 | -2.0370 | -2.0367 | -2.0367 | -2.0317 | -2.0315 |
| DMRG Energy: -2.0482 | | | | | | | | | | |

**Table S74** NP ansatz with U/t = 8, overlap-based VQE Energies and DMRG Energy for lattice 1x7

| Num Parameters | VQE 1 | VQE 2 | VQE 3 | VQE 4 | VQE 5 | VQE 6 | VQE 7 | VQE 8 | VQE 9 | VQE 10 |
|---|---|---|---|---|---|---|---|---|---|---|
| 60 | -0.0328 | 0.0076 | 0.0076 | 0.0524 | 0.0524 | 0.0524 | 0.1478 | 0.1782 | 0.1782 | 0.1925 |
| 104 | -1.9095 | -1.8943 | -1.7950 | -1.6807 | -1.6721 | -1.4172 | -1.2923 | -1.2253 | -1.2182 | -0.7592 |
| 148 | -2.1237 | -2.0981 | -2.0942 | -2.0619 | -2.0610 | -2.0383 | -2.0019 | -1.9875 | -1.9462 | -1.9339 |
| 192 | -2.3509 | -2.3209 | -2.3083 | -2.2824 | -2.1940 | -2.1900 | -2.1498 | -2.1357 | -2.0955 | -2.0553 |
| 236 | -2.3631 | -2.3563 | -2.3395 | -2.3385 | -2.3226 | -2.3199 | -2.3191 | -2.3094 | -2.2440 | -2.2211 |
| 280 | -2.3976 | -2.3845 | -2.3840 | -2.3803 | -2.3775 | -2.3745 | -2.3666 | -2.3593 | -2.3592 | -2.3354 |
| 324 | -2.3941 | -2.3853 | -2.3831 | -2.3767 | -2.3734 | -2.3696 | -2.3628 | -2.3622 | -2.3558 | -2.3508 |
| 368 | -2.4006 | -2.3979 | -2.3934 | -2.3923 | -2.3911 | -2.3902 | -2.3864 | -2.3744 | -2.3692 | -2.3539 |
| 412 | -2.4052 | -2.4004 | -2.3969 | -2.3918 | -2.3911 | -2.3910 | -2.3878 | -2.3875 | -2.3788 | -2.3599 |
| 456 | -2.4076 | -2.4065 | -2.4045 | -2.4035 | -2.4016 | -2.4007 | -2.3980 | -2.3971 | -2.3968 | -2.3955 |
| 500 | -2.4113 | -2.4105 | -2.4103 | -2.4085 | -2.4054 | -2.4043 | -2.4036 | -2.4025 | -2.3916 | -2.3906 |
| 544 | -2.4110 | -2.4102 | -2.4090 | -2.4073 | -2.4060 | -2.4048 | -2.4047 | -2.4030 | -2.3996 | -2.3996 |
| 588 | -2.4130 | -2.4127 | -2.4123 | -2.4116 | -2.4103 | -2.4084 | -2.4078 | -2.4070 | -2.4034 | -2.4026 |
| DMRG Energy: -2.4208 | | | | | | | | | | |

**Table S75** NP ansatz with U/t = 8, overlap-based VQE Energies and DMRG Energy for lattice 1x8

| Num Parameters | VQE 1 | VQE 2 | VQE 3 | VQE 4 | VQE 5 | VQE 6 | VQE 7 | VQE 8 | VQE 9 | VQE 10 |
|---|---|---|---|---|---|---|---|---|---|---|
| 68 | -0.3490 | -0.3426 | -0.3359 | -0.3304 | -0.3259 | -0.3258 | -0.3244 | -0.2928 | -0.2760 | -0.2760 |
| 118 | -2.1547 | -2.1176 | -2.0587 | -1.9818 | -1.9433 | -1.8724 | -1.8724 | -1.8625 | -1.8485 | -1.7274 |
| 168 | -2.3825 | -2.3657 | -2.2464 | -2.2228 | -2.2111 | -2.2092 | -2.1998 | -2.1847 | -2.1647 | -2.0634 |
| 218 | -2.5358 | -2.5188 | -2.5140 | -2.5015 | -2.4738 | -2.4738 | -2.4442 | -2.4266 | -2.4160 | -2.4066 |
| 268 | -2.5962 | -2.5868 | -2.5682 | -2.5343 | -2.5341 | -2.5291 | -2.5214 | -2.5028 | -2.5008 | -2.4624 |
| 318 | -2.6248 | -2.6206 | -2.5993 | -2.5962 | -2.5954 | -2.5897 | -2.5826 | -2.5795 | -2.5786 | -2.5601 |
| 368 | -2.6261 | -2.6237 | -2.6228 | -2.6214 | -2.6207 | -2.6204 | -2.6200 | -2.6152 | -2.6105 | -2.5874 |
| 418 | -2.6547 | -2.6501 | -2.6494 | -2.6491 | -2.6466 | -2.6462 | -2.6449 | -2.6418 | -2.6351 | -2.6286 |
| 468 | -2.6726 | -2.6639 | -2.6618 | -2.6616 | -2.6588 | -2.6575 | -2.6559 | -2.6545 | -2.6299 | -2.6248 |
| 518 | -2.6806 | -2.6778 | -2.6764 | -2.6752 | -2.6737 | -2.6731 | -2.6714 | -2.6700 | -2.6693 | -2.6550 |
| 568 | -2.6851 | -2.6822 | -2.6814 | -2.6812 | -2.6811 | -2.6804 | -2.6800 | -2.6729 | -2.6700 | -2.6641 |
| 618 | -2.6904 | -2.6882 | -2.6870 | -2.6850 | -2.6830 | -2.6825 | -2.6823 | -2.6819 | -2.6736 | -2.6710 |
| 668 | -2.6954 | -2.6888 | -2.6886 | -2.6886 | -2.6879 | -2.6848 | -2.6842 | -2.6840 | -2.6838 | -2.6759 |
| DMRG Energy: -2.7098 | | | | | | | | | | |

**Table S76** NP ansatz with U/t = 8, overlap-based VQE Energies and DMRG Energy for lattice 1x9

| Num Parameters | VQE 1 | VQE 2 | VQE 3 | VQE 4 | VQE 5 | VQE 6 | VQE 7 | VQE 8 | VQE 9 | VQE 10 |
|---|---|---|---|---|---|---|---|---|---|---|
| 76 | -0.0236 | -0.0236 | -0.0236 | 0.0406 | 0.0412 | 0.0727 | 0.0728 | 0.1242 | 0.1580 | 0.2217 |
| 132 | -2.3275 | -2.2392 | -2.2214 | -2.1851 | -2.0776 | -1.9618 | -1.8035 | -1.7147 | -1.6042 | -1.1435 |
| 188 | -2.7235 | -2.6822 | -2.6126 | -2.5481 | -2.5201 | -2.5119 | -2.5008 | -2.4946 | -2.4852 | -2.4259 |
| 244 | -2.9560 | -2.9357 | -2.9184 | -2.8813 | -2.8576 | -2.8572 | -2.8395 | -2.7911 | -2.6851 | -2.6130 |
| 300 | -2.9643 | -2.9582 | -2.9564 | -2.9546 | -2.9470 | -2.9128 | -2.8863 | -2.8616 | -2.8107 | -2.7825 |
| 356 | -2.9997 | -2.9894 | -2.9613 | -2.9581 | -2.9322 | -2.9299 | -2.9056 | -2.8939 | -2.8842 | -2.8558 |
| 412 | -3.0103 | -2.9967 | -2.9959 | -2.9919 | -2.9879 | -2.9819 | -2.9561 | -2.9514 | -2.8735 | -2.8472 |
| 468 | -3.0269 | -3.0248 | -3.0215 | -3.0215 | -3.0202 | -3.0060 | -2.9966 | -2.9945 | -2.9901 | -2.9278 |
| 524 | -3.0313 | -3.0282 | -3.0276 | -3.0253 | -3.0209 | -3.0146 | -3.0100 | -3.0080 | -2.9769 | -2.9608 |
| 580 | -3.0479 | -3.0435 | -3.0378 | -3.0358 | -3.0355 | -3.0353 | -3.0325 | -3.0322 | -3.0273 | -2.9984 |
| 636 | -3.0482 | -3.0453 | -3.0443 | -3.0398 | -3.0378 | -3.0371 | -3.0351 | -3.0306 | -3.0285 | -3.0113 |
| 692 | -3.0526 | -3.0504 | -3.0502 | -3.0422 | -3.0421 | -3.0413 | -3.0338 | -3.0282 | -3.0219 | -2.9940 |
| 748 | -3.0508 | -3.0469 | -3.0446 | -3.0423 | -3.0419 | -3.0410 | -3.0403 | -3.0374 | -3.0327 | -3.0321 |
| DMRG Energy: -3.0744 | | | | | | | | | | |

**Table S77** NP ansatz with U/t = 8, overlap-based VQE Energies and DMRG Energy for lattice 1x10

| Num Parameters | VQE 1 | VQE 2 | VQE 3 | VQE 4 | VQE 5 | VQE 6 | VQE 7 | VQE 8 | VQE 9 | VQE 10 |
|---|---|---|---|---|---|---|---|---|---|---|
| 84 | -0.4208 | -0.4206 | -0.4206 | -0.4105 | -0.3992 | -0.3848 | -0.3727 | -0.3556 | -0.3523 | -0.3523 |
| 146 | -2.6728 | -2.6516 | -2.6017 | -2.5535 | -2.4755 | -2.4612 | -2.2676 | -2.2278 | -2.2150 | -2.2040 |
| 208 | -2.9649 | -2.8772 | -2.8379 | -2.8003 | -2.7945 | -2.7725 | -2.7491 | -2.7386 | -2.7061 | -2.6565 |
| 270 | -3.1665 | -3.1127 | -3.1031 | -3.0634 | -3.0265 | -3.0251 | -3.0124 | -2.9950 | -2.9740 | -2.9639 |
| 332 | -3.1691 | -3.1593 | -3.1407 | -3.1396 | -3.1246 | -3.1210 | -3.1124 | -3.0918 | -3.0670 | -3.0385 |
| 394 | -3.2323 | -3.2250 | -3.2142 | -3.2139 | -3.2100 | -3.2014 | -3.1926 | -3.1749 | -3.1159 | -3.1157 |
| 456 | -3.2760 | -3.2615 | -3.2561 | -3.2262 | -3.2220 | -3.2114 | -3.2114 | -3.1973 | -3.1855 | -3.1611 |
| 518 | -3.3049 | -3.2845 | -3.2740 | -3.2698 | -3.2687 | -3.2668 | -3.2645 | -3.2548 | -3.2471 | -3.2237 |
| 580 | -3.3191 | -3.3137 | -3.3059 | -3.2985 | -3.2936 | -3.2901 | -3.2761 | -3.2718 | -3.2687 | -3.2511 |
| 642 | -3.3251 | -3.3189 | -3.3185 | -3.3144 | -3.3099 | -3.3070 | -3.2916 | -3.2866 | -3.2816 | -3.2596 |
| 704 | -3.3246 | -3.3173 | -3.3168 | -3.3105 | -3.3028 | -3.3008 | -3.2956 | -3.2916 | -3.2915 | -3.2888 |
| 766 | -3.3276 | -3.3249 | -3.3207 | -3.3183 | -3.3174 | -3.3115 | -3.3110 | -3.3107 | -3.2909 | -3.2906 |
| 828 | -3.3314 | -3.3290 | -3.3251 | -3.3222 | -3.3216 | -3.3196 | -3.2972 | -3.2923 | -3.2905 | -3.2802 |
| DMRG Energy: -3.3693 | | | | | | | | | | |

**Table S78** NP ansatz with U/t = 8, overlap-based VQE Energies and DMRG Energy for lattice 1x11

| Num Parameters | VQE 1 | VQE 2 | VQE 3 | VQE 4 | VQE 5 | VQE 6 | VQE 7 | VQE 8 | VQE 9 | VQE 10 |
|---|---|---|---|---|---|---|---|---|---|---|
| 92 | -0.1207 | -0.1007 | -0.0589 | -0.0300 | 0.0065 | 0.0244 | 0.0590 | 0.0590 | 0.0759 | 0.0759 |
| 160 | -2.9607 | -2.6107 | -2.5805 | -2.5051 | -2.4468 | -2.3853 | -2.3589 | -2.2655 | -2.0377 | -1.7172 |
| 228 | -3.3064 | -3.2773 | -3.1419 | -3.0584 | -3.0409 | -3.0046 | -2.9672 | -2.9562 | -2.9037 | -2.7625 |
| 296 | -3.5413 | -3.4383 | -3.4100 | -3.3694 | -3.3584 | -3.3572 | -3.3080 | -3.2758 | -3.2523 | -3.1826 |
| 364 | -3.5452 | -3.5380 | -3.5307 | -3.5145 | -3.5073 | -3.5059 | -3.4683 | -3.4393 | -3.3884 | -3.2909 |
| 432 | -3.5703 | -3.5561 | -3.5526 | -3.5284 | -3.5263 | -3.5099 | -3.5032 | -3.5023 | -3.4417 | -3.4124 |
| 500 | -3.6063 | -3.6004 | -3.5884 | -3.5832 | -3.5755 | -3.5626 | -3.5588 | -3.5553 | -3.5015 | -3.4922 |
| 568 | -3.6199 | -3.6125 | -3.6049 | -3.5905 | -3.5878 | -3.5843 | -3.5834 | -3.5656 | -3.5490 | -3.3754 |
| 636 | -3.6227 | -3.6176 | -3.6147 | -3.6133 | -3.6106 | -3.5960 | -3.5828 | -3.5800 | -3.5717 | -3.5516 |
| 704 | -3.6033 | -3.5963 | -3.5686 | -3.5671 | -3.5610 | -3.5496 | -3.5240 | -3.4598 | -3.4588 | -3.3976 |
| 772 | -3.5830 | -3.5816 | -3.5685 | -3.5636 | -3.5412 | -3.5154 | -3.5078 | -3.4959 | -3.4669 | -3.4399 |
| 840 | -3.6801 | -3.6341 | -3.6253 | -3.6248 | -3.6156 | -3.6044 | -3.6044 | -3.5911 | -3.5644 | -3.5611 |
| 908 | -3.6382 | -3.6307 | -3.6253 | -3.6205 | -3.6165 | -3.6082 | -3.6048 | -3.5959 | -3.5804 | -3.5758 |
| DMRG Energy: -3.7284 | | | | | | | | | | |

**Table S79** NP ansatz with U/t = 8, overlap-based VQE Energies and DMRG Energy for lattice 1x12

| Num Parameters | VQE 1 | VQE 2 | VQE 3 | VQE 4 | VQE 5 | VQE 6 | VQE 7 | VQE 8 | VQE 9 | VQE 10 |
|---|---|---|---|---|---|---|---|---|---|---|
| 32 | -0.0406 | -0.0406 | 0.0000 | 0.0000 | 0.0000 | 0.0000 | 0.0000 | 0.0681 | 0.0681 | 1.2268 |
| 56 | -1.1732 | -0.7598 | -0.7163 | -0.7123 | -0.5653 | -0.5618 | -0.3699 | -0.3699 | -0.3699 | 0.0490 |
| 80 | -1.3202 | -1.3119 | -1.3097 | -1.3022 | -1.2782 | -1.2592 | -1.1964 | -1.1885 | -1.1772 | -1.0896 |
| 104 | -1.3201 | -1.3186 | -1.3179 | -1.3032 | -1.2908 | -1.2849 | -1.2741 | -1.2375 | -1.2262 | -1.1885 |
| 128 | -1.3202 | -1.3201 | -1.3200 | -1.3167 | -1.3112 | -1.3108 | -1.3105 | -1.3104 | -1.3098 | -1.3081 |
| 152 | -1.3202 | -1.3200 | -1.3199 | -1.3199 | -1.3198 | -1.3195 | -1.3193 | -1.3192 | -1.3191 | -1.3190 |
| 176 | -1.3202 | -1.3202 | -1.3202 | -1.3202 | -1.3202 | -1.3202 | -1.3202 | -1.3202 | -1.3202 | -1.3202 |
| 200 | -1.3202 | -1.3202 | -1.3202 | -1.3202 | -1.3202 | -1.3202 | -1.3202 | -1.3202 | -1.3202 | -1.3202 |
| 224 | -1.3202 | -1.3202 | -1.3202 | -1.3202 | -1.3202 | -1.3202 | -1.3202 | -1.3202 | -1.3202 | -1.3202 |
| 248 | -1.3202 | -1.3202 | -1.3202 | -1.3202 | -1.3202 | -1.3202 | -1.3202 | -1.3202 | -1.3202 | -1.3202 |
| 272 | -1.3202 | -1.3202 | -1.3202 | -1.3202 | -1.3202 | -1.3202 | -1.3202 | -1.3202 | -1.3202 | -1.3202 |
| 296 | -1.3202 | -1.3202 | -1.3202 | -1.3202 | -1.3202 | -1.3202 | -1.3202 | -1.3202 | -1.3202 | -1.3202 |
| 320 | -1.3202 | -1.3202 | -1.3202 | -1.3202 | -1.3202 | -1.3202 | -1.3202 | -1.3202 | -1.3202 | -1.3202 |
| DMRG Energy: -1.3202 | | | | | | | | | | |

**Table S80** NP ansatz with U/t = 8, overlap-based VQE Energies and DMRG Energy for lattice 2x2

| Num Parameters | VQE 1 | VQE 2 | VQE 3 | VQE 4 | VQE 5 | VQE 6 | VQE 7 | VQE 8 | VQE 9 | VQE 10 |
|---|---|---|---|---|---|---|---|---|---|---|
| 52 | -0.4781 | -0.4442 | -0.4442 | -0.4442 | -0.4442 | -0.4442 | -0.4395 | -0.4390 | -0.1553 | -0.0928 |
| 92 | -1.1219 | -0.9950 | -0.9798 | -0.9661 | -0.4277 | -0.3965 | -0.3421 | -0.3046 | 0.1542 | 1.3157 |
| 132 | -1.7717 | -1.6135 | -1.5190 | -1.4972 | -1.4864 | -1.4791 | -1.4048 | -1.3954 | -1.2907 | -1.1405 |
| 172 | -2.0243 | -1.9753 | -1.9692 | -1.9314 | -1.8375 | -1.8365 | -1.8247 | -1.8052 | -1.6234 | -1.5987 |
| 212 | -2.0627 | -2.0567 | -2.0548 | -2.0381 | -2.0048 | -2.0009 | -1.9689 | -1.9654 | -1.9485 | -1.9468 |
| 252 | -2.0798 | -2.0741 | -2.0712 | -2.0596 | -2.0509 | -2.0495 | -1.9967 | -1.9896 | -1.9531 | -1.8834 |
| 292 | -2.1243 | -2.1141 | -2.1130 | -2.0990 | -2.0944 | -2.0902 | -2.0836 | -2.0833 | -2.0722 | -2.0171 |
| 332 | -2.1605 | -2.1469 | -2.1326 | -2.1246 | -2.1224 | -2.1184 | -2.1159 | -2.0957 | -2.0881 | -2.0635 |
| 372 | -2.1662 | -2.1609 | -2.1577 | -2.1480 | -2.1292 | -2.1226 | -2.1156 | -2.1117 | -2.1034 | -2.0893 |
| 412 | -2.1648 | -2.1546 | -2.1511 | -2.1499 | -2.1483 | -2.1412 | -2.1376 | -2.1259 | -2.1218 | -2.1015 |
| 452 | -2.1694 | -2.1632 | -2.1565 | -2.1559 | -2.1525 | -2.1519 | -2.1472 | -2.1367 | -2.1212 | -2.1150 |
| 492 | -2.1622 | -2.1608 | -2.1563 | -2.1506 | -2.1399 | -2.1360 | -2.1338 | -2.1299 | -2.1267 | -2.1221 |
| 532 | -2.1549 | -2.1539 | -2.1497 | -2.1461 | -2.1452 | -2.1399 | -2.1348 | -2.1300 | -2.1291 | -2.1010 |
| DMRG Energy: -2.1778 | | | | | | | | | | |

**Table S81** NP ansatz with U/t = 8, overlap-based VQE Energies and DMRG Energy for lattice 2x3

| Num Parameters | VQE 1 | VQE 2 | VQE 3 | VQE 4 | VQE 5 | VQE 6 | VQE 7 | VQE 8 | VQE 9 | VQE 10 |
|---|---|---|---|---|---|---|---|---|---|---|
| 84 | -1.2376 | -1.2319 | -1.2319 | -1.2319 | -1.2318 | -1.2318 | -1.2318 | -1.2310 | -1.2310 | -1.2309 |
| 150 | -2.6646 | -2.4076 | -2.3457 | -2.3273 | -2.2664 | -2.2553 | -2.2456 | -1.8513 | -1.7772 | -1.7704 |
| 216 | -3.1253 | -3.0934 | -3.0910 | -3.0644 | -3.0315 | -3.0170 | -3.0168 | -2.9960 | -2.9295 | -2.9208 |
| 282 | -3.1698 | -3.1312 | -3.1259 | -3.1246 | -3.1035 | -3.0778 | -3.0629 | -3.0388 | -3.0302 | -2.8958 |
| 348 | -3.1596 | -3.1565 | -3.1362 | -3.1210 | -3.1143 | -3.1130 | -3.0865 | -3.0838 | -3.0796 | -3.0431 |
| 414 | -3.2037 | -3.1864 | -3.1849 | -3.1838 | -3.1610 | -3.1571 | -3.1508 | -3.1367 | -3.1339 | -3.1104 |
| 480 | -3.2614 | -3.2511 | -3.2502 | -3.2280 | -3.2192 | -3.2183 | -3.2175 | -3.1894 | -3.1827 | -3.1657 |
| 546 | -3.2931 | -3.2695 | -3.2493 | -3.2489 | -3.2456 | -3.2378 | -3.2217 | -3.2092 | -3.1996 | -3.1356 |
| 612 | -3.3185 | -3.3076 | -3.2908 | -3.2648 | -3.2646 | -3.2629 | -3.2480 | -3.2423 | -3.2360 | -3.2343 |
| 678 | -3.3242 | -3.3163 | -3.3071 | -3.2963 | -3.2835 | -3.2695 | -3.2586 | -3.2498 | -3.1886 | 15.0438 |
| 744 | -3.3482 | -3.3339 | -3.3190 | -3.3125 | -3.3101 | -3.3082 | -3.3026 | -3.2873 | -3.2675 | -3.2165 |
| 810 | -3.3315 | -3.3206 | -3.3174 | -3.3119 | -3.3111 | -3.3071 | -3.3000 | -3.2975 | -3.2784 | -3.2769 |
| 876 | -3.3721 | -3.3364 | -3.3227 | -3.3186 | -3.3128 | -3.2981 | -3.2825 | -3.2371 | -3.2304 | -3.2213 |
| DMRG Energy: -3.4911 | | | | | | | | | | |

**Table S82** NP ansatz with U/t = 8, overlap-based VQE Energies and DMRG Energy for lattice 3x3

# S10 NP ansatz, $U/t = 2$, $4 \times 4$ lattice

| Num Parameters | VQE 1 | VQE 2 | VQE 3 | VQE 4 | VQE 5 | VQE 6 | VQE 7 | VQE 8 |
|---|---|---|---|---|---|---|---|---|
| 1568 | -15.1312 | -15.119887 | -15.020804 | -14.85806363 | -14.512017 | -14.48226568 | -14.461322 | -9.3937255 |
| DMRG Energy: -15.4634 | | | | | | | | |

**Table S83** NP ansatz with U/t = 2, VQE Energies and DMRG Energy for lattice 4x4
